# Supplementary material for: QInfer: Statistical inference software for quantum applications
Source: arXiv:1610.00336 ancillary file (2017-04-13)
Supplement: Supplementary file 1 [file User_Guide.pdf]

---

# QInfer: Bayesian Inference for Quantum Information

Christopher Granade and Christopher Ferrie

Sep 22, 2016

## ABSTRACT

Characterizing quantum systems through experimental data is critical to applications as diverse as metrology and quantum computing. Analyzing this experimental data in a robust and reproducible manner is made challenging, however, by the lack of readily-available software for performing principled statistical analysis. QInfer addresses this need. Our library makes it easy to analyze data from tomography, randomized benchmarking, and Hamiltonian learning experiments either in post-processing, or online as data is acquired. We also provide functionality for predicting the performance of a proposed experimental protocols from simulated runs.

|          |                                                  |           |
|----------|--------------------------------------------------|-----------|
| <b>1</b> | <b>Introduction</b>                              | <b>1</b>  |
| 1.1      | Installing QInfer . . . . .                      | 1         |
| 1.2      | Citing QInfer . . . . .                          | 1         |
| 1.3      | Getting Started . . . . .                        | 2         |
| <b>2</b> | <b>User's Guide</b>                              | <b>3</b>  |
| 2.1      | Simple Estimation Functions . . . . .            | 3         |
| 2.2      | Representing Probability Distributions . . . . . | 4         |
| 2.3      | Designing and Using Models . . . . .             | 5         |
| 2.4      | Sequential Monte Carlo . . . . .                 | 11        |
| 2.5      | Experiment Design Heuristics . . . . .           | 15        |
| 2.6      | Randomized Benchmarking . . . . .                | 19        |
| 2.7      | Quantum Tomography . . . . .                     | 20        |
| 2.8      | Learning Time-Dependent Models . . . . .         | 22        |
| 2.9      | Performance and Robustness Testing . . . . .     | 26        |
| 2.10     | Parallel Execution of Models . . . . .           | 31        |
| 2.11     | Interoperability . . . . .                       | 32        |
| <b>3</b> | <b>API Reference</b>                             | <b>35</b> |
| 3.1      | Abstract Model Classes . . . . .                 | 35        |
| 3.2      | Derived Models . . . . .                         | 41        |
| 3.3      | Probability Distributions . . . . .              | 44        |
| 3.4      | Domains . . . . .                                | 48        |
| 3.5      | Experiment Design Algorithms . . . . .           | 53        |
| 3.6      | GPU-Accelerated Models . . . . .                 | 55        |
| 3.7      | IPython/Jupyter Support . . . . .                | 56        |
| 3.8      | Mixin Classes for Model Development . . . . .    | 56        |
| 3.9      | Parallelized Models . . . . .                    | 57        |
| 3.10     | Performance Testing . . . . .                    | 58        |
| 3.11     | Randomized Benchmarking . . . . .                | 60        |
| 3.12     | Resampling Algorithms . . . . .                  | 61        |
| 3.13     | Simple Estimation . . . . .                      | 62        |
| 3.14     | Sequential Monte Carlo . . . . .                 | 64        |
| 3.15     | Testing Models . . . . .                         | 71        |
| 3.16     | Quantum Tomography . . . . .                     | 73        |
| 3.17     | Utility Functions . . . . .                      | 79        |
| <b>4</b> | <b>Development Guide</b>                         | <b>81</b> |
| 4.1      | Writing Documentation . . . . .                  | 81        |
| 4.2      | Unit and Documentation Testing . . . . .         | 84        |

|                           |           |
|---------------------------|-----------|
| <b>5 Acknowledgements</b> | <b>87</b> |
| <b>Bibliography</b>       | <b>89</b> |
| <b>Index</b>              | <b>91</b> |

## INTRODUCTION

**QInfer** is a library for working with sequential Monte Carlo methods for parameter estimation in quantum information. **QInfer** will use your custom experimental models to estimate properties of those models based on experimental data. Additionally, **QInfer** is designed for use with cutting-edge tools, such as Python and IPython, making it easier to integrate with the rich community of Python-based scientific software libraries.

### 1.1 Installing QInfer

We recommend using **QInfer** with the [Anaconda distribution](#). Download and install Anaconda for your platform, either Python 2.7 or 3.5. We suggest using Python 3.5, but **QInfer** works with either. Once Anaconda is installed, simply run `pip` to install **QInfer**:

```
$ pip install qinfer
```

Alternatively, **QInfer** can be installed manually by downloading from GitHub, then running the provided installer:

```
$ git clone git@github.com:QInfer/python-qinfer.git
$ cd python-qinfer
$ pip install -r requirements.txt
$ python setup.py install
```

### 1.2 Citing QInfer

If you use **QInfer** in your publication or presentation, we would appreciate it if you cited our work. We recommend citing **QInfer** by using the BibTeX entry:

```
@misc{qinfer-1_0b4,
  author      = {Christopher Granade and
                 Christopher Ferrie and
                 Steven Casagrande and
                 Ian Hincks and
                 Michal Kononenko and
                 Thomas Alexander and
                 Yuval Sanders},
  title       = {{QInfer}: Library for Statistical Inference in Quantum Information},
  month       = may,
  year        = 2016,
  doi         = {10.5281/zenodo.51273},
  url         = {http://dx.doi.org/10.5281/zenodo.51273}
}
```

If you wish to cite **QInfer** functionality that has not yet appeared in a released version, it may be helpful to cite a given SHA hash as listed on [GitHub](#) (the hashes of each commit are listed on the right hand side of the page). A recommended BibTeX entry for citing a particular commit is:

```
@misc{qinfer-1_0b4,  
  author      = {Christopher Granade and  
                 Christopher Ferrie and  
                 Steven Casagrande and  
                 Ian Hincks and  
                 Michal Kononenko and  
                 Thomas Alexander and  
                 Yuval Sanders},  
  title       = {{QInfer}: Library for Statistical Inference in Quantum Information},  
  month       = may,  
  year        = 2016,  
  url         = "https://github.com/QInfer/python-qinfer/commit/bc3736c",  
  note        = {Version \texttt{bc3736c}.}  
}
```

In this example, `bc3736c` should be replaced by the particular commit being cited, and the date should be replaced by the date of that commit.

## 1.3 Getting Started

To get started using **QInfer**, it may be helpful to give a look through the *User's Guide*. Alternatively, you may want to dive right into looking at some examples. We provide a number of [Jupyter Notebook](#)-based examples in the [qinfer-examples](#) repository. These examples can be viewed online using [nbviewer](#), or can be run online using [binder](#) without installing any additional software.

The examples can also be run locally, using the instructions available at [qinfer-examples](#).

## 2.1 Simple Estimation Functions

**QInfer** provides several functions to help you get up and running quickly with common estimation tasks, without having to worry about explicitly specifying models and distributions. Later, we'll see how to build up custom estimation problems in a straightforward and structured manner. For now, though, let's start by diving into how to use **QInfer** to learn a single precession frequency.

In particular, suppose that you have a qubit that starts in the  $|+\rangle = (|0\rangle + |1\rangle)/\sqrt{2}$  state, then evolves under  $U(t) = \exp(-i\omega\sigma_z)$  for an unknown frequency  $\omega$ . Then measuring the qubit in the  $\sigma_x$  basis results in observing a 1 with probability  $\sin^2(\omega t/2)$ . We can estimate the precession frequency  $\omega$  with **QInfer** using the `simple_est_prec()` function.

As an example, let's consider an experiment for learning  $\omega$  that consists of taking 40 measurements at each time  $t_k = k/(2\omega_{\max})$ , where  $k = 0, \dots, N - 1$  indexes each measurement,  $\omega_{\max}$  is the maximum plausible frequency to be estimated, and where  $N$  is the number of distinct times measured. We can generate this data using `binomial()`:

```
>>> omega_max = 100
>>> true_omega = 70.3
>>> ts = np.arange(1, 51) / (2 * omega_max)
>>> counts = np.random.binomial(40, p=np.sin(true_omega * ts / 2) ** 2)
```

We pass this data to **QInfer** as an array with three *columns* (that is, shape `(50, 3)` for this example), corresponding respectively to the observed counts, the time at which the counts were observed, and the number of measurements taken at that time.

```
>>> data = np.column_stack([counts, ts, np.ones_like(counts) * 40])
```

Finally, we're ready to call `simple_est_prec()`:

```
>>> from qinfer import simple_est_prec
>>> mean, cov = simple_est_prec(data, freq_max=omega_max)
```

The returned `mean` and `cov` tell us the mean and covariance, respectively, resulting from the frequency estimation problem.

```
>>> print(mean)
70.3822376258
```

Data can also be passed to `simple_est_prec()` as a string containing the name of a CSV-formatted data file, or as a **Pandas DataFrame**. The latter is especially useful for loading data from formats such as Excel spreadsheets, using `read_excel()`.

For more information, please see the [API reference](#) or the examples below.

### 2.1.1 Related Examples

- `simple_precession_example`
- `randomized_benchmarking`

## 2.2 Representing Probability Distributions

### 2.2.1 Introduction

Probability distributions such as prior distributions over model parameters are represented in QInfer by objects of type `Distribution` that are responsible for producing samples according to those distributions. This is especially useful, for instance, when drawing initial particles for use with an `SMCUpdater`.

The approach to representing distributions taken by QInfer is somewhat different to that taken by, for example, `scipy.stats`, in that a QInfer `Distribution` is a class that produces samples according to that distribution. This means that QInfer `Distribution` objects provide much less information than do those represented by objects in `scipy.stats`, but that they are much easier to write and combine.

### 2.2.2 Sampling Pre-made Distributions

QInfer comes along with several distributions, listed in *Specific Distributions*. Each of these is a subclass of `Distribution`, and hence has a method `sample()` that produces an array of samples.

```
>>> from qinfer import NormalDistribution
>>> dist = NormalDistribution(0, 1)
>>> samples = dist.sample(n=5)
>>> samples.shape == (5, 1)
True
```

### 2.2.3 Combining Distributions

Distribution objects can be combined using other distribution objects. For instance, if  $a \sim \mathcal{N}(0, 1)$  and  $b \sim \text{Uni}(0, 1)$ , then the product distribution on  $(a, b)$  can be produced by using `ProductDistribution`:

```
>>> from qinfer import UniformDistribution, ProductDistribution
>>> a = NormalDistribution(0, 1)
>>> b = UniformDistribution([0, 1])
>>> ab = ProductDistribution(a, b)
>>> samples = ab.sample(n=5)
>>> samples.shape == (5, 2)
True
```

### 2.2.4 Making Custom Distributions

To make a custom distribution, one need only implement `sample()` and set the property `n_rvs` to indicate how many random variables the new distribution class represents.

For example, to implement a distribution over  $x$  and  $y$  such that  $\sqrt{x^2 + y^2} \sim \mathcal{N}(1, 0.1)$  and such that the angle between  $x$  and  $y$  is drawn from  $\text{Uni}(0, 2\pi)$ :

```

from qinfer import Distribution

class RingDistribution(Distribution):
    @property
    def n_rvs(self):
        return 2

    def sample(self, n=1):
        r = np.random.randn(n, 1) * 0.1 + 1
        th = np.random.random((n, 1)) * 2 * np.pi

        x = r * np.cos(th)
        y = r * np.sin(th)

        return np.concatenate([x, y], axis=1)

```

## 2.3 Designing and Using Models

### 2.3.1 Introduction

The concept of a **model** is key to the use of QInfer. A model defines the probability distribution over experimental data given hypotheses about the system of interest, and given a description of the measurement performed. This distribution is called the *likelihood function*, and it encapsulates the definition of the model.

In QInfer, likelihood functions are represented as classes inheriting from either *Model*, when the likelihood function can be numerically evaluated, or *Simulatable* when only samples from the function can be efficiently generated.

### 2.3.2 Using Models and Simulations

#### Basic Functionality

Both *Model* and *Simulatable* offer basic functionality to describe how they are parameterized, what outcomes are possible, etc. For this example, we will use a premade model, *SimplePrecessionModel*. This model implements the likelihood function

$$\Pr(d|\omega; t) = \begin{cases} \cos^2(\omega t/2) & d = 0 \\ \sin^2(\omega t/2) & d = 1 \end{cases},$$

as can be derived from Born's Rule for a spin- $\frac{1}{2}$  particle prepared and measured in the  $|+\rangle \propto |0\rangle + |1\rangle$  state, and evolved under  $H = \omega\sigma_z/2$  for some time  $t$ .

In this way, we see that by defining the likelihood function in terms of the hypothetical outcome  $d$ , the model parameter  $\omega$ , and the experimental parameter  $t$ , we can reason about the experimental data that we would extract from the system.

In order to use this likelihood function, we must instantiate the model that implements the likelihood. Since *SimplePrecessionModel* is provided with QInfer, we can simply import it and make an instance.

```

>>> from qinfer import SimplePrecessionModel
>>> m = SimplePrecessionModel()

```

Once a model or simulator has been created, you can query how many model parameters it admits and how many outcomes a given experiment can have.



```
>>> print(m.n_modelparams)
1
>>> print(m.modelparam_names)
['\\omega']
>>> print(m.is_n_outcomes_constant)
True
>>> print(m.n_outcomes(expparams=0))
2
```

## Model and Experiment Parameters

The division between unknown parameters that we are trying to learn ( $\omega$  in the *SimplePrecessionModel* example) and the controls that we can use to design measurements ( $t$ ) is generic, and is key to how QInfer handles the problem of parameter estimation. Roughly speaking, model parameters are real numbers that represent properties of the system that we would like to learn, whereas experiment parameters represent the choices we get to make in performing measurements.

Model parameters are represented by NumPy arrays of dtype `float` and that have two indices, one representing which model is being considered and one representing which parameter. That is, model parameters are defined by matrices such that the element  $X_{ij}$  is the  $j^{\text{th}}$  parameter of the model parameter vector  $x_i$ .

By contrast, since not all experiment parameters are best represented by the data type `float`, we cannot use an array of homogeneous dtype unless there is only one experimental parameter. The alternative is to use NumPy's `record array` functionality to specify the *heterogeneous* type of the experiment parameters. To do so, instead of using a second index to refer to specific experiment parameters, we use *fields*. Each field then has its own dtype.

For instance, a dtype of `[('t', 'float'), ('basis', 'int')]` specifies that an array has two fields, named `t` and `basis`, having dtypes of `float` and `int`, respectively. Such arrays are initialized by passing lists of *tuples*, one for each field:

```
>>> eps = np.array([
...     (12.3, 2),
...     (14.1, 1)
... ], dtype=[('t', 'float'), ('basis', 'int')])
>>> print(eps)
[(12.3, 2) (14.1, 1)]
>>> eps.shape == (2,)
True
```

Once we have made a record array, we can then index by field names to get out each field as an array of that field's value in each record, or we can index by record to get all fields.

```
>>> print(eps['t'])
[ 12.3  14.1]
>>> print(eps['basis'])
[2 1]
>>> print(eps[0])
(12.3, 2)
```

Model classes specify the dtypes of their experimental parameters with the property `expparams_dtype`. Thus, a common idiom is to pass this property to the dtype keyword of NumPy functions. For example, the model class *BinomialModel* adds an `int` field specifying how many times a two-outcome measurement is repeated, so to specify that we can use its `expparams_dtype`:

```
>>> from qinfer import BinomialModel
>>> bm = BinomialModel(m)
>>> print(bm.expparams_dtype)
[('x', 'float'), ('n_meas', 'uint')]
```

```
>>> eps = np.array([
...     (5.0, 10)
... ], dtype=bm.expparams_dtype)
```

## Model Outcomes

Given a specific vector of model parameters  $\mathbf{x}$  and a specific experimental configuration  $\mathbf{c}$ , the experiment will yield some *outcome*  $d$  according to the model distribution  $\Pr(d|\mathbf{x}, \mathbf{c})$ .

In many cases, such as *SimplePrecessionModel* discussed above, there will be a finite number of outcomes, which we can label by some finite set of integers. For example, we labeled the outcome  $|0\rangle$  by  $d = 0$  and the outcome  $|1\rangle$  by  $d = 1$ . If this is the case for you, the rest of this section will likely not be very relevant, and you may assume your outcomes are zero-indexed integers ending at some value.

In other cases, there may be an infinite number of possible outcomes. For example, if the measurement returns the total number of photons measured in a time window, which can in principle be arbitrarily large, or if the measurement is of a voltage or current, which can be any real number. Or, we may have outcomes which require fancy data types. For instance, perhaps the output of a single experiment is a tuple of numbers rather than a single number.

To accomodate these possible situations, and to have a systematic way of testing whether or not all possible outcomes can be enumerated, *Simulatable* (and subclasses like *Model*) has a method *domain* which for every given experimental parameter, returns a *Domain* object. One major benefit of explicitly storing these objects is that certain quantities (like *bayes\_risk*) can be computed much more efficiently when all possible outcomes can be enumerated. *Domain* has attributes which specify whether or not it are finite, how many members it has and what they are, what data type they are, and so on.

For the *BinomialModel* defined above, there are `n_meas+1` possible outcomes, with possible values the integers between 0 and `n_meas` inclusive.

```
>>> bdomain = bm.domain(eps)[0]
>>> bdomain.n_members
11
>>> bdomain.values
array([ 0,  1,  2,  3,  4,  5,  6,  7,  8,  9, 10])
>>> bdomain.dtype == np.int
True
```

We need to extract the 0<sup>th</sup> element of `bm.domain(eps)` above because `eps` is a vector of length 1 and *domain* always returns one domain for every member of `eps`. In the case where the domain is completely independent of `eps`, it should be possible to call `m.domain(None)` to return the unique domain of the model `m`.

The *MultinomialModel* requires a fancy datatype so that outcomes can be tuples of integers. In the following a single experiment of the model `mm` consists of throwing a four sided die `n_meas` times and recording how many times each side lands facing down.

```
>>> from qinfer import MultinomialModel, NDieModel
>>> mm = MultinomialModel(NDieModel(n=4))
>>> mm.expparams_dtype
[('exp_num', 'int'), ('n_meas', 'uint')]
>>> mmeeps = np.array([(1, 3)], dtype=mm.expparams_dtype)
>>> mmdomain = mm.domain(mmeeps)[0]
>>> mmdomain.dtype
dtype([('k', '<i8', (4,))])
>>> mmdomain.n_members
20
>>> print(mmdomain.values)
[([3, 0, 0, 0],) ([2, 1, 0, 0],) ([2, 0, 1, 0],) ([2, 0, 0, 1],)
 ([1, 2, 0, 0],) ([1, 1, 1, 0],) ([1, 1, 0, 1],) ([1, 0, 2, 0],)
```

```
([1, 0, 1, 1],) ([1, 0, 0, 2],) ([0, 3, 0, 0],) ([0, 2, 1, 0],)
([0, 2, 0, 1],) ([0, 1, 2, 0],) ([0, 1, 1, 1],) ([0, 1, 0, 2],)
([0, 0, 3, 0],) ([0, 0, 2, 1],) ([0, 0, 1, 2],) ([0, 0, 0, 3],)
```

We see here all 20 possible ways to roll this die four times.

---

**Note:** `Model` inherits from `Simulatable`, and `FiniteOutcomeModel` inherits from `Model`. The subclass `FiniteOutcomeModel` is able to concretely define some methods (like `simulate_experiment`) because of the guarantee that all domains have a finite number of elements. Therefore, it is generally a bit less work to construct a `FiniteOutcomeModel` than it is to construct a `Model`.

Additionally, `FiniteOutcomeModel` automatically defines the domain corresponding to the experimental parameter `ep` by looking at `n_outcomes`, namely, if `nep=n_outcomes(ep)`, then the corresponding domain has members `0, 1, ..., nep` by default.

Finally, make note of the slightly subtle role of the method `n_outcomes`. In principle, `n_outcomes` is completely independent of `domain`. For `FiniteOutcomeModel`, it will almost always hold that `m.n_outcomes(ep)==domain(ep)[0].n_members`. For models with an infinite number of outcomes, `n_members` is not defined, but `n_outcomes` is defined and refers to “enough outcomes” (at the user’s discretion) to make estimates of quantities `bayes_risk`.

---

## Simulation

Both models and simulators allow for simulated data to be drawn from the model distribution using the `simulate_experiment()` method. This method takes a matrix of model parameters and a vector of experiment parameter records or scalars (depending on the model or simulator), then returns an array of sample data, one sample for each combination of model and experiment parameters.

```
>>> modelparams = np.linspace(0, 1, 100)
>>> expparams = np.arange(1, 10) * np.pi / 2
>>> D = m.simulate_experiment(modelparams, expparams, repeat=3)
>>> print(isinstance(D, np.ndarray))
True
>>> D.shape == (3, 100, 9)
True
```

If exactly one datum is requested, `simulate_experiment()` will return a scalar:

```
>>> print(m.simulate_experiment(np.array([0.5]), np.array([3.5 * np.pi]), repeat=1).shape)
()
```

Note that in NumPy, a shape tuple of length zero indicates a scalar value, as such an array has no indices.

---

**Note:** For models with fancy outcome datatypes, it is demanded that the outcome data types, `[d.dtype for d in m.domain(expparams)]`, be identical for every experimental parameter `expparams` being simulated. This can be checked with `are_expparam_datypes_consistent`.

---

## Likelihoods

The core functionality of `Model`, however, is the `likelihood()` method. This takes vectors of outcomes, model parameters and experiment parameters, then returns for each combination of the three the corresponding probability  $\Pr(d|\mathbf{x}; e)$ .

```
>>> modelparams = np.linspace(0, 1, 100)
>>> expparams = np.arange(1, 10) * np.pi / 2
>>> outcomes = np.array([0], dtype=int)
>>> L = m.likelihood(outcomes, modelparams, expparams)
```

The return value of `likelihood()` is a three-index array of probabilities whose shape is given by the lengths of `outcomes`, `modelparams` and `expparams`. In particular, `likelihood()` returns a rank-three tensor  $L_{ijk} := \Pr(d_i | x_j; e_k)$ .

```
>>> print(isinstance(L, np.ndarray))
True
>>> L.shape == (1, 100, 9)
True
```

### 2.3.3 Implementing Custom Simulators and Models

In order to implement a custom simulator or model, one must specify metadata describing the number of outcomes, model parameters, experimental parameters, etc. in addition to implementing the simulation and/or likelihood methods.

Here, we demonstrate how to do so by walking through a simple subclass of `FiniteOutcomeModel`. For more detail, please see the [API Reference](#).

Suppose we wish to implement the likelihood function

$$\Pr(0 | \omega_1, \omega_2; t_1, t_2) = \cos^2(\omega_1 t_1 / 2) \cos^2(\omega_2 t_2 / 2),$$

as may arise in looking, for instance, at an experiment inspired by 2D NMR. This model has two model parameters,  $\omega_1$  and  $\omega_2$ , and so we start by creating a new class and declaring the number of model parameters as a `property`:

```
from qinfer import FiniteOutcomeModel
import numpy as np

class MultiCosModel(FiniteOutcomeModel):

    @property
    def n_modelparams(self):
        return 2
```

Next, we proceed to add a property and method indicating that this model always admits two outcomes, irrespective of what measurement is performed. This will also automatically define the `domain` method.

```
@property
def is_n_outcomes_constant(self):
    return True
def n_outcomes(self, expparams):
    return 2
```

We indicate the valid range for model parameters by returning an array of dtype `bool` for each of an input matrix of model parameters, specifying whether each model vector is valid or not (this is important in resampling, for instance, to make sure particles don't move to bad locations). Typically, this will look like some typical bounds checking, combined using `logical_and` and `all`. Here, we follow that model by insisting that *all* elements of each model parameter vector must be at least 0, *and* must not exceed 1.

```
def are_models_valid(self, modelparams):
    return np.all(np.logical_and(modelparams > 0, modelparams <= 1), axis=1)
```

Next, we specify what a measurement looks like by defining `expparams_dtype`. In this case, we want one field that is an array of two `float` elements:

```
@property
def expparams_dtype(self):
    return [('ts', 'float', 2)]
```

Finally, we write the likelihood itself. Since this is a two-outcome model, we can calculate the rank-two tensor  $p_{jk} = \Pr(0|x_j; e_k)$  and let `pr0_to_likelihood_array()` add an index over outcomes for us so  $L_{0jk} = p_{jk}$  and  $L_{1jk} = 1 - p_{jk}$ . To compute  $p_{jk}$  efficiently, it is helpful to do a bit of index gymnastics using NumPy's powerful [broadcasting rules](#). In this example, we set up the calculation to produce terms of the form  $\cos^2(x_{j,l}e_{k,l}/2)$  for  $l \in \{0,1\}$  indicating whether we're referring to  $\omega_1$  or  $\omega_2$ , respectively. Multiplying along this axis then gives us the product of the two cosine functions, and in a way that very nicely generalizes to likelihood functions of the form

$$\Pr(0|\omega_1, \omega_2; t_1, t_2) = \prod_l \cos^2(\omega_l t_l / 2).$$

Running through the index gymnastics, we can implement the likelihood function as:

```
def likelihood(self, outcomes, modelparams, expparams):
    # We first call the superclass method, which basically
    # just makes sure that call count diagnostics are properly
    # logged.
    super(MultiCosModel, self).likelihood(outcomes, modelparams, expparams)

    # Next, since we have a two-outcome model, everything is defined by
    # Pr(0 | modelparams; expparams), so we find the probability of 0
    # for each model and each experiment.
    #
    # We do so by taking a product along the modelparam index (len 2,
    # indicating omega_1 or omega_2), then squaring the result.
    pr0 = np.prod(
        np.cos(
            # shape (n_models, 1, 2)
            modelparams[:, np.newaxis, :] *
            # shape (n_experiments, 2)
            expparams['ts']
        ), # <- broadcasts to shape (n_models, n_experiments, 2).
        axis=2 # <- product over the final index (len 2)
    ) ** 2 # square each element

    # Now we use pr0_to_likelihood_array to turn this two index array
    # above into the form expected by SMCUpdater and other consumers
    # of likelihood().
    return FiniteOutcomeModel.pr0_to_likelihood_array(outcomes, pr0)
```

Our new custom model is now ready to use! To simulate data from this model, we set up `modelparams` and `expparams` as before, taking care to conform to the `expparams_dtype` of our model:

```
>>> mcm = MultiCosModel()
>>> modelparams = np.dstack(np.mgrid[0:1:100j, 0:1:100j]).reshape(-1, 2)
>>> expparams = np.empty((81,), dtype=mcm.expparams_dtype)
>>> expparams['ts'] = np.dstack(np.mgrid[1:10, 1:10] * np.pi / 2).reshape(-1, 2)
>>> D = mcm.simulate_experiment(modelparams, expparams, repeat=2)
>>> print(isinstance(D, np.ndarray))
True
>>> D.shape == (2, 10000, 81)
True
```

---

**Note:** Creating `expparams` as an empty array and filling it by field name is a straightforward way to make sure it matches `expparams_dtype`, but it comes with the risk of forgetting to initialize a field, so take care when using this method.

---

### 2.3.4 Adding Functionality to Models with Other Models

QInfer also provides model classes which add functionality or otherwise modify other models. For instance, the `BinomialModel` class accepts instances of two-outcome models and then represents the likelihood for many repeated measurements of that model. This is especially useful in cases where experimental concerns make switching experiments costly, such that repeated measurements make sense.

To use `BinomialModel`, simply provide an instance of another model class:

```
>>> from qinfer import SimplePrecessionModel
>>> from qinfer import BinomialModel
>>> bin_model = BinomialModel(SimplePrecessionModel())
```

Experiments for `BinomialModel` have an additional field from the underlying models, called `n_meas`. If the original model used scalar experiment parameters (e.g.: `expparams_dtype` is `float`), then the original scalar will be referred to by a field `x`.

```
>>> eps = np.array([(12.1, 10)], dtype=bin_model.expparams_dtype)
>>> print(eps['x'], eps['n_meas'])
[ 12.1] [10]
```

Another model which *decorates* other models in this way is `PoisonedModel`, which is discussed in more detail in *Performance and Robustness Testing*. Roughly, this model causes the likelihood functions calculated by its underlying model to be subject to random noise, so that the robustness of an inference algorithm against such noise can be tested.

## 2.4 Sequential Monte Carlo

### 2.4.1 Introduction

Arguably the core of QInfer, the `qinfer.smc` module implements the sequential Monte Carlo algorithm in a flexible and robust manner. At its most basic, using QInfer's SMC implementation consists of specifying a model, a prior, and a number of SMC particles to use.

The main component of QInfer's SMC support is the `SMCUpdater` class, which performs Bayesian updates on a given prior in response to new data. In doing so, `SMCUpdater` will also ensure that the posterior particles are properly resampled. For more details on the SMC algorithm as implemented by QInfer, please see [\[GFWC12\]](#).

### 2.4.2 Using SMCUpdater

#### Creating and Configuring Updaters

The most straightforward way of creating an `SMCUpdater` instance is to provide a model, a number of SMC particles and a prior distribution to choose those particles from. Using the example of a `SimplePrecessionModel`, and a uniform prior  $\omega \sim \text{Uni}(0, 1)$ :

```
>>> from qinfer import SMCUpdater, UniformDistribution, SimplePrecessionModel
>>> model = SimplePrecessionModel()
>>> prior = UniformDistribution([0, 1])
>>> updater = SMCUpdater(model, 1000, prior)
```

## Updating from Data

Once an updater has been created, one can then use it to update the prior distribution to a posterior conditioned on experimental data. For example,

```
>>> true_model = prior.sample()
>>> experiment = np.array([12.1], dtype=model.expparams_dtype)
>>> outcome = model.simulate_experiment(true_model, experiment)
>>> updater.update(outcome, experiment)
```

## Drawing Posterior Samples and Estimates

Since *SMCUpdater* inherits from *Distribution*, it can be sampled in the same way described in *Representing Probability Distributions*.

```
>>> posterior_samples = updater.sample(n=100)
>>> posterior_samples.shape == (100, 1)
True
```

More commonly, however, one will want to calculate estimates such as  $\hat{x} = \mathbb{E}_{x|\text{data}}[x]$ . These estimates are given methods such as *est\_mean()* and *est\_covariance\_mtx()*.

```
>>> est = updater.est_mean()
>>> print(est)
[ 0.53147953]
```

## Plotting Posterior Distributions

The *SMCUpdater* also provides tools for producing plots to describe the updated posterior. For instance, the *plot\_posterior\_marginal()* method uses kernel density estimation to plot the marginal over all but a single parameter over the posterior.

```
prior = UniformDistribution([0, 1])
model = SimplePrecessionModel()
updater = SMCUpdater(model, 2000, prior)

# Plot according to the initial prior.
updater.plot_posterior_marginal()

# Simulate 50 different measurements and use
# them to update.
true = prior.sample()
heuristic = ExpSparseHeuristic(updater)

for idx_exp in range(25):
    expparams = heuristic()
    datum = model.simulate_experiment(true, expparams)
    updater.update(datum, expparams)

# Plot the posterior.
```

```

updater.plot_posterior_marginal()

# Add a legend and show the final plot.
plt.legend(['Prior', 'Posterior'])
plt.show()

```

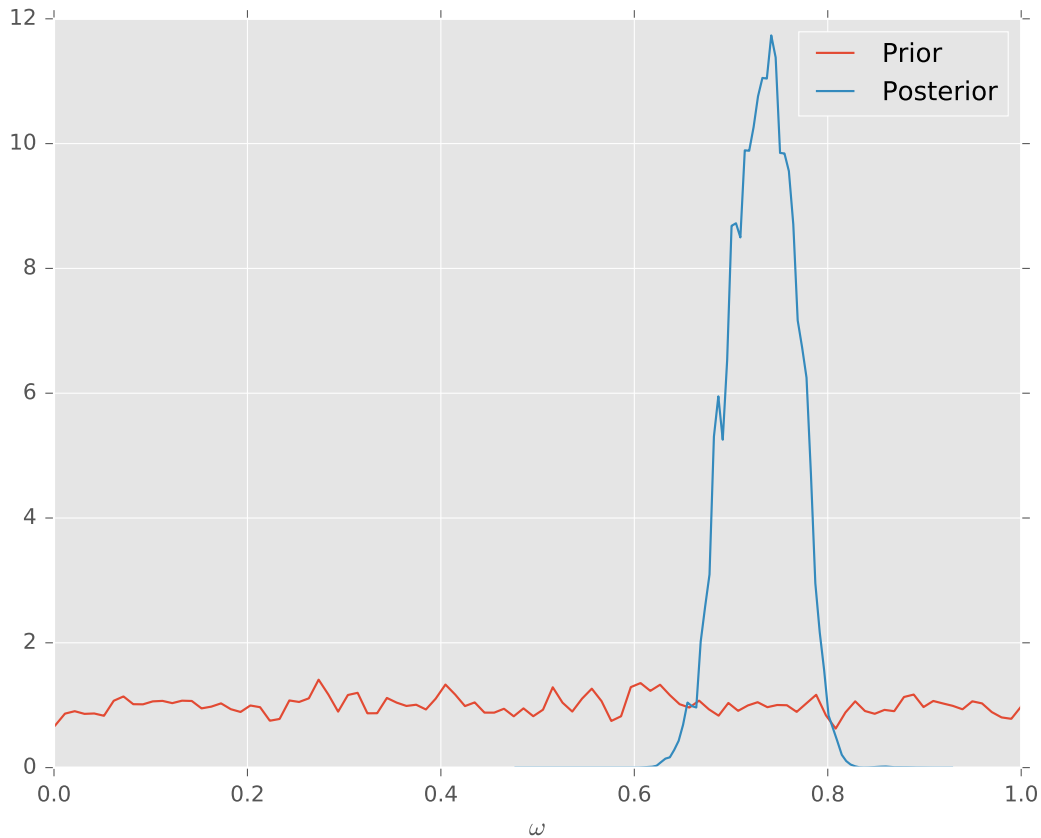

For multi-parameter models, the `plot_covariance()` method plots the covariance matrix for the current posterior as a [Hinton diagram](#). That is, positive elements are shown as white squares, while negative elements are shown as black squares. The relative sizes of each square indicate the magnitude, making it easy to quickly identify correlations that impact estimator performance. In the example below, we use the [Simple Estimation Functions](#) to quickly analyze [Randomized Benchmarking](#) data and show the resulting correlation between the  $p$ ,  $A$  and  $B$  parameters. For more detail, please see the [randomized benchmarking example](#).

```

p = 0.995
A = 0.5
B = 0.5

ms = np.linspace(1, 800, 201).astype(int)
signal = A * p ** ms + B

n_shots = 25
counts = np.random.binomial(p=signal, n=n_shots)

data = np.column_stack([counts, ms, n_shots * np.ones_like(counts)])
mean, cov, extra = simple_est_rb(data, return_all=True, n_particles=12000, p_min=0.8)
extra['updater'].plot_covariance()

```



```
plt.show()
```

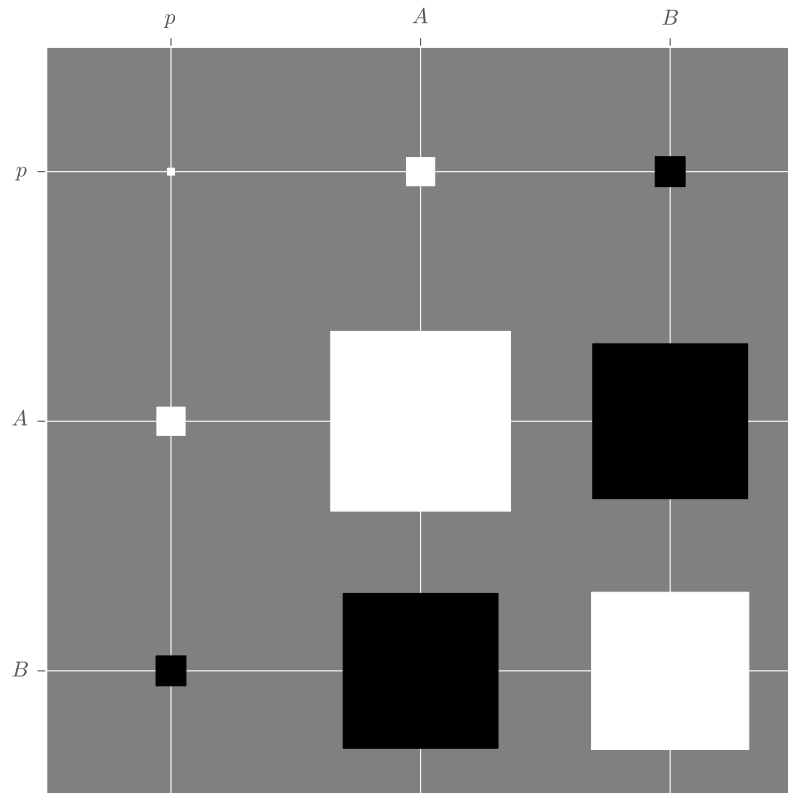

## 2.4.3 Advanced Usage

### Custom Resamplers

By default, `SMCUpdater` uses the Liu and West resampling algorithm [LW01] with  $a = 0.98$ . The resampling behavior can be controlled, however, by passing resampler objects to `SMCUpdater`. For instance, if one wants to create an updater with  $a = 0.9$  as was suggested by [WGFC13a]:

```
>>> from qinfer import LiuWestResampler
>>> updater = SMCUpdater(model, 1000, prior, resampler=LiuWestResampler(0.9))
```

This causes the resampling procedure to more aggressively approximate the posterior as a Gaussian distribution, and can allow for a much smaller number of particles to be used when the Gaussian approximation is accurate. For multimodal problems, it can make sense to relax the requirement that the resampler preserve the mean and covariance, and to instead allow the resampler to increase the uncertainty. For instance, the modified Liu-West resampler  $a = 1$  and  $h = 0.005$  can accurately find exactly degenerate peaks in precession models [Gra15].

## Posterior Credible Regions

Posterior credible regions can be found by using the `est_credible_region()` method. This method returns a set of points  $\{x'_i\}$  such that the sum  $\sum_i w'_i$  of the corresponding weights  $\{w'_i\}$  is at least a specified ratio of the total weight.

This does not admit a very compact description, however, such that it is useful to find region estimators  $\hat{X}$  containing all of the particles describing a credible region, as above.

The `region_est_hull()` method does this by finding a convex hull of the credible particles, while `region_est_ellipsoid()` finds the minimum-volume enclosing ellipse (MVEE) of the convex hull region estimator.

The derivation of these estimators, as well as a detailed discussion of their performances, can be found in [GFWC12] and [Fer14].

## Online Bayesian Cramer-Rao Bound Estimation

TODO

## Model Selection with Bayes Factors

When considering which of two models  $A$  or  $B$  best explains a data record  $D$ , the normalizations of SMC updates of the posterior conditioned on each provide the probabilities  $\Pr(D|A)$  and  $\Pr(D|B)$ . The normalization records can be obtained from the `normalization_record` properties of each. As the probabilities of any individual data record quickly reach zero, however, it becomes numerically unstable to consider these probabilities directly. Instead, the property `log_total_likelihood` records the quantity

$$\ell(D|M) = \sum_i \log \Pr(d_i|M)$$

for  $M \in \{A, B\}$ . This is related to the Bayes factor  $f$  by

$$f = \exp(\ell(D|A) - \ell(D|B)).$$

As discussed in [WGFC13b], the Bayes factor tells which of the two models under consideration is to be preferred as an explanation for the observed data.

## 2.5 Experiment Design Heuristics

### 2.5.1 Using Heuristics in Updater Loops

During an experiment, the current posterior distribution represented by an `SMCUpdater` instance can be used to *adaptively* make decisions about which measurements should be performed. For example, utility functions such as the information gain and negative variance can be used to choose optimal measurements.

On the other hand, this optimization is generally quite computationally expensive, such that many less optimal measurements could have been performed before an optimization step completes. Philosophically, there are no “bad” experiments, in that even suboptimal measurements can still carry useful information about the parameters of interest.

In light of this, it can be substantially less expensive to use a *heuristic* function of prior information to select experiments without explicit optimization. For example, consider the single-parameter inversion precession model with model parameters  $x = (\omega)$ , experiment parameters  $e = (\omega_-, t)$  and likelihood function

$$\Pr(1|\omega; \omega_-, t) = \sin^2([\omega - \omega_-]t/2).$$

For a given posterior distribution, the *particle guess heuristic* (PGH) [WGFC13a] then chooses  $\omega_-$  and  $t$  for the next experiment by first sampling two particles  $\omega_-$  and  $\omega'_-$  from the posterior. The PGH then assigns the time  $t = 1/|\omega_- - \omega'_-|$ .

**QInfer** implements heuristics as subtypes of *Heuristic*, each of which take an updater and can be called to produce experimental parameters. For example, the PGH is implemented by the class *PGH*, and can be used in an updater loop to adaptively select experiments.

```

model = SimpleInversionModel()
prior = UniformDistribution([0, 1])
updater = SMCUpdater(model, 1000, prior)
heuristic = PGH(updater, inv_field='w_', t_field='t')

true_omega = prior.sample()

ts = []
est_omegas = []

for idx_exp in range(100):
    experiment = heuristic()
    datum = model.simulate_experiment(true_omega, experiment)
    updater.update(datum, experiment)

    ts.append(experiment['t'])
    est_omegas.append(updater.est_mean())

ax = plt.subplot(2, 1, 1)
plt.semilogy((est_omegas - true_omega) ** 2)
plt.ylabel('Squared Error')

plt.subplot(2, 1, 2, sharex=ax)
plt.semilogy(ts)
plt.xlabel('# of Measurements')
plt.ylabel('$t$')

plt.show()

```

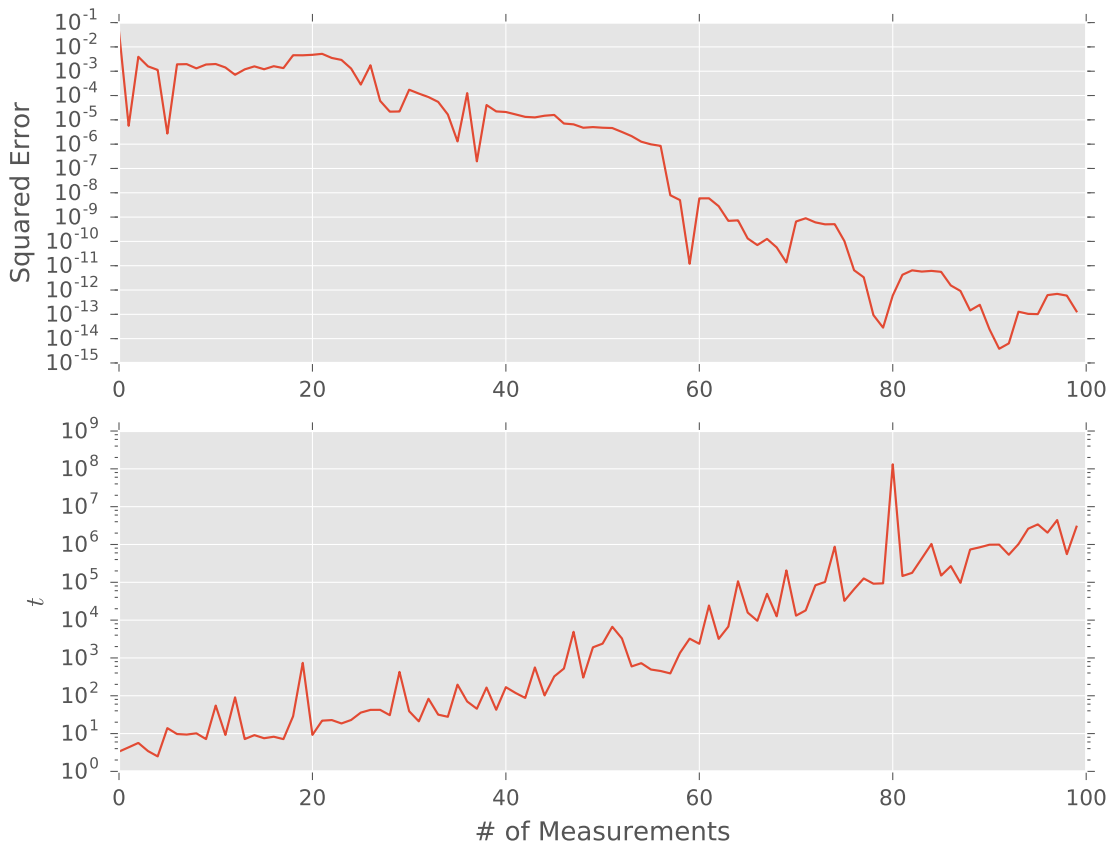

## 2.5.2 Changing Heuristic Parameters

Essentially, heuristics in **QInfer** are functions that take *SMCUpdater* instances and return functions that then yield experiments. This design allows for specializing heuristics by providing other arguments along with the updater. For instance, the *ExpSparseHeuristic* class implements exponentially-sparse sampling  $t_k = ab^k$  for *SimplePrecessionModel*. Both  $a$  and  $b$  are parameters of the heuristic, named *scale* and *base*, respectively. Thus, it is easy to override the defaults to obtain different heuristics.

```
model = SimplePrecessionModel()
prior = UniformDistribution([0, 1])
updater = SMCUpdater(model, 1000, prior)
heuristic = ExpSparseHeuristic(updater, scale=0.5)

true_omega = prior.sample()
est_omegas = []

for idx_exp in range(100):
    experiment = heuristic()
    datum = model.simulate_experiment(true_omega, experiment)
    updater.update(datum, experiment)

    est_omegas.append(updater.est_mean())

plt.semilogy((est_omegas - true_omega) ** 2)
```

```
plt.xlabel('# of Measurements')
plt.ylabel('Squared Error')

plt.show()
```

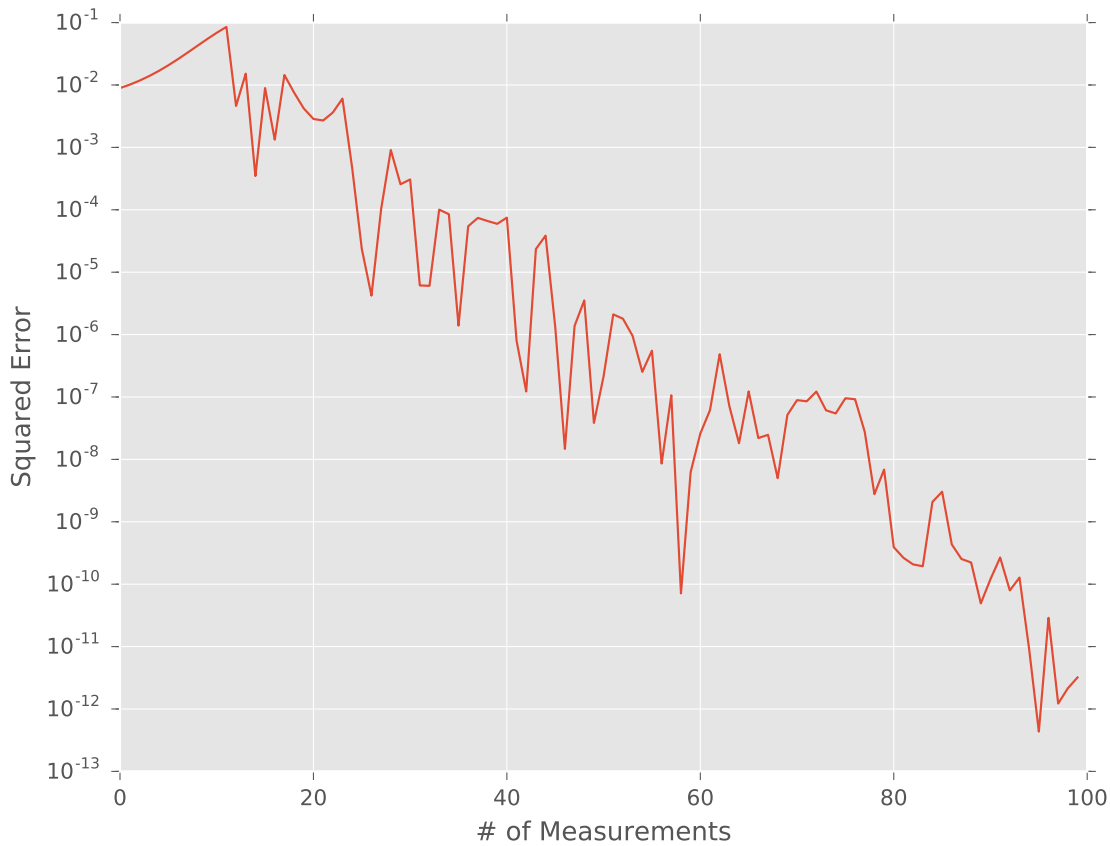

In overriding the default parameters of heuristics, the `functools.partial()` function provided with the Python standard library is especially useful, as it allows for easily making new heuristics with different default parameter values:

```
>>> from qinfer import ExpSparseHeuristic
>>> from functools import partial
>>> rescaled_heuristic_class = partial(ExpSparseHeuristic, scale=0.01)
```

Later, once we have an updater, we can then make new instances of our rescaled heuristic.

```
>>> heuristic = rescaled_heuristic_class(updater)
```

This technique is especially useful in *Performance Testing*, as it makes it easy to modify existing heuristics by changing default parameters through partial application.

## 2.6 Randomized Benchmarking

### 2.6.1 Introduction

Randomized benchmarking allows for extracting information about the fidelity of a quantum operation by exploiting *twirling* errors over an approximate implementation of the Clifford group [KL+08]. This provides the advantage that the fidelity can be learned without simulating the dynamics of a quantum system. Instead, benchmarking admits an analytic form for the survival probability for an arbitrary input state in terms of the strength  $p$  of an equivalent depolarizing channel.

**QInfer** supports randomized benchmarking by implementing this survival probability as a *likelihood function*. This allows for randomized benchmarking to be used together with *Sequential Monte Carlo*, such that prior information can be incorporated and robustness to finite sampling can be obtained [GFC14].

Regardless of the order or interleaving mode, each model instance for randomized benchmarking yields 0/1 data, with 1 indicating a survival (measuring the same state after applying a gate sequence as was initially prepared). To use these models with data batched over many sequences, model instances can be augmented by *BinomialModel*.

### 2.6.2 Zeroth-Order Model

The *RandomizedBenchmarkingModel* class implements randomized benchmarking as a **QInfer** model, both in interleaved and non-interleaved modes. For the non-interleaved mode, there are three model parameters,  $\mathbf{x} = (p, A_0, B_0)$ , given by [MGE12] as

$$\begin{aligned} A_0 &:= \text{Tr} \left[ E_\psi \Lambda \left( \rho_\psi - \frac{\mathbb{1}}{d} \right) \right] \\ B_0 &:= \text{Tr} \left[ E_\psi \Lambda \left( \frac{\mathbb{1}}{d} \right) \right] \\ p &:= (dF_{\text{ave}} - 1)/(d - 1), \end{aligned}$$

where  $E_\psi$  is the measurement,  $\rho_\psi$  is the state preparation,  $\Lambda$  is the average map over timesteps and gateset elements,  $d$  is the dimension of the system, and where  $F_{\text{ave}}$  is the average gate fidelity, taken over the gateset. The functions  $p$  and  $F$  convert back and forth between depolarizing parameters and fidelities.

An experiment parameter vector for this model is simply a specification of  $m$ , the length of the Clifford sequence used for that datum. Since *RandomizedBenchmarkingModel* represents 0/1 data, it is common to wrap this model in a *BinomialModel*:

```
>>> from qinfer import BinomialModel
>>> from qinfer import RandomizedBenchmarkingModel
>>> model = BinomialModel(RandomizedBenchmarkingModel(order=0, interleaved=False))
>>> expparams = np.array([
...     (100, 1000) # 1000 shots of sequences with length 100.
... ], dtype=model.expparams_dtype)
```

### Interleaved Mode

If one is interested in the fidelity of a single gate, rather than an entire gateset, then the gate of interest can be interleaved with other gates from the gateset to isolate its performance. In this mode, models admit an additional model and experiment parameter,  $\tilde{p}$  and  $\text{mode}$ , respectively. The  $\tilde{p}$  model parameter is the depolarizing strength of the twirl of the interleaved gate, such that the interleaved survival probability is given by

$$\text{Pr}(\text{survival} | \tilde{p}, p_{\text{ref}}, A_0, B_0; m, \text{interleaved}) = A_0(\tilde{p}p_{\text{ref}})^m + B_0.$$

Model instances for interleaved mode are constructed using the `interleaved=True` keyword argument:

```
>>> from qinfer.rb import RandomizedBenchmarkingModel
>>> model = RandomizedBenchmarkingModel(interleaved=True)
```

## 2.7 Quantum Tomography

### 2.7.1 Introduction

Tomography is the most common quantum statistical problem being the subject of both theoretical and practical studies. The `qinfer.tomography` module has rich support for many of the common models of tomography including standard distributions and heuristics, and also provides convenient plotting tools.

If the quantum state of a system is  $\rho$  and a measurement is obtained, then the probability of obtaining the outcome associated with effect  $E$  is  $\Pr(E|\rho) = \text{Tr}(\rho E)$ , the Born rule. The tomography problem is the inverse problem and is succinctly stated as follows. Given an unknown state  $\rho$ , and a set of count statistics  $\{n_k\}$  from measurements, the corresponding operators of which are  $\{E_k\}$ , determine  $\rho$ .

In the context of Bayesian statistics, priors are distributions of quantum states and models define the Hilbert space dimension and the Born rule as a likelihood function (and perhaps additional complications associated with drift parameters and measurement errors). The tomography module implements these details and has built-in support for common specifications.

The tomography module was developed concurrently with new results on Bayesian priors in [\[GCC16\]](#). Please see the paper for more detailed discussions of these more advanced topics.

#### QuTiP

Note that the Tomography module requires [QuTiP](#) which must be installed separately. Rather than reimplementing common operations on quantum states, we make use of QuTiP [Quantum objects](#). For many simple use cases the QuTiP dependency is not exposed, but familiarity with [Quantum objects](#) would be required to implement new distributions, models or heuristics.

### 2.7.2 Bases

Bases define the map from abstract quantum theory to concrete representations. Once a basis is chosen, the tomography problem becomes a special case of a generic parameter estimation problem.

The tomography module is used in the same way as other but requires the specification of a basis via the `TomographyBasis` class. QInfer comes with the following *Built-in bases*: the [Gell-Mann basis](#), the [Pauli basis](#) and function to combine bases with the tensor product. Thus, the first step in using the tomography module is to define a basis. For example, here we define the 1-qubit Pauli basis:

```
>>> from qinfer.tomography import pauli_basis
>>> basis = pauli_basis(1)
>>> print(basis)
<TomographyBasis pauli_basis dims=[2] at ...>
```

User defined bases must be orthogonal Hermitian operators and have a 0'th component of  $I/\sqrt{d}$ , where  $d$  is the dimension of the quantum system and  $I$  is the identity operator. This implies the remaining operators are traceless.

### 2.7.3 Built-in Distributions

QInfer comes with several built-in distributions listed in *Specific Distributions*. Each of these is a subclass of *DensityOperatorDistribution*. Distributions of quantum channels can also be subclassed as such with appeal to the Choi-Jamiołkowski isomorphism.

For density matrices, the *GinibreDistribution* defines a prior over mixed quantum which allows for support also for states of fixed rank [OSZ10]. For example, we can draw a sample from the this prior as follows:

```
>>> from qinfer.tomography import GinibreDistribution
>>> prior = GinibreDistribution(basis)
>>> print(prior.sample())
[[ 0.70710678 -0.17816233  0.45195168 -0.08341437]]
```

Recall this is this representation of of a qubit in the Pauli basis defined above. Quantum states are in general high dimensional objects which makes visualizing distributions of them challenging. The only 2-dimensional example is that of a rebit, which is usually defined as a qubit in the Pauli (or Bloch) representation with one of the Pauli expectations constrained to zero (usually  $\text{Tr}(\rho\sigma_y) = 0$ ).

Here we create a distribution of rebits accord to the Ginibre ensemble and use `plot_rebit_prior()` to depict this distribution through (by default) 2000 random samples. While discussing models below, we will see how to depict the particles of an *SMCUpdater* directly.

```
basis = tomography.bases.pauli_basis(1)
prior = tomography.distributions.GinibreDistribution(basis)
tomography.plot_rebit_prior(prior, rebit_axes=[1, 3])
plt.show()
```

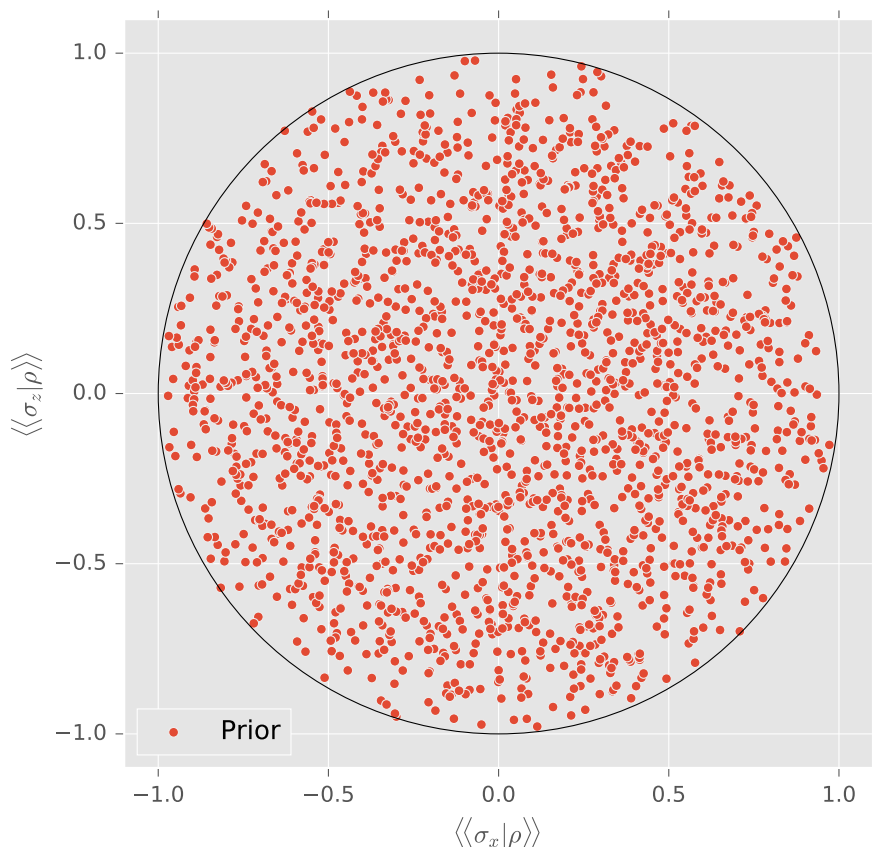



## 2.7.4 Using TomographyModel

The core of the tomography module is the *TomographyModel*. The key assumption in the current version is that of two-outcome measurements. This has the convenience of allowing experiments to be specified by a single vectorized positive operator:

```
>>> from qinfer.tomography import TomographyModel
>>> model = TomographyModel(basis)
>>> print(model.expparams_dtype)
[('meas', <type 'float'>, 4)]
```

Suppose we measure  $\sigma_z$  on a random state. The measurement effects are  $\frac{1}{2}(I \pm \sigma_z)$ . Since they sum to identity, we need only specify one of them. We can use *TomographyModel* to calculate the Born rule probability of obtaining one of these outcomes as follows:

```
>>> expparams = np.zeros((1,), dtype=model.expparams_dtype)
>>> expparams['meas'][0, :] = basis.state_to_modelparams(np.sqrt(2)*(basis[0]+basis[1])/2)
>>> print(model.likelihood(0, prior.sample(), expparams))
[[[ 0.62219803]]]
```

## 2.7.5 Built-in Heuristics

In addition to analyzing given data sets, the tomography module is well suited for testing measurement strategies against standard heuristics. These built-in heuristics are listed at *Abstract Heuristics*. For qubits, the most commonly used heuristic is the random sampling of Pauli basis measurements, which is implemented by *RandomPauliHeuristic*.

```
>>> from qinfer.tomography import RandomPauliHeuristic
>>> from qinfer import SMCUpdater
>>> updater = SMCUpdater(model, 100, prior)
>>> heuristic = RandomPauliHeuristic(updater)
>>> print(model.simulate_experiment(prior.sample(), heuristic()))
0
```

## 2.8 Learning Time-Dependent Models

### 2.8.1 Time-Dependent Parameters

In addition to learning static parameters, **QInfer** can be used to learn the values of parameters that change stochastically as a function of time. In this case, the model parameter vector  $\mathbf{x}$  is interpreted as a time-dependent vector  $\mathbf{x}(t)$  representing the state of an underlying process. The resulting statistical problem is often referred to as *state-space estimation*. By using an appropriate resampling algorithm, such as the Liu-West algorithm [LW01], state-space and static parameter estimation can be combined such that a subset of the components of  $\mathbf{x}$  are allowed to vary with time.

**QInfer** represents state-space filtering by the use of the *Simulatable.update\_timestep()* method, which samples how a model parameter vector is updated as a function of time. In particular, this method is used by *SMCUpdater* to draw samples from the distribution  $f$

$$\mathbf{x}(t_{\ell+1}) \sim f(\mathbf{x}(t_{\ell}), e(t_{\ell})),$$

where  $t_{\ell}$  is the time at which the experiment  $e_{\ell}$  is measured, and where  $t_{\ell+1}$  is the time step immediately following  $t_{\ell}$ . As this distribution is in general dependent on the experiment being performed, *update\_timestep()* is vectorized in a manner similar to *likelihood()* (see *Designing and Using Models* for details). That is, given a tensor  $X_{i,j}$  of model parameter vectors and a vector  $e_k$  of experiments, *update\_timestep()* returns a tensor  $X'_{i,j,k}$  of sampled model parameters at the next time step.

## 2.8.2 Random Walk Models

As an example, `RandomWalkModel` implements `update_timestep()` by taking as an input a *Distribution* specifying steps  $\Delta x = x(t + \delta t) - x(t)$ . An instance of `RandomWalkModel` decorates another model in a similar fashion to *other derived models*. For instance, the following code declares a precession model in which the unknown frequency  $\omega$  changes by a normal random variable with mean 0 and standard deviation 0.005 after each measurement.

```
>>> from qinfer import (
...     SimplePrecessionModel, RandomWalkModel, NormalDistribution
... )
>>> model = RandomWalkModel(
...     underlying_model=SimplePrecessionModel(),
...     step_distribution=NormalDistribution(0, 0.005 ** 2)
... )
```

We can then draw simulated trajectories for the true and estimated value of  $\omega$  using a minor modification to the updater loop discussed in *Sequential Monte Carlo*.

```
model = RandomWalkModel(
    # Note that we set a minimum frequency of negative
    # infinity to prevent problems if the random walk
    # causes omega to cross zero.
    underlying_model=SimplePrecessionModel(min_freq=-np.inf),
    step_distribution=NormalDistribution(0, 0.005 ** 2)
)
prior = UniformDistribution([0, 1])
updater = SMCUpdater(model, 2000, prior)

expparams = np.empty((1, ), dtype=model.expparams_dtype)

true_trajectory = []
est_trajectory = []

true_params = prior.sample()

for idx_exp in range(400):
    # We don't want to grow the evolution time to be arbitrarily
    # large, so we'll instead choose a random time up to some
    # maximum.
    expparams[0] = np.random.random() * 10 * np.pi
    datum = model.simulate_experiment(true_params, expparams)
    updater.update(datum, expparams)

    # We index by[:, :, 0] to pull off the index corresponding
    # to experiment parameters.
    true_params = model.update_timestep(true_params, expparams[:, :, 0])

    true_trajectory.append(true_params[0])
    est_trajectory.append(updater.est_mean())

plt.plot(true_trajectory, label='True')
plt.plot(est_trajectory, label='Est.')
plt.legend()
plt.xlabel('# of Measurements')
plt.ylabel(r'$\omega$')

plt.show()
```

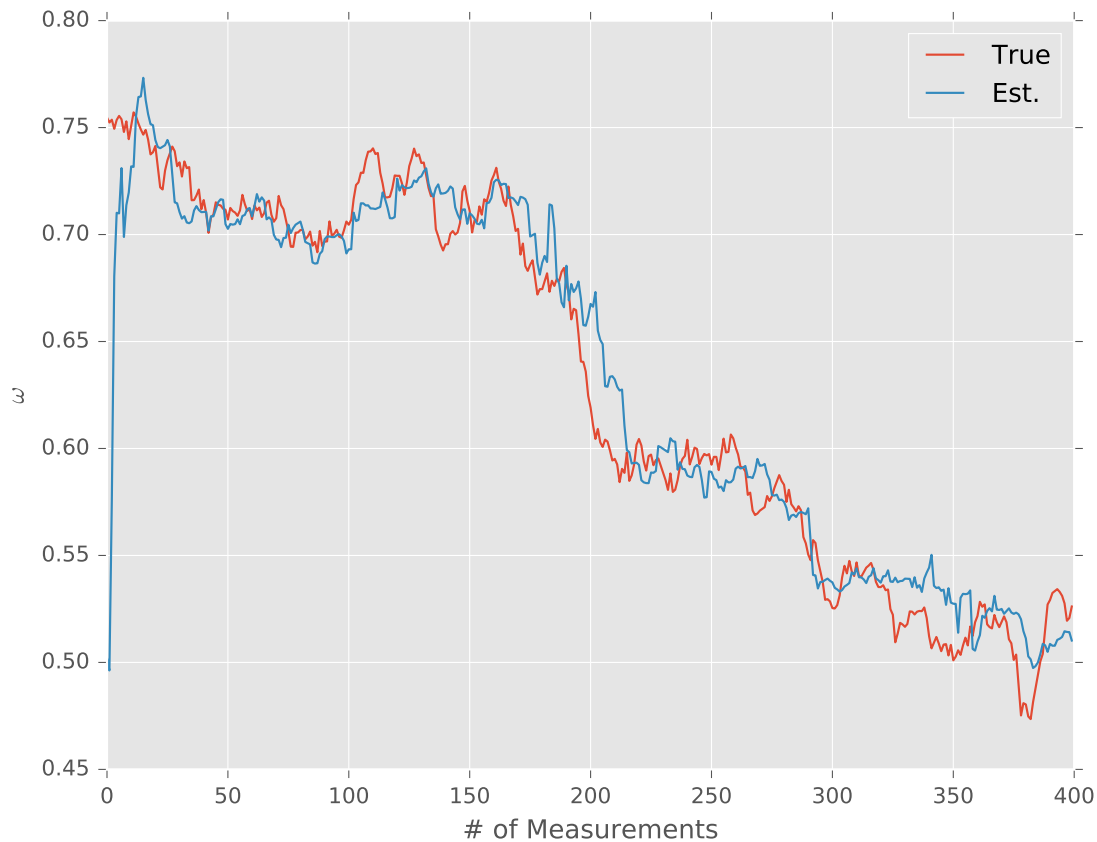

### 2.8.3 Specifying Custom Time-Step Updates

The `RandomWalkModel` example above is somewhat unrealistic, however, in that the step distribution is independent of the evolution time. For a more reasonable noise process, we would expect that  $\mathbb{V}[\omega(t + \Delta t) - \omega(t)] \propto \Delta t$ . We can subclass `SimplePrecessionModel` to add this behavior with a custom `update_timestep()` implementation.

```
class DiffusivePrecessionModel(SimplePrecessionModel):
    diffusion_rate = 0.0005 # We'll multiply this by
                            # sqrt(time) below.

    def update_timestep(self, modelparams, expparams):
        step_std_dev = self.diffusion_rate * np.sqrt(expparams)
        steps = step_std_dev * np.random.randn(
            # We want the shape of the steps in omega
            # to match the input model parameter and experiment
            # parameter shapes.
            # The axis of length 1 represents that this model
            # has only one model parameter (omega).
            modelparams.shape[0], 1, expparams.shape[0]
        )
        # Finally, we add a new axis to the input model parameters
        # to match the experiment parameters.
        return modelparams[:, :, np.newaxis] + steps
```

```

model = DiffusivePrecessionModel()
prior = UniformDistribution([0, 1])
updater = SMCUpdater(model, 2000, prior)

expparams = np.empty((1, ), dtype=model.expparams_dtype)

true_trajectory = []
est_trajectory = []

true_params = prior.sample()

for idx_exp in range(400):
    expparams[0] = np.random.random() * 10 * np.pi
    datum = model.simulate_experiment(true_params, expparams)
    updater.update(datum, expparams)

    true_params = model.update_timestep(true_params, expparams)[: , :, 0]

    true_trajectory.append(true_params[0])
    est_trajectory.append(updater.est_mean())

plt.plot(true_trajectory, label='True')
plt.plot(est_trajectory, label='Est.')
plt.legend()
plt.xlabel('# of Measurements')
plt.ylabel(r'$\omega$')

plt.show()

```

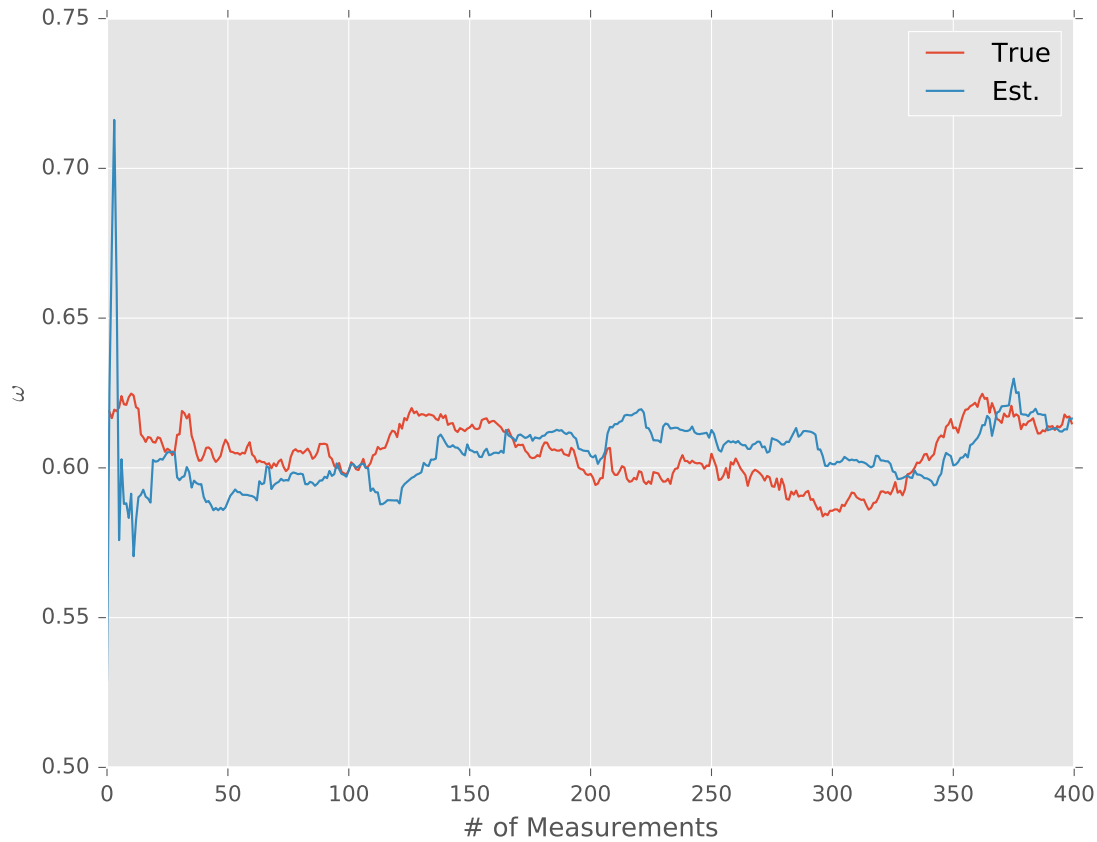

## 2.9 Performance and Robustness Testing

### 2.9.1 Introduction

In developing statistical inference applications, it is essential to test the robustness of one's software to errors and noise of various kinds. Thus, QInfer provides tools to do so by repeatedly running estimation tasks to measure performance, and by corrupting likelihood calculations in various realistic ways.

### 2.9.2 Testing Estimation Performance

Given an estimator, a common question of interest is what *risk* that estimator incurs; that is, what is the expected error of the estimates reported by the estimator? This is formalized by defining the *loss*  $L(\hat{x}, x)$  of an estimate  $\hat{x}$  given a true value  $x$ . In QInfer, we adopt the quadratic loss  $L_Q$  as a default, defined as

$$L_Q(\hat{x}, x) = \text{Tr}((\hat{x} - x)^T Q (\hat{x} - x)),$$

where  $Q$  is a positive-semidefinite matrix that establishes the relative scale of each model parameter.

We can now define the risk for an estimator as

$$R(\hat{x}(\cdot), x) = \mathbb{E}_{\text{data}} [L_Q(\hat{x}(\text{data}, x))].$$

As the risk is defined by an expectation value, we can estimate it by again Monte Carlo sampling over *trials*. That is, for a given true model  $x$ , we can draw many different data sets and then find the corresponding estimate for each in order to determine the risk.

Similarly, the Bayes risk  $r(\hat{x}(\cdot), \pi)$  is defined by also taking the expectation over a prior distribution  $\pi$ ,

$$r(\hat{x}(\cdot), \pi) = \mathbb{E}_{x \sim \pi}[R(\hat{x}(\cdot), x)].$$

The Bayes risk can thus be estimated by drawing a new set of true model parameters with each trial. **QInfer** implements risk and Bayes risk estimation by providing a function `perf_test()` which simulates a single trial with a given model, an experiment design heuristic, and either a true model parameter vector or a prior distribution. The `perf_test_multiple()` function then collects the results of `perf_test()` for many trials, reporting an array of performance metrics that can be used to quickly compute the risk and Bayes risk.

For example, we can use performance testing to evaluate the Bayes risk as a function of the number of particles used in order to determine quality parameters in experimental practice. Consider the simple precession model (`SimplePrecessionModel`) under an exponentially sparse sampling heuristic (`ExpSparseHeuristic`). Then, we can test the performance of estimating the precession frequency for several different values of `n_particles`:

```
model = SimplePrecessionModel()
prior = UniformDistribution([0, 1])
heuristic_class = ExpSparseHeuristic

for n_particles in [100, 200, 400]:
    perf = perf_test_multiple(
        n_trials=50,
        model=model, n_particles=n_particles, prior=prior,
        n_exp=50, heuristic_class=heuristic_class
    )
    # The array returned by perf_test_multiple has
    # shape (n_trials, n_exp), so to take the mean over
    # trials (Bayes risk), we need to average over the
    # zeroth axis.
    bayes_risk = perf['loss'].mean(axis=0)

    plt.semilogy(bayes_risk, label='{} particles'.format(n_particles))

plt.xlabel('# of Measurements')
plt.ylabel('Bayes Risk')
plt.legend()
plt.show()
```

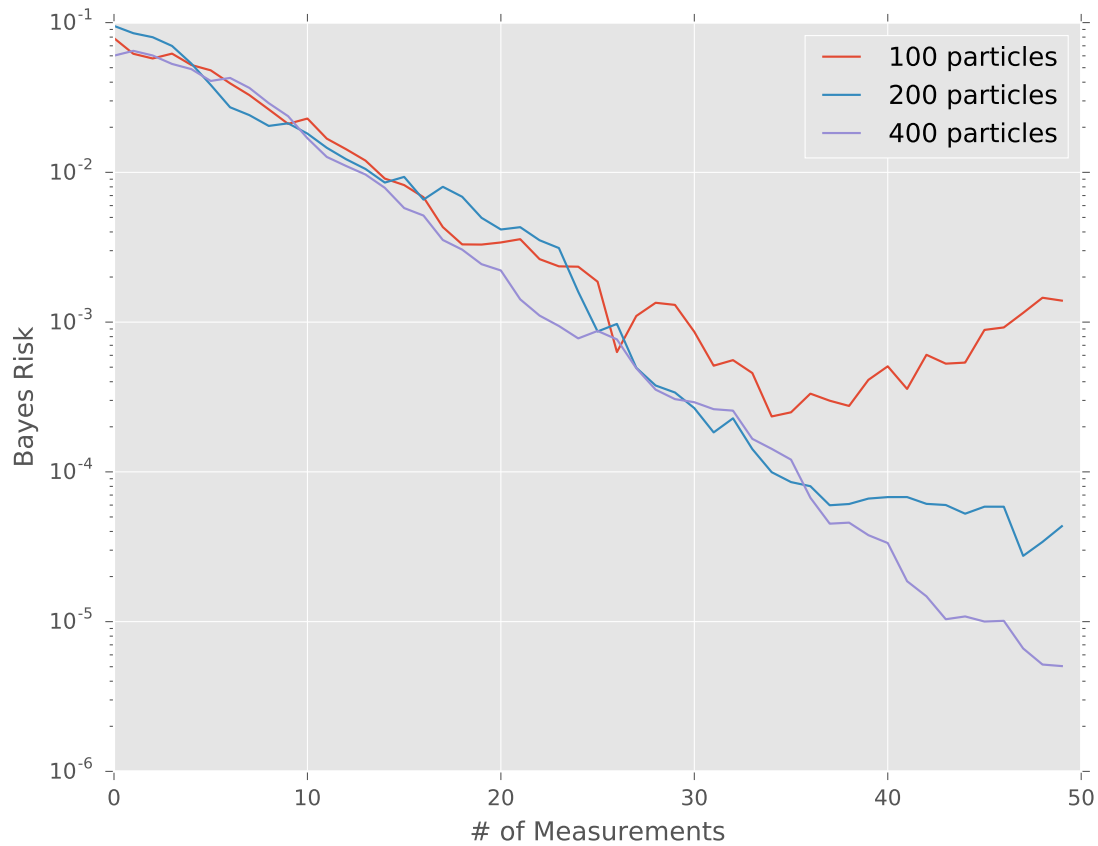

We can also pass fixed model parameter vectors to evaluate the risk (that is, not the Bayes risk) as a function of the true model:

```
model = SimplePrecessionModel()
prior = UniformDistribution([0, 1])
heuristic_class = ExpSparseHeuristic
n_exp = 50

omegas = np.linspace(0.1, 0.9, 6)
risks = np.empty_like(omegas)

for idx_omega, omega in enumerate(omegas[:, np.newaxis]):
    perf = perf_test_multiple(
        n_trials=100,
        model=model, n_particles=400, prior=prior,
        n_exp=n_exp, heuristic_class=heuristic_class,
        true_mps=omega
    )
    # We now only take the loss after the last
    # measurement (indexed by -1 along axis 1).
    risks[idx_omega] = perf['loss'][:, -1].mean(axis=0)

plt.semilogy(omegas, risks)

plt.xlabel(r'$\omega$')
plt.ylabel('Risk')
```

```
plt.show()
```

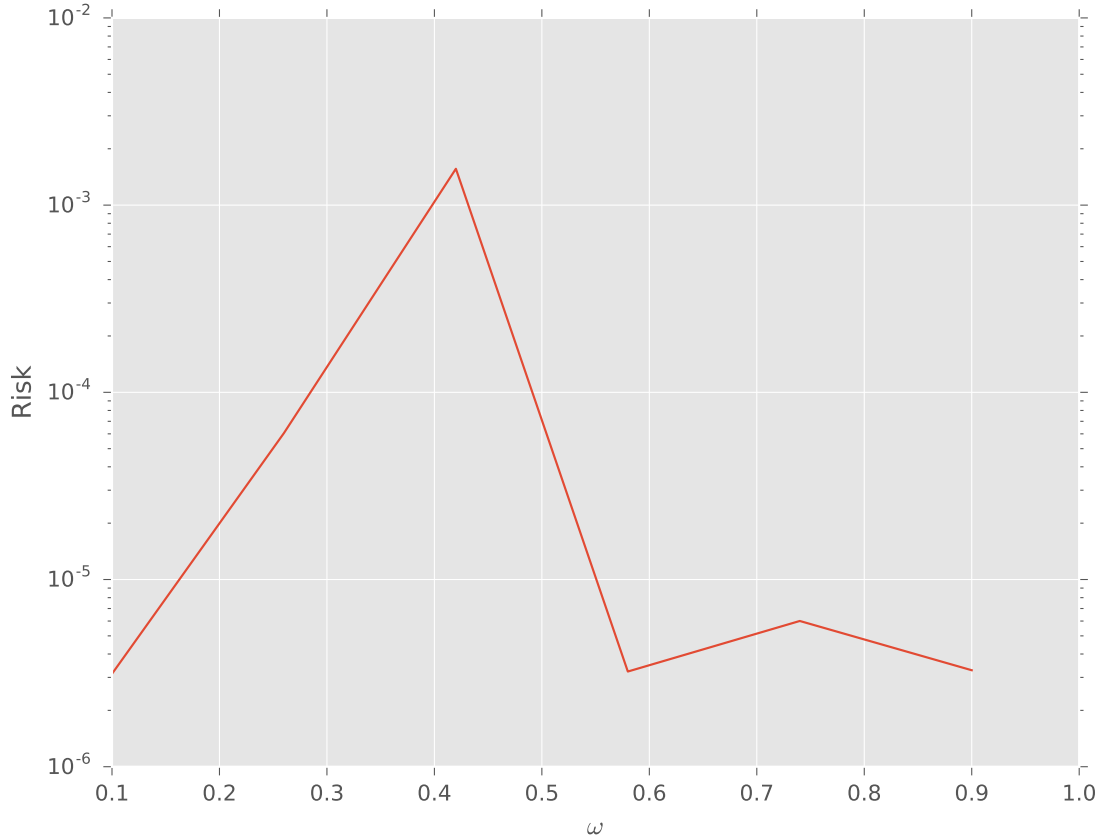

## 2.9.3 Robustness Testing

### Incorrect Priors and Models

The `perf_test()` and `perf_test_multiple()` functions also allow for testing the effect of “bad” prior assumptions, and of using the “wrong” model for estimation. In particular, the `true_prior` and `true_model` arguments allow for testing the effect of using a different prior or model for performing estimation than for simulating data.

### Modeling Faulty or Noisy Simulators

In addition, **QInfer** allows for testing robustness against errors in the model itself by using `PoisonedModel`. This `derived_model` adds noise to a model’s `likelihood()` method in such a way as to simulate sampling errors incurred in likelihood-free parameter estimation (LFPE) approaches [FG13]. The noise that `PoisonedModel` adds can be specified as the tolerance of an adaptive likelihood estimation (ALE) step [FG13], or as the number of samples and hedging used for a hedged maximum likelihood estimator of the likelihood [FB12]. In either case, the requested noise is added to the likelihood reported by the underlying model, such that

$$\widehat{\Pr}(d|\mathbf{x}; \mathbf{e}) = \Pr(d|\mathbf{x}; \mathbf{e}) + \epsilon,$$

where  $\widehat{\Pr}$  is the reported estimate of the true likelihood.



For example, to simulate using adaptive likelihood estimation to reach a threshold tolerance of 0.01:

```
>>> from qinfer import SimplePrecessionModel, PoisonedModel
>>> model = PoisonedModel(SimplePrecessionModel(), tol=0.01)
```

We can then use `perf_test_multiple()` as above to quickly test the effect of noise in the likelihood function on the Bayes risk.

```
models = [
    SimplePrecessionModel(),
    PoisonedModel(SimplePrecessionModel(), tol=0.25)
]
prior = UniformDistribution([0, 1])
heuristic_class = ExpSparseHeuristic

for model in models:
    perf = perf_test_multiple(
        n_trials=50,
        model=model, n_particles=400, prior=prior,
        true_model=models[0],
        n_exp=50, heuristic_class=heuristic_class
    )
    bayes_risk = perf['loss'].mean(axis=0)

    plt.semilogy(bayes_risk, label=type(model).__name__)

plt.xlabel('# of Measurements')
plt.ylabel('Bayes Risk')
plt.legend()
plt.show()
```

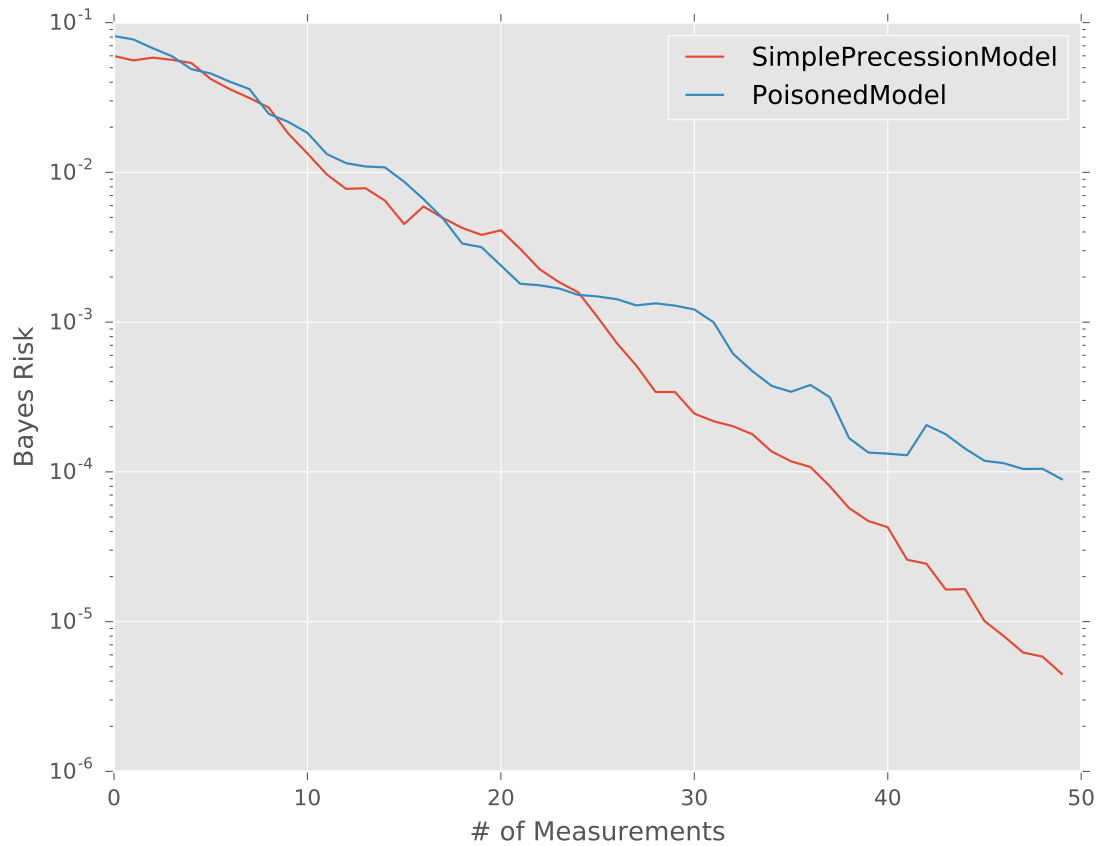

## 2.10 Parallel Execution of Models

### 2.10.1 Introduction

**QInfer** provides tools to expedite simulation by distributing computation across multiple nodes using standard parallelization tools.

### 2.10.2 Distributed Computation with IPython

The `ipyparallel` package (previously `IPython.parallel`) provides facilities for parallelizing computation across multiple cores and/or nodes. `ipyparallel` separates computation into a *controller* that is responsible for one or more *engines*, and a *client* that sends commands to these engines via the controller. **QInfer** can use a client to send likelihood evaluation calls to engines, via the `DirectViewParallelizedModel` class.

This class takes a `DirectView` onto one or more engines, typically obtained with an expression similar to `client[:]`, and splits calls to `likelihood()` across the engines accessible from the `DirectView`.

**Note:** **QInfer** does not include `ipyparallel` in its installation, so you must `install` it separately. To run the example code also requires some initialization, which is also described in the [docs](#).

```
>>> from ipyparallel import Client
>>> from qinfer import SimplePrecessionModel
>>> from qinfer import DirectViewParallelizedModel
>>> c = Client()
>>> serial_model = SimplePrecessionModel()
>>> parallel_model = DirectViewParallelizedModel(serial_model, c[:])
```

The newly decorated model will now distribute likelihood calls, such that each engine computes the likelihood for an equal number of particles. As a consequence, information shared per-experiment or per-outcome is local to each engine, and is not distributed. Therefore, this approach works best at quickly parallelizing where the per-model cost is significantly larger than the per-experiment or per-outcome cost.

---

**Note:** The `DirectViewParallelizedModel` assumes that it has ownership over engines, such that the behavior is unpredictable if any further commands are sent to the engines from outside the class.

---

## Distributed Performance Testing

As an alternative to distributing a single likelihood call across multiple engines, **QInfer** also supports distributed *Performance and Robustness Testing*. Under this model, each engine performs an independent trial of an estimation procedure, which is then collected by the client process. Distributed performance testing is implemented using the `perf_test_multiple()` function, with the keyword argument `apply` provided. For instance, the `ipyparallel` package offers a `LoadBalancedView` class whose `apply()` method sends tasks to engines according to their respective loads.

```
>>> lbview = client.load_balanced_view()
>>> performance = qi.perf_test_multiple(
...     100, serial_model, 6000, prior, 200, heuristic_class,
...     apply=lbview.apply
... )
```

Examples of both approaches to parallelization are provided as a [Jupyter Notebook](#).

### 2.10.3 GPGPU-based Likelihood Computation with PyOpenCL

Though **QInfer** does not yet have built-in support for GPU-based parallelization, `PyOpenCL` can be used to effectively distribute models as well. Here, the Cartesian product over outcomes, models and experiments matches closely the OpenCL concept of a *global ID*, as [this example](#) demonstrates. Once a kernel is developed in this way, `PyOpenCL` will allow for it to be used with any available OpenCL-compliant device.

Note that for sufficiently fast models, the overhead of copying data between the CPU and GPU may overwhelm any speed benefits obtained by this parallelization.

## 2.11 Interoperability

### 2.11.1 Introduction

**QInfer** can be used in conjunction with software written in scientific software platforms other than Python, thanks to the ready availability of interoperability libraries for interacting with Python. In this section, we provide brief examples of using these libraries with **QInfer**.

### 2.11.2 MATLAB Interoperability

As of version 2016a, MATLAB includes built-in functions for calling Python-language software. In particular, these functions can be used to use **QInfer** from within MATLAB. For example, the following MATLAB snippet will generate and analyze frequency estimation data using the *Simple Estimation* functions provided by **QInfer**.

```
>> true_omega = 70.3;
>> n_shots = 400;
>>
>> ts = pi * (1:1:100) / (2 * 100);
>>
>> signal = sin(true_omega * ts / 2) .^ 2;
>> counts = binornd(n_shots, signal);
>>
>> setenv MKL_NUM_THREADS 1
>> data = py.numpy.column_stack({counts ts ...
n_shots * ones(1, size(ts, 2))});
>> est = py.qinfer.simple_est_prec(data, ...
pyargs('freq_min', 0, 'freq_max', 100));
```

Importantly, the `setenv` command is *required* to work around a bug internal to the MATLAB interpreter.

### 2.11.3 Julia Interoperability

In Julia, interoperability can be achieved using the `PyCall.jl` package, which provides macros for making Python modules available as Julia variables. To install `PyCall.jl`, use Julia's built-in package installer:

```
julia> Pkg.add("PyCall")
```

After installing `PyCall.jl`, the example above proceeds in a very similar fashion:

```
julia> true_omega = 70.3
julia> n_shots = 100
julia>
julia> ts = pi * (1:1:100) / (2 * 100)
julia>
julia> signal = sin(true_omega * ts / 2) .^ 2
julia> counts = map(p -> rand(Binomial(n_shots, p)), signal);
julia> @pyimport numpy as np
julia> @pyimport qinfer as qi
julia>
julia> data = [counts'; ts'; n_shots * ones(length(ts))]'
julia> est_mean, est_cov = qi.simple_est_prec(data, freq_min=0, freq_max=100)
```



## API REFERENCE

### 3.1 Abstract Model Classes

#### 3.1.1 Introduction

A *model* in QInfer is a class that describes the probabilities of observing data, given a particular experiment and given a particular set of model parameters. The observation probabilities may be given implicitly or explicitly, in that the class may only allow for sampling observations, rather than finding the a distribution explicitly. In the former case, a model is represented by a subclass of *Simulatable*, while in the latter, the model is represented by a subclass of *Model*.

#### 3.1.2 *Simulatable* - Base Class for Implicit (*Simulatable*) Models

##### Class Reference

**class** `qinfer.Simulatable`

Bases: `object`

Represents a system which can be simulated according to various model parameters and experimental control parameters in order to produce representative data.

See *Designing and Using Models* for more details.

**Parameters** `allow_identical_outcomes` (*bool*) – Whether the method `outcomes` should be allowed to return multiple identical outcomes for a given `expparam`. It will be more efficient to set this to `True` whenever it is likely that multiple identical outcomes will occur.

**n\_modelparams**

Returns the number of real model parameters admitted by this model.

This property is assumed by inference engines to be constant for the lifetime of a *Model* instance.

**expparams\_dtype**

Returns the dtype of an experiment parameter array. For a model with single-parameter control, this will likely be a scalar dtype, such as `"float64"`. More generally, this can be an example of a record type, such as `[('time', py.'float64'), ('axis', 'uint8')]`.

This property is assumed by inference engines to be constant for the lifetime of a *Model* instance.

**is\_n\_outcomes\_constant**

Returns `True` if and only if both the domain and `n_outcomes` are independent of the `expparam`.

This property is assumed by inference engines to be constant for the lifetime of a *Model* instance.

**model\_chain**

Returns a tuple of models upon which this model is based, such that properties and methods of underlying models for models that decorate other models can be accessed. For a standalone model, this is always the empty tuple.

**base\_model**

Returns the most basic model that this model depends on. For standalone models, this property satisfies `model.base_model is model`.

**underlying\_model**

Returns the model that this model is based on (decorates) if such a model exists, or `None` if this model is independent.

**sim\_count**

Returns the number of data samples that have been produced by this simulator.

**Return type** `int`

**Q**

Returns the diagonal of the scale matrix  $Q$  that relates the scales of each of the model parameters. In particular, the quadratic loss for this Model is defined as:

$$L_Q(x, \hat{x}) = (x - \hat{x})^T Q (x - \hat{x})$$

If a subclass does not explicitly define the scale matrix, it is taken to be the identity matrix of appropriate dimension.

**Returns** The diagonal elements of  $Q$ .

**Return type** `ndarray` of shape `(n_modelparams, )`.

**modelparam\_names**

Returns the names of the various model parameters admitted by this model, formatted as LaTeX strings.

**are\_expparam\_dtypes\_consistent** (*expparams*)

Returns `True` iff all of the given expparams correspond to outcome domains with the same dtype. For efficiency, concrete subclasses should override this method if the result is always `True`.

**Parameters** **expparams** (`np.ndarray`) – Array of expparamms of type `expparams_dtype`

**Return type** `bool`

**n\_outcomes** (*expparams*)

Returns an array of dtype `uint` describing the number of outcomes for each experiment specified by `expparams`. If the number of outcomes does not depend on `expparams` (i.e. `is_n_outcomes_constant` is `True`), this method should return a single number. If there are an infinite (or intractibly large) number of outcomes, this value specifies the number of outcomes to randomly sample.

**Parameters** **expparams** (`numpy.ndarray`) – Array of experimental parameters. This array must be of dtype agreeing with the `expparams_dtype` property.

**domain** (*expparams*)

Returns a list of *Domain* objects, one for each input expparam.

**Parameters** **expparams** (`numpy.ndarray`) – Array of experimental parameters. This array must be of dtype agreeing with the `expparams_dtype` property, or, in the case where `n_outcomes_constant` is `True`, `None` should be a valid input.

**Return type** list of *Domain*

**are\_models\_valid** (*modelparams*)

Given a shape (*n\_models*, *n\_modelparams*) array of model parameters, returns a boolean array of shape (*n\_models*) specifying whether each set of model parameters represents is valid under this model.

**simulate\_experiment** (*modelparams*, *expparams*, *repeat=1*)

Produces data according to the given model parameters and experimental parameters, structured as a NumPy array.

#### Parameters

- **modelparams** (*np.ndarray*) – A shape (*n\_models*, *n\_modelparams*) array of model parameter vectors describing the hypotheses under which data should be simulated.
- **expparams** (*np.ndarray*) – A shape (*n\_experiments*, ) array of experimental control settings, with dtype given by *expparams\_dtype*, describing the experiments whose outcomes should be simulated.
- **repeat** (*int*) – How many times the specified experiment should be repeated.

**Return type** *np.ndarray*

**Returns** A three-index tensor *data[i, j, k]*, where *i* is the repetition, *j* indexes which vector of model parameters was used, and where *k* indexes which experimental parameters were used. If *repeat == 1*, *len(modelparams) == 1* and *len(expparams) == 1*, then a scalar datum is returned instead.

**clear\_cache** ()

Tells the model to clear any internal caches used in computing likelihoods and drawing samples. Calling this method should not cause any different results, but should only affect performance.

**experiment\_cost** (*expparams*)

Given an array of experimental parameters, returns the cost associated with performing each experiment. By default, this cost is constant (one) for every experiment.

**Parameters** *expparams* (*ndarray* of dtype given by *expparams\_dtype*) – An array of experimental parameters for which the cost is to be evaluated.

**Returns** An array of costs corresponding to the specified experiments.

**Return type** *ndarray* of dtype float and of the same shape as *expparams*.

**distance** (*a*, *b*)

Gives the distance between two model parameter vectors *a* and *b*. By default, this is the vector 1-norm of the difference  $\mathbf{Q}(\mathbf{a} - \mathbf{b})$  rescaled by  $\mathbf{Q}$ .

#### Parameters

- **a** (*np.ndarray*) – Array of model parameter vectors having shape (*n\_models*, *n\_modelparams*).
- **b** (*np.ndarray*) – Array of model parameters to compare to, having the same shape as *a*.

**Returns** An array *d* of distances *d[i]* between *a[i, :]* and *b[i, :]*.

**update\_timestep** (*modelparams*, *expparams*)

Returns a set of model parameter vectors that is the update of an input set of model parameter vectors, such that the new models are conditioned on a particular experiment having been performed. By default, this is the trivial function  $\mathbf{x}(t_{k+1}) = \mathbf{x}(t_k)$ .

#### Parameters



- **modelparams** (*np.ndarray*) – Set of model parameter vectors to be updated.
- **expparams** (*np.ndarray*) – An experiment parameter array describing the experiment that was just performed.

**Return** *np.ndarray* Array of shape (n\_models, n\_modelparams, n\_experiments) describing the update of each model according to each experiment.

**canonicalize** (*modelparams*)

Returns a canonical set of model parameters corresponding to a given possibly non-canonical set. This is used for models in which there exist model parameters  $x_i$  and  $\text{vec}\{x\}_j$  such that

$$\Pr(d|x_i; e) = \Pr(d|x_j; e)$$

for all outcomes  $d$  and experiments  $e$ . For models admitting such an ambiguity, this method should then be overridden to return a consistent choice out of such vectors, hence avoiding supurious model degeneracies.

Note that, by default, `SMCUpdater` will *not* call this method.

### 3.1.3 Model - Base Class for Explicit (Likelihood) Models

If a model supports explicit calculation of the likelihood function, then this is represented by subclassing from `Model`.

#### Class Reference

**class** `qinfer.Model` (*allow\_identical\_outcomes=False, outcome\_warning\_threshold=0.99*)

Bases: `qinfer.abstract_model.Simulatable`

Represents a system which can be simulated according to various model parameters and experimental control parameters in order to produce the probability of a hypothetical data record. As opposed to `Simulatable`, instances of `Model` not only produce data consistent with the description of a system, but also evaluate the probability of that data arising from the system.

#### Parameters

- **allow\_identical\_outcomes** (*bool*) – Whether the method `representative_outcomes` should be allowed to return multiple identical outcomes for a given `expparam`.
- **outcome\_warning\_threshold** (*float*) – Threshold value below which `representative_outcomes` will issue a warning about the representative outcomes not adequately covering the domain with respect to the relevant distribution.

See *Designing and Using Models* for more details.

#### **call\_count**

Returns the number of points at which the probability of this model has been evaluated, where a point consists of a hypothesis about the model (a vector of model parameters), an experimental control setting (`expparams`) and a hypothetical or actual datum. *rtype*: int

**likelihood** (*outcomes, modelparams, expparams*)

Calculates the probability of each given outcome, conditioned on each given model parameter vector and each given experimental control setting.

#### Parameters

- **modelparams** (*np.ndarray*) – A shape (n\_models, n\_modelparams) array of model parameter vectors describing the hypotheses for which the likelihood function is to be calculated.

- **expparams** (*np.ndarray*) – A shape (*n\_experiments*, ) array of experimental control settings, with dtype given by *expparams\_dtype*, describing the experiments from which the given outcomes were drawn.

**Return type** *np.ndarray*

**Returns** A three-index tensor  $L[i, j, k]$ , where *i* is the outcome being considered, *j* indexes which vector of model parameters was used, and where *k* indexes which experimental parameters were used. Each element  $L[i, j, k]$  then corresponds to the likelihood  $\Pr(d_i | \mathbf{x}_j; e_k)$ .

**allow\_identical\_outcomes**

Whether the method *representative\_outcomes* should be allowed to return multiple identical outcomes for a given *expparam*. It will be more efficient to set this to *True* whenever it is likely that multiple identical outcomes will occur.

**Returns** Flag state.

**Return type** *bool*

**outcome\_warning\_threshold**

Threshold value below which *representative\_outcomes* will issue a warning about the representative outcomes not adequately covering the domain with respect to the relevant distribution.

**Returns** Threshold value.

**Return type** *float*

**is\_model\_valid** (*modelparams*)

Returns *True* if and only if the model parameters given are valid for this model.

### 3.1.4 FiniteOutcomeModel - Base Class for Models with a Finite Number of Outcomes

The likelihood function provided by a subclass is used to implement *Simulatable.simulate\_experiment()*, which is possible because the likelihood of all possible outcomes can be computed. This class also concretely implements the *domain* method by looking at the definition of *n\_outcomes*.

#### Class Reference

```
class qinfer.FiniteOutcomeModel (allow_identical_outcomes=False, out-
                                come_warning_threshold=0.99, n_outcomes_cutoff=None)
Bases: qinfer.abstract_model.Model
```

Represents a system in the same way that *Model*, except that it is demanded that the number of outcomes for any experiment be known and finite.

#### Parameters

- **allow\_identical\_outcomes** (*bool*) – Whether the method *representative\_outcomes* should be allowed to return multiple identical outcomes for a given *expparam*.
- **outcome\_warning\_threshold** (*float*) – Threshold value below which *representative\_outcomes* will issue a warning about the representative outcomes not adequately covering the domain with respect to the relevant distribution.

- **n\_outcomes\_cutoff** (*int*) – If `n_outcomes` exceeds this value, `representative_outcomes` will use this value in its place. This is useful in the case of a finite yet untractable number of outcomes. Use `None` for no cutoff.

See [Model](#) and [Designing and Using Models](#) for more details.

#### **n\_outcomes\_cutoff**

If `n_outcomes` exceeds this value for some `expparm`, `representative_outcomes` will use this value in its place. This is useful in the case of a finite yet untractable number of outcomes.

**Returns** Cutoff value.

**Return type** `int`

#### **domain** (*expparams*)

Returns a list of [Domain](#) objects, one for each input `expparm`.

**Parameters** **expparams** (*numpy.ndarray*) – Array of experimental parameters. This array must be of dtype agreeing with the `expparams_dtype` property, or, in the case where `n_outcomes_constant` is `True`, `None` should be a valid input.

**Return type** list of `Domain`

#### **simulate\_experiment** (*modelparams, expparams, repeat=1*)

#### **static pr0\_to\_likelihood\_array** (*outcomes, pr0*)

Assuming a two-outcome measurement with probabilities given by the array `pr0`, returns an array of the form expected to be returned by `likelihood` method.

#### **Parameters**

- **outcomes** (*numpy.ndarray*) – Array of integers indexing outcomes.
- **pr0** (*numpy.ndarray*) – Array of shape `(n_models, n_experiments)` describing the probability of obtaining outcome 0 from each set of model parameters and experiment parameters.

### 3.1.5 DifferentiableModel - Base Class for Explicit Models with Differentiable Likelihoods

#### Class Reference

**class** `qinfer.DifferentiableModel` (*allow\_identical\_outcomes=False, out-*  
*come\_warning\_threshold=0.99*)

Bases: `qinfer.abstract_model.Model`

#### **score** (*outcomes, modelparams, expparams, return\_L=False*)

Returns the score of this likelihood function, defined as:

$$q(d, \mathbf{x}; \mathbf{e}) = \nabla_{\mathbf{x}} \log \Pr(d|\mathbf{x}; \mathbf{e}).$$

Calls are represented as a four-index tensor `score[idx_modelparam, idx_outcome, idx_model, idx_experiment]`. The left-most index may be suppressed for single-parameter models.

If `return_L` is `True`, both `q` and the likelihood `L` are returned as `q, L`.

#### **fisher\_information** (*modelparams, expparams*)

Returns the covariance of the score taken over possible outcomes, known as the Fisher information.

The result is represented as the four-index tensor `fisher[idx_modelparam_i, idx_modelparam_j, idx_model, idx_experiment]`, which gives the Fisher information matrix for each model vector and each experiment vector.

---

**Note:** The default implementation of this method calls `score()` for each possible outcome, which can be quite slow. If possible, overriding this method can give significant speed advantages.

---

## 3.2 Derived Models

### 3.2.1 Introduction

QInfer provides several models which *decorate* other models, providing additional functionality or changing the behaviors of underlying models.

### 3.2.2 `PoisonedModel` - Model corrupted by likelihood errors

`class qinfer.PoisonedModel(underlying_model, tol=None, n_samples=None, hedge=None)`

Bases: `qinfer.derived_models.DerivedModel`

Model that simulates sampling error incurred by the MLE or ALE methods of reconstructing likelihoods from sample data. The true likelihood given by an underlying model is perturbed by a normally distributed random variable  $\epsilon$ , and then truncated to the interval  $[0, 1]$ .

The variance of  $\epsilon$  can be specified either as a constant, to simulate ALE (in which samples are collected until a given threshold is met), or as proportional to the variance of a possibly-hedged binomial estimator, to simulate MLE.

#### Parameters

- **`underlying_model`** (`Model`) – The “true” model to be poisoned.
- **`tol`** (`float`) – For ALE, specifies the given error tolerance to simulate.
- **`n_samples`** (`int`) – For MLE, specifies the number of samples collected.
- **`hedge`** (`float`) – For MLE, specifies the hedging used in estimating the true likelihood.

**`likelihood`** (`outcomes, modelparams, expparams`)

**`simulate_experiment`** (`modelparams, expparams, repeat=1`)

Simulates experimental data according to the original (unpoisoned) model. Note that this explicitly causes the simulated data and the likelihood function to disagree. This is, strictly speaking, a violation of the assumptions made about `Model` subclasses. This violation is by intention, and allows for testing the robustness of inference algorithms against errors in that assumption.

### 3.2.3 `BinomialModel` - Model over batches of two-outcome experiments

`class qinfer.BinomialModel(underlying_model)`

Bases: `qinfer.derived_models.DerivedModel`

Model representing finite numbers of iid samples from another model, using the binomial distribution to calculate the new likelihood function.

**Parameters** `underlying_model` (`qinfer.abstract_model.Model`) – An instance of a two- outcome model to be decorated by the binomial distribution.

Note that a new experimental parameter field `n_meas` is added by this model. This parameter field represents how many times a measurement should be made at a given set of experimental parameters. To ensure the correct operation of this model, it is important that the decorated model does not also admit a field with the name `n_meas`.

**decorated\_model**

**expparams\_dtype**

**is\_n\_outcomes\_constant**

Returns `True` if and only if the number of outcomes for each experiment is independent of the experiment being performed.

This property is assumed by inference engines to be constant for the lifetime of a `Model` instance.

**n\_outcomes** (`expparams`)

Returns an array of dtype `uint` describing the number of outcomes for each experiment specified by `expparams`.

**Parameters** `expparams` (`numpy.ndarray`) – Array of experimental parameters. This array must be of dtype agreeing with the `expparams_dtype` property.

**domain** (`expparams`)

Returns a list of “Domain”s, one for each input `expparam`.

**Parameters** `expparams` (`numpy.ndarray`) – Array of experimental parameters. This array must be of dtype agreeing with the `expparams_dtype` property, or, in the case where `n_outcomes_constant` is `True`, `None` should be a valid input.

**Return type** list of `Domain`

**are\_expparam\_dtypes\_consistent** (`expparams`)

Returns `True` iff all of the given `expparams` correspond to outcome domains with the same dtype. For efficiency, concrete subclasses should override this method if the result is always `True`.

**Parameters** `expparams` (`np.ndarray`) – Array of `expparamms` of type `expparams_dtype`

**Return type** `bool`

**likelihood** (`outcomes`, `modelparams`, `expparams`)

**simulate\_experiment** (`modelparams`, `expparams`, `repeat=1`)

**update\_timestep** (`modelparams`, `expparams`)

### 3.2.4 MultinomialModel - Model over batches of D-outcome experiments

**class** `qinfer.MultinomialModel` (`underlying_model`)

Bases: `qinfer.derived_models.DerivedModel`

Model representing finite numbers of iid samples from another model with a fixed and finite number of outcomes, using the multinomial distribution to calculate the new likelihood function.

**Parameters** `underlying_model` (`qinfer.abstract_model.FiniteOutcomeModel`) – An instance of a D-outcome model to be decorated by the multinomial distribution. This underlying model must have `is_n_outcomes_constant` as `True`.

Note that a new experimental parameter field `n_meas` is added by this model. This parameter field represents how many times a measurement should be made at a given set of experimental parameters. To ensure the correct operation of this model, it is important that the decorated model does not also admit a field with the name `n_meas`.

**decorated\_model**

**expparams\_dtype**

**is\_n\_outcomes\_constant**

Returns `True` if and only if the number of outcomes for each experiment is independent of the experiment being performed.

This property is assumed by inference engines to be constant for the lifetime of a `Model` instance.

**n\_sides**

Returns the number of possible outcomes of the underlying model.

**underlying\_domain**

Returns the *Domain* of the underlying model.

**n\_outcomes** (*expparams*)

Returns an array of dtype `uint` describing the number of outcomes for each experiment specified by *expparams*.

**Parameters** *expparams* (*numpy.ndarray*) – Array of experimental parameters. This array must be of dtype agreeing with the `expparams_dtype` property.

**domain** (*expparams*)

Returns a list of *Domain* objects, one for each input *expparam*. :param *numpy.ndarray expparams*: Array of experimental parameters. This

array must be of dtype agreeing with the `expparams_dtype` property.

**Return type** list of *Domain*

**are\_expparam\_dtypes\_consistent** (*expparams*)

Returns `True` iff all of the given *expparams* correspond to outcome domains with the same dtype. For efficiency, concrete subclasses should override this method if the result is always `True`.

**Parameters** *expparams* (*np.ndarray*) – Array of *expparams* of type *expparams\_dtype*

**Return type** `bool`

**likelihood** (*outcomes*, *modelparams*, *expparams*)

**simulate\_experiment** (*modelparams*, *expparams*, *repeat=1*)

### 3.2.5 MLEModel - Model for approximating maximum-likelihood estimation

**class** `qinfer.MLEModel` (*underlying\_model*, *likelihood\_power*)

Bases: `qinfer.derived_models.DerivedModel`

Uses the method of [JDD08] to approximate the maximum likelihood estimator as the mean of a fictional posterior formed by amplifying the Bayes update by a given power  $\gamma$ . As  $\gamma \rightarrow \infty$ , this approximation to the MLE improves, but at the cost of numerical stability.

**Parameters** *likelihood\_power* (*float*) – Power to which the likelihood calls should be raised in order to amplify the Bayes update.

**simulate\_experiment** (*modelparams*, *expparams*, *repeat=1*)

`likelihood(outcomes, modelparams, expparams)`

## 3.3 Probability Distributions

### 3.3.1 Distribution - Abstract Base Class for Probability Distributions

`class qinfer.Distribution`

Bases: `object`

Abstract base class for probability distributions on one or more random variables.

**n\_rvs**

The number of random variables that this distribution is over.

Type `int`

**sample** (*n=1*)

Returns one or more samples from this probability distribution.

**Parameters** *n* (`int`) – Number of samples to return.

**Return type** `numpy.ndarray`

**Returns** An array containing samples from the distribution of shape `(n, d)`, where `d` is the number of random variables.

### 3.3.2 Specific Distributions

`class qinfer.UniformDistribution(ranges=array([[0, 1]]))`

Bases: `qinfer.distributions.Distribution`

Uniform distribution on a given rectangular region.

**Parameters** *ranges* (`numpy.ndarray`) – Array of shape `(n_rvs, 2)`, where `n_rvs` is the number of random variables, specifying the upper and lower limits for each variable.

**n\_rvs**

**sample** (*n=1*)

**grad\_log\_pdf** (*var*)

`class qinfer.NormalDistribution(mean, var, trunc=None)`

Bases: `qinfer.distributions.Distribution`

Normal or truncated normal distribution over a single random variable.

**Parameters**

- **mean** (`float`) – Mean of the represented random variable.
- **var** (`float`) – Variance of the represented random variable.
- **trunc** (`tuple`) – Limits at which the PDF of this distribution should be truncated, or `None` if the distribution is to have infinite support.

**n\_rvs**

**sample** (*n=1*)

**grad\_log\_pdf** (*x*)

```
class qinfer.MultivariateNormalDistribution(mean, cov)
```

Bases: qinfer.distributions.Distribution

Multivariate (vector-valued) normal distribution.

#### Parameters

- **mean** (*np.ndarray*) – Array of shape  $(n\_rvs, )$  representing the mean of the distribution.
- **cov** (*np.ndarray*) – Array of shape  $(n\_rvs, n\_rvs)$  representing the covariance matrix of the distribution.

**n\_rvs**

**sample** ( $n=1$ )

**grad\_log\_pdf** ( $x$ )

```
class qinfer.SlantedNormalDistribution(ranges=array([[0, 1]]), weight=0.01)
```

Bases: qinfer.distributions.Distribution

Uniform distribution on a given rectangular region.

**Parameters** **ranges** (*numpy.ndarray*) – Array of shape  $(n\_rvs, 2)$ , where  $n\_rvs$  is the number of random variables, specifying the upper and lower limits for each variable.

**n\_rvs**

**sample** ( $n=1$ )

```
class qinfer.LogNormalDistribution(mu=0, sigma=1)
```

Bases: qinfer.distributions.Distribution

Log-normal distribution.

#### Parameters

- **mu** – Location parameter (numeric), set to 0 by default.
- **sigma** – Scale parameter (numeric), set to 1 by default. Must be strictly greater than zero.

**n\_rvs**

**sample** ( $n=1$ )

```
class qinfer.ConstantDistribution(values)
```

Bases: qinfer.distributions.Distribution

Represents a deterministic variable; useful for combining with other distributions, marginalizing, etc.

**Parameters** **values** – Shape  $(n, )$  array or list of values  $X_0$  such that  $\Pr(X) = \delta(X - X_0)$ .

**n\_rvs**

**sample** ( $n=1$ )

```
class qinfer.BetaDistribution(alpha=None, beta=None, mean=None, var=None)
```

Bases: qinfer.distributions.Distribution

The beta distribution, whose pdf at  $x$  is proportional to  $x^{\alpha-1}(1-x)^{\beta-1}$ . Note that either  $\alpha$  and  $\beta$ , or  $\text{mean}$  and  $\text{var}$ , must be specified as inputs; either case uniquely determines the distribution.

#### Parameters

- **alpha** (*float*) – The alpha shape parameter of the beta distribution.
- **beta** (*float*) – The beta shape parameter of the beta distribution.



- **mean** (*float*) – The desired mean value of the beta distribution.
- **var** (*float*) – The desired variance of the beta distribution.

**n\_rvs**

**sample** (*n=1*)

**class** `qinfer.BetaBinomialDistribution` (*n, alpha=None, beta=None, mean=None, var=None*)  
 Bases: `qinfer.distributions.Distribution`

The beta-binomial distribution, whose pmf at the non-negative integer  $k$  is equal to  $\binom{n}{k} \frac{B(k+\alpha, n-k+\beta)}{B(\alpha, \beta)}$  with  $B(\cdot, \cdot)$  the beta function. This is the compound distribution whose variates are binomial distributed with a bias chosen from a beta distribution. Note that either `alpha` and `beta`, or `mean` and `var`, must be specified as inputs; either case uniquely determines the distribution.

#### Parameters

- **n** (*int*) – The  $n$  parameter of the beta-binomial distribution.
- **alpha** (*float*) – The alpha shape parameter of the beta-binomial distribution.
- **beta** (*float*) – The beta shape parameter of the beta-binomial distribution.
- **mean** (*float*) – The desired mean value of the beta-binomial distribution.
- **var** (*float*) – The desired variance of the beta-binomial distribution.

**n\_rvs**

**sample** (*n=1*)

**class** `qinfer.GammaDistribution` (*alpha=None, beta=None, mean=None, var=None*)  
 Bases: `qinfer.distributions.Distribution`

The gamma distribution, whose pdf at  $x$  is proportional to  $x^{-\alpha-1}e^{-x\beta}$ . Note that either `alpha` and `beta`, or `mean` and `var`, must be specified as inputs; either case uniquely determines the distribution.

#### Parameters

- **alpha** (*float*) – The alpha shape parameter of the gamma distribution.
- **beta** (*float*) – The beta shape parameter of the gamma distribution.
- **mean** (*float*) – The desired mean value of the gamma distribution.
- **var** (*float*) – The desired variance of the gamma distribution.

**n\_rvs**

**sample** (*n=1*)

**class** `qinfer.HilbertSchmidtUniform` (*dim=2*)  
 Bases: `qinfer.distributions.SingleSampleMixin`, `qinfer.distributions.Distribution`

Creates a new Hilber-Schmidt uniform prior on state space of dimension `dim`. See e.g. [Mez06] and [Mis12].

**Parameters** **dim** (*int*) – Dimension of the state space.

**n\_rvs**

**sample** ()

**make\_Paulis** (*paulis, d*)

**class** `qinfer.HaarUniform` (*dim=2*)  
 Bases: `qinfer.distributions.SingleSampleMixin`, `qinfer.distributions.Distribution`

Creates a new Haar uniform prior on state space of dimension `dim`.

**Parameters** `dim (int)` – Dimension of the state space.

`n_rvs`

`sample ()`

**class** `qinfer.GinibreUniform (dim=2, k=2)`

Bases: `qinfer.distributions.SingleSampleMixin`, `qinfer.distributions.Distribution`

Creates a prior on state space of dimension `dim` according to the Ginibre ensemble with parameter `k`. See e.g. [\[Mis12\]](#).

**Parameters** `dim (int)` – Dimension of the state space.

`n_rvs`

`sample ()`

### 3.3.3 Combining Distributions

QInfer also offers classes for combining distributions together to produce new ones.

**class** `qinfer.ProductDistribution (*factors)`

Bases: `qinfer.distributions.Distribution`

Takes a non-zero number of QInfer distributions  $D_k$  as input and returns their Cartesian product.

In other words, the returned distribution is  $\Pr(D_1, \dots, D_N) = \prod_k \Pr(D_k)$ .

**Parameters** `factors (Distribution)` – Distribution objects representing  $D_k$ . Alternatively, one iterable argument can be given, in which case the factors are the values drawn from that iterator.

`n_rvs`

`sample (n=1)`

**class** `qinfer.PostselectedDistribution (distribution, model, maxiters=100)`

Bases: `qinfer.distributions.Distribution`

Postselects a distribution based on validity within a given model.

`n_rvs`

`sample (n=1)`

Returns one or more samples from this probability distribution.

**Parameters** `n (int)` – Number of samples to return.

**Return** `numpy.ndarray` An array containing samples from the distribution of shape  $(n, d)$ , where  $d$  is the number of random variables.

`grad_log_pdf (x)`

**class** `qinfer.MixtureDistribution (weights, dist, dist_args=None, dist_kw_args=None, shuffle=True)`

Bases: `qinfer.distributions.Distribution`

Samples from a weighted list of distributions.

**Parameters**

- **weights** – Length `n_dist` list or `np.ndarray` of probabilities summing to 1.

- **dist** – Either a length `n_dist` list of `Distribution` instances, or a `Distribution` class, for example, `NormalDistribution`. It is assumed that a list of `Distribution`'s all have the same `n_rvs`.
- **dist\_args** – If `dist` is a class, an array of shape `(n_dist, n_rvs)` where `dist_args[k, :]` defines the arguments of the `k`'th distribution. Use `None` if the distribution has no arguments.
- **dist\_kw\_args** – If `dist` is a class, a dictionary where each key's value is an array of shape `(n_dist, n_rvs)` where `dist_kw_args[key][k, :]` defines the keyword argument corresponding to `key` of the `k`'th distribution. Use `None` if the distribution needs no keyword arguments.
- **shuffle** (*bool*) – Whether or not to shuffle result after sampling. Not shuffling will result in variates being in the same order as the distributions. Default is `True`.

**n\_rvs**

**n\_dist**

The number of distributions in the mixture distribution.

**sample** (*n=1*)

### 3.3.4 Mixins for Distribution Development

```
class qinfer.SingleSampleMixin
```

Bases: `object`

Mixin class that extends a class so as to generate multiple samples correctly, given a method `_sample` that generates one sample at a time.

**sample** (*n=1*)

## 3.4 Domains

### 3.4.1 Introduction

A *Domain* represents a collection of objects. They are used by *Simulatable* (and subclasses like *Model* and *FiniteOutcomeModel*) to store relevant information about the possible outcomes of a given experiment. This includes properties like whether or not there are a finite number of possibilities, if so how many, and what their data types are.

### 3.4.2 Domain - Base Class for Domains

All domains should inherit from this base class.

#### Class Reference

```
class qinfer.Domain
```

Bases: `object`

Abstract base class for domains of outcomes of models.

**is\_continuous**

Whether or not the domain has an uncountable number of values.

**Type** `bool`

**is\_finite**

Whether or not the domain contains a finite number of points.

**Type** `bool`

**dtype**

The numpy dtype of a single element of the domain.

**Type** `np.dtype`

**n\_members**

Returns the number of members in the domain if it *is\_finite*, otherwise, returns *None*.

**Type** `int`

**example\_point**

Returns any single point guaranteed to be in the domain, but no other guarantees; useful for testing purposes. This is given as a size 1 `np.array` of type *dtype*.

**Type** `np.ndarray`

**values**

Returns an `np.array` of type *dtype* containing some values from the domain. For domains where *is\_finite* is *True*, all elements of the domain will be yielded exactly once.

**Return type** `np.ndarray`

**is\_discrete**

Whether or not the domain has a countable number of values.

**Type** `bool`

**in\_domain** (*points*)

Returns *True* if all of the given points are in the domain, *False* otherwise.

**Parameters** **points** (`np.ndarray`) – An `np.ndarray` of type `self.dtype`.

**Return type** `bool`

### 3.4.3 RealDomain - (A subset of) Real Numbers

#### Class Reference

**class** `qinfer.RealDomain` (*min=None, max=None*)

Bases: `qinfer.domains.Domain`

A domain specifying a contiguous (and possibly open ended) subset of the real numbers.

**Parameters**

- **min** (*float*) – A number specifying the lowest possible value of the domain. If left as *None*, negative infinity is assumed.
- **max** (*float*) – A number specifying the largest possible value of the domain. If left as *None*, positive infinity is assumed.

**min**

Returns the minimum value of the domain. The outcome *None* is interpreted as negative infinity.

**Return type** `float`

**max**

Returns the maximum value of the domain. The outcome `None` is interpreted as positive infinity.

**Return type** `float`

**is\_continuous**

Whether or not the domain has an uncountable number of values.

**Type** `bool`

**is\_finite**

Whether or not the domain contains a finite number of points.

**Type** `bool`

**dtype**

The numpy dtype of a single element of the domain.

**Type** `np.dtype`

**n\_members**

Returns the number of members in the domain if it *is\_finite*, otherwise, returns `None`.

**Type** `int`

**example\_point**

Returns any single point guaranteed to be in the domain, but no other guarantees; useful for testing purposes. This is given as a size 1 `np.array` of type `dtype`.

**Type** `np.ndarray`

**values**

Returns an `np.array` of type `self.dtype` containing some values from the domain. For domains where *is\_finite* is `True`, all elements of the domain will be yielded exactly once.

**Return type** `np.ndarray`

**in\_domain** (*points*)

Returns `True` if all of the given points are in the domain, `False` otherwise.

**Parameters** **points** (`np.ndarray`) – An `np.ndarray` of type `self.dtype`.

**Return type** `bool`

### 3.4.4 IntegerDomain - (A subset of) Integers

This is the default domain for *FiniteOutcomeModel*.

#### Class Reference

**class** `qinfer.IntegerDomain` (*min=0, max=None*)

Bases: `qinfer.domains.Domain`

A domain specifying a contiguous (and possibly open ended) subset of the integers.

**Parameters**

- **min** (`int`) – A number specifying the lowest possible value of the domain. If `None`, negative infinity is assumed.
- **max** (`int`) – A number specifying the largest possible value of the domain. If left as `None`, positive infinity is assumed.

Note: Yes, it is slightly unpythonic to specify `max` instead of `'max'+1`.

**min**

Returns the minimum value of the domain. The outcome `None` is interpreted as negative infinity.

**Return type** `float`

**max**

Returns the maximum value of the domain. The outcome `None` is interpreted as positive infinity.

**Return type** `float`

**is\_continuous**

Whether or not the domain has an uncountable number of values.

**Type** `bool`

**is\_finite**

Whether or not the domain contains a finite number of points.

**Type** `bool`

**dtype**

The numpy dtype of a single element of the domain.

**Type** `np.dtype`

**n\_members**

Returns the number of members in the domain if it *is\_finite*, otherwise, returns `None`.

**Type** `int`

**example\_point**

Returns any single point guaranteed to be in the domain, but no other guarantees; useful for testing purposes. This is given as a size 1 `np.array` of type `dtype`.

**Type** `np.ndarray`

**values**

Returns an `np.array` of type `self.dtype` containing some values from the domain. For domains where *is\_finite* is `True`, all elements of the domain will be yielded exactly once.

**Return type** `np.ndarray`

**in\_domain** (*points*)

Returns `True` if all of the given points are in the domain, `False` otherwise.

**Parameters** **points** (`np.ndarray`) – An `np.ndarray` of type `self.dtype`.

**Return type** `bool`

### 3.4.5 MultinomialDomain - Tuples of Integers with a Constant Sum

This domain is used by *MultinomialModel*.

#### Class Reference

**class** `qinfer.MultinomialDomain` (*n\_meas*, *n\_elements*=2)

Bases: `qinfer.domains.Domain`

A domain specifying k-tuples of non-negative integers which sum to a specific value.

**Parameters**

- **n\_meas** (*int*) – The sum of any tuple in the domain.
- **n\_elements** (*int*) – The number of elements in a tuple.

**n\_meas**

Returns the sum of any tuple in the domain.

**Return type** *int*

**n\_elements**

Returns the number of elements of a tuple in the domain.

**Return type** *int*

**is\_continuous**

Whether or not the domain has an uncountable number of values.

**Type** *bool*

**is\_finite**

Whether or not the domain contains a finite number of points.

**Type** *bool*

**dtype**

The numpy dtype of a single element of the domain.

**Type** *np.dtype*

**n\_members**

Returns the number of members in the domain if it *is\_finite*, otherwise, returns *None*.

**Type** *int*

**example\_point**

Returns any single point guaranteed to be in the domain, but no other guarantees; useful for testing purposes. This is given as a size 1 *np.array* of type *dtype*.

**Type** *np.ndarray*

**values**

Returns an *np.array* of type *self.dtype* containing some values from the domain. For domains where *is\_finite* is *True*, all elements of the domain will be yielded exactly once.

**Return type** *np.ndarray*

**to\_regular\_array** (*A*)

Converts from an array of type *self.dtype* to an array of type *int* with an additional index labeling the tuple indices.

**Parameters** **A** (*np.ndarray*) – An *np.array* of type *self.dtype*.

**Return type** *np.ndarray*

**from\_regular\_array** (*A*)

Converts from an array of type *int* where the last index is assumed to have length *self.n\_elements* to an array of type *self.dtype* with one fewer index.

**Parameters** **A** (*np.ndarray*) – An *np.array* of type *int*.

**Return type** *np.ndarray*

**in\_domain** (*points*)

Returns *True* if all of the given points are in the domain, *False* otherwise.

**Parameters** **points** (*np.ndarray*) – An *np.ndarray* of type *self.dtype*.

Return type `bool`

## 3.5 Experiment Design Algorithms

### 3.5.1 Optimization

#### ExperimentDesigner - Greedy Risk Minimization Algorithm

##### Class Reference

`class qinfer.ExperimentDesigner(updater, opt_algo=1)`

Bases: `object`

Designs new experiments using the current best information provided by a Bayesian updater.

##### Parameters

- **updater** (`qinfer.smc.SMCUpdater`) – A Bayesian updater to design experiments for.
- **opt\_algo** (`OptimizationAlgorithms`) – Algorithm to be used to perform local optimization.

##### `new_exp()`

Resets this `ExperimentDesigner` instance and prepares for designing the next experiment.

**design\_expparams\_field**(`guess`, `field`, `cost_scale_k=1.0`, `disp=False`, `maxiter=None`, `maxfun=None`, `store_guess=False`, `grad_h=None`, `cost_mult=False`)

Designs a new experiment by varying a single field of a shape `(1,)` record array and minimizing the objective function

$$O(e) = r(e) + k\$(e),$$

where  $r$  is the Bayes risk as calculated by the updater, and where  $\$$  is the cost function specified by the model. Here,  $k$  is a parameter specified to relate the units of the risk and the cost. See [Experiment Design Algorithms](#) for more details.

##### Parameters

- **guess** (Instance of `Heuristic`, `callable` or `ndarray` of dtype `expparams_dtype`) – Either a record array with a single guess, or a callable function that generates guesses.
- **field** (`str`) – The name of the `expparams` field to be optimized. All other fields of `guess` will be held constant.
- **cost\_scale\_k** (`float`) – A scale parameter  $k$  relating the Bayes risk to the experiment cost. See [Experiment Design Algorithms](#).
- **disp** (`bool`) – If `True`, the optimization will print additional information as it proceeds.
- **maxiter** (`int`) – For those optimization algorithms which support it (currently, only CG and NELDER\_MEAD), limits the number of optimization iterations used for each guess.
- **maxfun** (`int`) – For those optimization algorithms which support it (currently, only NCG and NELDER\_MEAD), limits the number of objective calls that can be made.
- **store\_guess** (`bool`) – If `True`, will compare the outcome of this guess to previous guesses and then either store the optimization of this experiment, or the previous best-known experiment design.



- **grad\_h** (*float*) – Step size to use in estimating gradients. Used only if `opt_algo` is NCG.

**Returns** An array representing the best experiment design found so far for the current experiment.

### 3.5.2 Heuristics

**Heuristic - Base class for heuristic experiment designers.**

```
class qinfer.Heuristic(updater)
    Bases: object
```

Defines a heuristic used for selecting new experiments without explicit optimization of the risk. As an example, the  $t_k = (9/8)^k$  heuristic discussed by [FGC12] does not make explicit reference to the risk, and so would be appropriate as a *Heuristic* subclass. In particular, the [FGC12] heuristic is implemented by the *ExpSparseHeuristic* class.

**ExpSparseHeuristic - Exponentially-sparse time-sampling heuristic.**

```
class qinfer.ExpSparseHeuristic(updater, scale=1, base=1.125, t_field=None, other_fields=None)
    Bases: qinfer.expdesign.Heuristic
```

Implements the exponentially-sparse time evolution heuristic of [FGC12], under which  $t_k = Ab^k$ , where  $A$  and  $b$  are parameters of the heuristic.

#### Parameters

- **updater** (*qinfer.smc.SMCUpdater*) – Posterior updater for which experiments should be heuristically designed.
- **scale** (*float*) – The value of  $A$ , implicitly setting the frequency scale for the problem.
- **base** (*float*) – The base of the exponent; in general, should be closer to 1 for higher-dimensional models.
- **t\_field** (*str*) – Name of the expparams field representing time. If `None`, then the generated expparams are taken to be scalar, and not a record.
- **other\_fields** (*dict*) – Values of the other fields to be used in designed experiments.

**PGH - Particle Guess Heuristic**

```
class qinfer.PGH(updater, inv_field='x_', t_field='t', inv_func=<function identity>, t_func=<function identity>, maxiters=10, other_fields=None)
    Bases: qinfer.expdesign.Heuristic
```

Implements the *particle guess heuristic* (PGH) of [WGFC13a], which selects two particles from the current posterior, selects one as an inversion hypothesis and sets the time parameter to be the inverse of the distance between the particles. In this way, the PGH adapts to the current uncertainty without additional simulation resources.

#### Parameters

- **updater** (*qinfer.smc.SMCUpdater*) – Posterior updater for which experiments should be heuristically designed.

- **inv\_field**(*str*) – Name of the `expparams` field corresponding to the inversion hypothesis.
- **t\_field**(*str*) – Name of the `expparams` field corresponding to the evolution time.
- **inv\_func**(*callable*) – Function to be applied to modelparameter vectors to produce an inversion field  $x_-$ .
- **t\_func**(*callable*) – Function to be applied to the evolution time to produce a time field  $t$ .
- **maxiters**(*int*) – Number of times to try and choose distinct particles before giving up.
- **other\_fields**(*dict*) – Values to set for fields not given by the PGH.

Once initialized, a PGH object can be called to generate a new experiment parameter vector:

```
>>> pgh = PGH(updater)
>>> expparams = pgh()
```

If the posterior weights are very highly peaked (that is, if the effective sample size is too small, as measured by `n_ess`), then it may be the case that the two particles chosen by the PGH are identical, such that the time would be determined by  $1 / 0$ . In this case, the `PGH` class will instead draw new pairs of particles until they are not identical, up to `maxiters` attempts. If that limit is reached, a `RuntimeError` will be raised.

## 3.6 GPU-Accelerated Models

### 3.6.1 Introduction

These models demonstrate using GPU acceleration with `PyOpenCL` to efficiently perform likelihood calls.

### 3.6.2 AcceleratedPrecessionModel - GPU model for a single qubit Larmor precession

```
class qinfer.AcceleratedPrecessionModel(context=None)
    Bases: qinfer.abstract_model.FiniteOutcomeModel

    Reimplementation of qinfer.test_models.SimplePrecessionModel, using OpenCL to accelerate
    computation.

    n_modelparams
    expparams_dtype
    is_n_outcomes_constant
        Returns True if and only if the number of outcomes for each experiment is independent of the experiment
        being performed.

        This property is assumed by inference engines to be constant for the lifetime of a Model instance.

    static are_models_valid(modelparams)

    n_outcomes(expparams)
        Returns an array of dtype uint describing the number of outcomes for each experiment specified by
        expparams.

        Parameters expparams (numpy.ndarray) – Array of experimental parameters. This array
        must be of dtype agreeing with the expparams_dtype property.
```

`likelihood(outcomes, modelparams, expparams)`

## 3.7 IPython/Jupyter Support

### 3.7.1 Introduction

These classes integrate with Jupyter Notebook using the `ipywidgets` package.

### 3.7.2 IPythonProgressBar - Progress bar for Jupyter Notebook

`class qinfer.IPythonProgressBar`  
Bases: `object`

Represents a progress bar as an IPython widget. If the widget is closed by the user, or by calling `finalize()`, any further operations will be ignored.

---

**Note:** This progress bar is compatible with QuTiP progress bar classes.

---

**description**

Text description for the progress bar widget, or `None` if the widget has been closed.

**Type** `str`

**start(max)**

Displays the progress bar for a given maximum value.

**Parameters** `max(float)` – Maximum value of the progress bar.

**update(n)**

Updates the progress bar to display a new value.

**finished()**

Destroys the progress bar.

## 3.8 Mixin Classes for Model Development

### 3.8.1 ScoreMixin - Numerical Differentiation for Fisher Scores

`class qinfer.ScoreMixin`  
Bases: `object`

A mixin which includes a method `score` that numerically estimates the score of the likelihood function. Any class which mixes in this class should be equipped with a property `n_modelparams` and a method `likelihood` to satisfy dependency.

**h**

Returns the step size to be used in numerical differentiation with respect to the model parameters.

The step size is given as a vector with length `n_modelparams` so that each model parameter can be weighted independently.

**score** (*outcomes, modelparams, expparams, return\_L=False*)

Returns the numerically computed score of the likelihood function, defined as:

$$q(d, \mathbf{x}; \mathbf{e}) = \nabla_{\mathbf{x}} \log \Pr(d|\mathbf{x}; \mathbf{e}).$$

Calls are represented as a four-index tensor `score[idx_modelparam, idx_outcome, idx_model, idx_experiment]`. The left-most index may be suppressed for single-parameter models.

The numerical gradient is computed using the central difference method, with step size given by the property `h`.

If `return_L` is True, both `q` and the likelihood `L` are returned as `q, L`.

## 3.9 Parallelized Models

### 3.9.1 DirectViewParallelizedModel

**class** `qinfer.DirectViewParallelizedModel` (*serial\_model, direct\_view, purge\_client=False, serial\_threshold=None*)  
 Bases: `qinfer.derived_models.DerivedModel`

Given an instance of a [Model](#), parallelizes execution of that model's likelihood by breaking the `modelparams` array into segments and executing a segment on each member of a [DirectView](#).

This [Model](#) assumes that it has ownership over the [DirectView](#), such that no other processes will send tasks during the lifetime of the [Model](#).

If you are having trouble pickling your model, consider switching to `dill` by calling `direct_view.use_dill()`. This mode gives more support for closures.

#### Parameters

- **serial\_model** (`qinfer.Model`) – Model to be parallelized. This model will be distributed to the engines in the direct view, such that the model must support pickling.
- **direct\_view** (`ipyparallel.DirectView`) – Direct view onto the engines that will be used to parallelize evaluation of the model's likelihood function.
- **purge\_client** (`bool`) – If True, then this model will purge results and metadata from the IPython client whenever the model cache is cleared. This is useful for solving memory leaks caused by very large numbers of calls to `likelihood`. By default, this is disabled, since enabling this option can cause data loss if the client is being sent other tasks during the operation of this model.
- **serial\_threshold** (`int`) – Sets the number of model vectors below which the serial model is to be preferred. By default, this is set to `10 * n_engines`, where `n_engines` is the number of engines exposed by `direct_view`.

#### `n_engines`

The number of engines seen by the direct view owned by this parallelized model.

#### Return type `int`

#### **clear\_cache** ()

Clears any cache associated with the serial model and the engines seen by the direct view.

#### **likelihood** (*outcomes, modelparams, expparams*)

Returns the likelihood for the underlying (serial) model, distributing the model parameter array across the engines controlled by this parallelized model.

## 3.10 Performance Testing

### 3.10.1 Introduction

These functions provide performance testing support, allowing for the quick comparison of models, experiment design heuristics and quality parameters. QInfer’s performance testing functionality can be quickly applied without writing lots of boilerplate code every time. For instance:

```
>>> import qinfer
>>> n_particles = int(1e5)
>>> perf = qinfer.perf_test(
...     qinfer.SimplePrecessionModel(), n_particles,
...     qinfer.UniformDistribution([0, 1]), 200,
...     qinfer.ExpSparseHeuristic
... )
```

### 3.10.2 Function Reference

`qinfer.perf_test(model, n_particles, prior, n_exp, heuristic_class, true_model=None, true_prior=None, true_mps=None, extra_updater_args=None)`

Runs a trial of using SMC to estimate the parameters of a model, given a number of particles, a prior distribution and an experiment design heuristic.

#### Parameters

- **model** (`qinfer.Model`) – Model whose parameters are to be estimated.
- **n\_particles** (`int`) – Number of SMC particles to use.
- **prior** (`qinfer.Distribution`) – Prior to use in selecting SMC particles.
- **n\_exp** (`int`) – Number of experimental data points to draw from the model.
- **heuristic\_class** (`qinfer.Heuristic`) – Constructor function for the experiment design heuristic to be used.
- **true\_model** (`qinfer.Model`) – Model to be used in generating experimental data. If `None`, assumed to be `model`. Note that if the true and estimation models have different numbers of parameters, the loss will be calculated by aligning the respective model vectors “at the right,” analogously to the convention used by NumPy broadcasting.
- **true\_prior** (`qinfer.Distribution`) – Prior to be used in selecting the true model parameters. If `None`, assumed to be `prior`.
- **true\_mps** (`numpy.ndarray`) – The true model parameters. If `None`, it will be sampled from `true_prior`. Note that as this function runs exactly one trial, only one model parameter vector may be passed. In particular, this requires that `len(true_mps.shape) == 1`.
- **extra\_updater\_args** (`dict`) – Extra keyword arguments for the updater, such as re-sampling and zero-weight policies.

**Rtype** `np.ndarray` See [Performance Results Structure](#) for more details on the type returned by this function.

**Returns** A record array of performance metrics, indexed by the number of experiments performed.

```
qinfer.perf_test_multiple(n_trials, model, n_particles, prior, n_exp, heuristic_class,
                          true_model=None, true_prior=None, true_mps=None, apply=<class
                          'qinfer.perf_testing.apply_serial'>, allow_failures=False, ex-
                          tra_updater_args=None, progressbar=None)
```

Runs many trials of using SMC to estimate the parameters of a model, given a number of particles, a prior distribution and an experiment design heuristic.

In addition to the parameters accepted by `perf_test()`, this function takes the following arguments:

#### Parameters

- **n\_trials** (*int*) – Number of different trials to run.
- **apply** (*callable*) – Function to call to delegate each trial. See, for example, `apply()`.
- **progressbar** (*qutip.ui.BaseProgressBar*) – QuTiP-style progress bar class used to report how many trials have successfully completed.
- **allow\_failures** (*bool*) – If `False`, an exception raised in any trial will propagate out. Otherwise, failed trials are masked out of the returned performance array using NumPy masked arrays.

**Rtype** `np.ndarray` See *Performance Results Structure* for more details on the type returned by this function.

**Returns** A record array of performance metrics, indexed by the trial and the number of experiments performed.

### 3.10.3 Performance Results Structure

Performance results, as collected by `perf_test()`, are returned as a *record array* with several fields, each describing a different metric collected by **QInfer** about the performance. In addition to these fields, each field in `model.expparams_dtype` is added as a field to the performance results structure to record what measurements are performed.

For a single performance trial, the shape of the performance results array is `(n_exp, )`, such that `perf[idx_exp]` returns metrics describing the performance immediately following collecting the datum `idx_exp`. Some fields are not scalar-valued, such that `perf[field]` then has shape `(n_exp, ) + field_shape`.

On the other hand, when multiple trials are collected by `perf_test_multiple`, the results are returned as an array with the same fields, but with an additional index over trials, for a shape of `(n_trials, n_exp)`.

| Field                                                                                                                                                                                                                                                                                                                                                   | Type               | Shape                                     |
|---------------------------------------------------------------------------------------------------------------------------------------------------------------------------------------------------------------------------------------------------------------------------------------------------------------------------------------------------------|--------------------|-------------------------------------------|
| <code>elapsed_time</code>                                                                                                                                                                                                                                                                                                                               | <code>float</code> | scalar                                    |
| Time (in seconds) elapsed during the SMC update for this experiment. Includes resampling, but excludes experiment design, generation of "true" data and calculation of performance metrics.                                                                                                                                                             |                    |                                           |
| <code>loss</code>                                                                                                                                                                                                                                                                                                                                       | <code>float</code> | scalar                                    |
| Decision-theoretic loss incurred by the estimate after updating with this experiment, given by the quadratic loss $\text{Tr}(Q(\hat{x} - x)(\hat{x} - x)^T)$ . If the true and estimation models have different numbers of parameters, the loss will only be evaluated for those parameters that are in common (aligning the two vectors at the right). |                    |                                           |
| <code>resample_count</code>                                                                                                                                                                                                                                                                                                                             | <code>int</code>   | scalar                                    |
| Number of times that resampling was performed on the SMC updater.                                                                                                                                                                                                                                                                                       |                    |                                           |
| <code>outcome</code>                                                                                                                                                                                                                                                                                                                                    | <code>int</code>   | scalar                                    |
| Outcome of the experiment that was performed.                                                                                                                                                                                                                                                                                                           |                    |                                           |
| <code>true</code>                                                                                                                                                                                                                                                                                                                                       | <code>float</code> | <code>(true_model.n_modelparams, )</code> |
| Vector of model parameters used to simulate data. For time-dependent models, this changes with each experiment as per <code>true_model.update_timestep</code> .                                                                                                                                                                                         |                    |                                           |
| <code>est</code>                                                                                                                                                                                                                                                                                                                                        | <code>float</code> | <code>(model.n_modelparams, )</code>      |
| Mean vector of model parameters over the current posterior.                                                                                                                                                                                                                                                                                             |                    |                                           |

## 3.11 Randomized Benchmarking

### 3.11.1 RandomizedBenchmarkingModel - Likelihood for RB experiments

#### Class Reference

**class** `qinfer.RandomizedBenchmarkingModel` (*interleaved=False, order=0*)

Bases: `qinfer.abstract_model.FiniteOutcomeModel`, `qinfer.abstract_model.DifferentiableModel`

Implements the randomized benchmarking or interleaved randomized benchmarking protocol, such that the depolarizing strength  $p$  of the twirled channel is a parameter to be estimated, given a sequence length  $m$  as an experimental control. In addition, the zeroth-order "fitting"-parameters  $A$  and  $B$  are represented as model parameters to be estimated.

**Parameters** `interleaved` (*bool*) – If `True`, the model implements the interleaved protocol, with  $\tilde{p}$  being the depolarizing parameter for the interleaved gate and with  $p_{\text{ref}}$  being the reference parameter.

#### Model Parameters

- **p** – Fidelity of the twirled error channel  $\Lambda$ , represented as a decay rate  $p = (dF - 1)/(d - 1)$ , where  $F$  is the fidelity and  $d$  is the dimension of the Hilbert space.
- **A** – Scale of the randomized benchmarking decay, defined as  $\text{Tr}[Q\Lambda(\rho - \mathbb{1}/d)]$ , where  $Q$  is the final measurement, and where  $\mathbb{1}$  is the initial preparation.

- **B** – Offset of the randomized benchmarking decay, defined as  $\text{Tr}[Q\Lambda(\mathbb{1}/d)]$ .

#### Experiment Parameters

- **m** (*int*) – Length of the randomized benchmarking sequence that was measured.

```

n_modelparams
modelparam_names
is_n_outcomes_constant
expparams_dtype
n_outcomes (expparams)
are_models_valid (modelparams)
likelihood (outcomes, modelparams, expparams)
score (outcomes, modelparams, expparams, return_L=False)

```

## Function Reference

`qinfer.rb.p(F, d=2)`

Given the fidelity of a gate in  $d$  dimensions, returns the depolarizing probability of the twirled channel.

#### Parameters

- **F** (*float*) – Fidelity of a gate.
- **d** (*int*) – Dimensionality of the Hilbert space on which the gate acts.

`qinfer.rb.F(p, d=2)`

Given the depolarizing probability of a twirled channel in  $d$  dimensions, returns the fidelity of the original gate.

#### Parameters

- **p** (*float*) – Depolarizing parameter for the twirled channel.
- **d** (*int*) – Dimensionality of the Hilbert space on which the gate acts.

## 3.12 Resampling Algorithms

### 3.12.1 Introduction

In order to restore numerical stability to the sequential Monte Carlo algorithm as the effective sample size is reduced, *resampling* is used to adaptively move particles so as to better represent the posterior distribution. **QInfer** allows for such algorithms to be specified in a modular way.

### 3.12.2 LiuWestResampler - Liu and West (2000) resampling algorithm

#### Class Reference

```

class qinfer.LiuWestResampler(a=0.98, h=None, maxiter=1000, debug=False, postselect=True,
                              zero_cov_comp=1e-10, kernel=<built-in method randn of
                              mtrand.RandomState object>)

```

Bases: `object`

Creates a resampler instance that applies the algorithm of [LW01] to redistribute the particles.



#### Parameters

- **a** (*float*) – Value of the parameter  $a$  of the [LW01] algorithm to use in resampling.
- **h** (*float*) – Value of the parameter  $h$  to use, or `None` to use that corresponding to  $a$ .
- **maxiter** (*int*) – Maximum number of times to attempt to resample within the space of valid models before giving up.
- **debug** (*bool*) – Because the resampler can generate large amounts of debug information, nothing is output to the logger, even at DEBUG level, unless this flag is `True`.
- **postselect** (*bool*) – If `True`, ensures that models are valid by postselecting.
- **zero\_cov\_comp** (*float*) – Amount of covariance to be added to every parameter during resampling in the case that the estimated covariance has zero norm.
- **kernel** (*callable*) – Callable function `kernel(*shape)` that returns samples from a resampling distribution with mean 0 and variance 1.

**Warning:** The [LW01] algorithm preserves the first two moments of the distribution (in expectation over the random choices made by the resampler) if and only if  $a^2 + h^2 = 1$ , as is set by the `h=None` keyword argument.

a

## 3.13 Simple Estimation

### 3.13.1 Function Reference

`qinfer.simple_est_prec(data, freq_min=0.0, freq_max=1.0, n_particles=6000, return_all=False)`

Estimates a simple precession ( $\cos^2$ ) from experimental data. Note that this model is mainly for testing purposes, as it does not consider the phase or amplitude of precession, leaving only the frequency.

#### Parameters

- **data** (see *Data Argument Type*) – Data to be used in estimating the precession frequency.
- **freq\_min** (*float*) – The minimum feasible frequency to consider.
- **freq\_max** (*float*) – The maximum feasible frequency to consider.
- **n\_particles** (*int*) – The number of particles to be used in estimating the precession frequency.
- **return\_all** (*bool*) – Controls whether additional return values are provided, such as the updater.

#### Columns

- **counts** (*int*) – How many counts were observed at the sampled time.
- **t** (*float*) – The evolution time at which the samples were collected.
- **n\_shots** (*int*) – How many samples were collected at the given evolution time.

**Return mean** Bayesian mean estimator for the precession frequency.

**Return var** Variance of the final posterior over frequency.

**Return extra** See *Extra Return Values*. Only returned if `return_all` is `True`.

`qinfer.simple_est_rb(data, interleaved=False, p_min=0.0, p_max=1.0, n_particles=8000, return_all=False)`

Estimates the fidelity of a gateset from a standard or interleaved randomized benchmarking experiment.

#### Parameters

- **data** (see *Data Argument Type*) – Data to be used in estimating the gateset fidelity.
- **p\_min** (*float*) – Minimum value of the parameter  $p$  to consider feasible.
- **p\_max** (*float*) – Minimum value of the parameter  $p$  to consider feasible.
- **n\_particles** (*int*) – The number of particles to be used in estimating the randomized benchmarking model.
- **return\_all** (*bool*) – Controls whether additional return values are provided, such as the updater.

#### Columns

- **counts** (*int*) – How many sequences of length  $m$  were observed to survive.
- **m** (*int*) – How many gates were used for sequences in this row of the data.
- **n\_shots** (*int*) – How many different sequences of length  $m$  were measured.
- **reference** (*bool*) – `True` if this row represents reference sequences, or `False` if the gate of interest is interleaved. Note that this column is omitted if `interleaved` is `False`.

**Return mean** Bayesian mean estimator for the model vector  $(p, A, B)$ , or  $(\tilde{p}, p_{\text{ref}}, A, B)$  for the interleaved case.

**Return var** Variance of the final posterior over RB model vectors.

**Return extra** See *Extra Return Values*. Only returned if `return_all` is `True`.

### 3.13.2 Data Argument Type

Each of the functions above takes as its first argument the data to be used in estimation. This data can be passed in two different ways (more will be added soon):

- A *file-like object* or a `str` containing a file name: These will cause the data to be loaded from the given file as comma-separated values. Columns will be read in based on the order in which they appear in the file.
- A `DataFrame`: This will cause the data to be loaded from the given data frame, reading in columns by their headings.
- An `ndarray` with scalar data type and shape `(n_rows, n_cols)`: Each column will be read in by its order.
- An `ndarray` with record data types and shape `(n_rows, )`: Each column will be read in as a field of the array.

### 3.13.3 Extra Return Values

Each of the functions above supports an argument `return_all`. If `True`, a dictionary with the following fields will be returned as well:

- **updater** (*SMCUpdater*): An updater representing the final posterior for the estimation procedure.

## 3.14 Sequential Monte Carlo

### 3.14.1 SMCUpdater - SMC-Based Particle Updater

#### Class Reference

```
class qinfer.SMCUpdater(model, n_particles, prior, resample_a=None, resam-
                        pler=None, resample_thresh=0.5, debug_resampling=False,
                        track_resampling_divergence=False, zero_weight_policy='error',
                        zero_weight_thresh=None, canonicalize=True)
```

Bases: `qinfer.distributions.Distribution`

Creates a new Sequential Monte carlo updater, using the algorithm of [\[GFWC12\]](#).

#### Parameters

- **model** (`Model`) – Model whose parameters are to be inferred.
- **n\_particles** (`int`) – The number of particles to be used in the particle approximation.
- **prior** (`Distribution`) – A representation of the prior distribution.
- **resampler** (`callable`) – Specifies the resampling algorithm to be used. See [Resampling Algorithms](#) for more details.
- **resample\_thresh** (`float`) – Specifies the threshold for  $N_{\text{ess}}$  to decide when to resample.
- **debug\_resampling** (`bool`) – If `True`, debug information will be generated on resampling performance, and will be written to the standard Python logger.
- **track\_resampling\_divergence** (`bool`) – If true, then the divergences between the pre- and post-resampling distributions are tracked and recorded in the `resampling_divergences` attribute.
- **zero\_weight\_policy** (`str`) – Specifies the action to be taken when the particle weights would all be set to zero by an update. One of ["ignore", "skip", "warn", "error", "reset"].
- **zero\_weight\_thresh** (`float`) – Value to be used when testing for the zero-weight condition.
- **canonicalize** (`bool`) – If `True`, particle locations will be updated to canonical locations as described by the model class after each prior sampling and resampling.

#### **n\_particles**

Returns the number of particles currently used in the sequential Monte Carlo approximation.

Type `int`

#### **resample\_count**

Returns the number of times that the updater has resampled the particle approximation.

Type `int`

#### **just\_resampled**

`True` if and only if there has been no data added since the last resampling, or if there has not yet been a resampling step.

Type `bool`

**normalization\_record**

Returns the normalization record.

Type `float`

**log\_total\_likelihood**

Returns the log-likelihood of all the data collected so far.

Equivalent to:

`np.sum(np.log(updater.normalization_record))`

Type `float`

**n\_ess**

Estimates the effective sample size (ESS) of the current distribution over model parameters.

Type `float`

Returns The effective sample size, given by  $1 / \sum_i w_i^2$ .

**min\_n\_ess**

Returns the smallest effective sample size (ESS) observed in the history of this updater.

Type `float`

Returns The minimum of observed effective sample sizes as reported by `n_ess`.

**data\_record**

List of outcomes given to `update()`.

Type `list of int`

**resampling\_divergences**

List of KL divergences between the pre- and post-resampling distributions, if that is being tracked. Otherwise, `None`.

Type `list of float or None`

**reset** (*n\_particles=None, only\_params=None, reset\_weights=True*)

Causes all particle locations and weights to be drawn fresh from the initial prior.

**Parameters**

- **n\_particles** (*int*) – Forces the size of the new particle set. If `None`, the size of the particle set is not changed.
- **only\_params** (*slice*) – Resets only some of the parameters. Cannot be set if `n_particles` is also given.
- **reset\_weights** (*bool*) – Resets the weights as well as the particles.

**hypothetical\_update** (*outcomes, expparams, return\_likelihood=False, return\_normalization=False*)

Produces the particle weights for the posterior of a hypothetical experiment.

**Parameters**

- **outcomes** (*int or an ndarray of dtype int.*) – Integer index of the outcome of the hypothetical experiment.
- **expparams** (*numpy.ndarray*) – Experiments to be used for the hypothetical updates.

- **weights** (`ndarray`, `shape` (`n_outcomes`, `n_expparams`, `n_particles`)) – Weights assigned to each particle in the posterior distribution  $\Pr(\omega|d)$ .

**update** (`outcome`, `expparams`, `check_for_resample=True`)

Given an experiment and an outcome of that experiment, updates the posterior distribution to reflect knowledge of that experiment.

After updating, resamples the posterior distribution if necessary.

#### Parameters

- **outcome** (`int`) – Label for the outcome that was observed, as defined by the `Model` instance under study.
- **expparams** (`ndarray` of dtype given by the `expparams_dtype` property of the underlying model) – Parameters describing the experiment that was performed.
- **check\_for\_resample** (`bool`) – If `True`, after performing the update, the effective sample size condition will be checked and a resampling step may be performed.

**batch\_update** (`outcomes`, `expparams`, `resample_interval=5`)

Updates based on a batch of outcomes and experiments, rather than just one.

#### Parameters

- **outcomes** (`numpy.ndarray`) – An array of outcomes of the experiments that were performed.
- **expparams** (`numpy.ndarray`) – Either a scalar or record single-index array of experiments that were performed.
- **resample\_interval** (`int`) – Controls how often to check whether  $N_{\text{ess}}$  falls below the resample threshold.

**resample** ()

Forces the updater to perform a resampling step immediately.

**n\_rvs**

The number of random variables described by the posterior distribution.

**sample** (`n=1`)

Returns samples from the current posterior distribution.

**Parameters** `n` (`int`) – The number of samples to draw.

**Returns** The sampled model parameter vectors.

**Return type** `ndarray` of shape (`n`, `updater.n_rvs`).

**est\_mean** ()

Returns an estimate of the posterior mean model, given by the expectation value over the current SMC approximation of the posterior model distribution.

**Return type** `numpy.ndarray`, `shape` (`n_modelparams`,).

**Returns** An array containing the an estimate of the mean model vector.

**est\_meanfn** (`fn`)

Returns an estimate of the expectation value of a given function  $f$  of the model parameters, given by a sum over the current SMC approximation of the posterior distribution over models.

Here,  $f$  is represented by a function `fn` that is vectorized over particles, such that `f(modelparams)` has shape `(n_particles, k)`, where `n_particles = modelparams.shape[0]`, and where `k` is a positive integer.

**Parameters** `fn` (*callable*) – Function implementing  $f$  in a vectorized manner. (See above.)

**Return type** `numpy.ndarray`, shape `(k, )`.

**Returns** An array containing the an estimate of the mean of  $f$ .

**est\_covariance\_mtx** (`corr=False`)

Returns an estimate of the covariance of the current posterior model distribution, given by the covariance of the current SMC approximation.

**Parameters** `corr` (*bool*) – If `True`, the covariance matrix is normalized by the outer product of the square root diagonal of the covariance matrix such that the correlation matrix is returned instead.

**Return type** `numpy.ndarray`, shape `(n_modelparams, n_modelparams)`.

**Returns** An array containing the estimated covariance matrix.

**bayes\_risk** (`expparams`)

Calculates the Bayes risk for a hypothetical experiment, assuming the quadratic loss function defined by the current model's scale matrix (see `qinfer.abstract_model.Simulatable.Q`).

**Parameters** `expparams` (`ndarray` of dtype given by the current model's `expparams_dtype` property, and of shape `(1,)`) – The experiment at which to compute the Bayes risk.

**Return float** The Bayes risk for the current posterior distribution of the hypothetical experiment `expparams`.

**expected\_information\_gain** (`expparams`)

Calculates the expected information gain for a hypothetical experiment.

**Parameters** `expparams` (`ndarray` of dtype given by the current model's `expparams_dtype` property, and of shape `(1,)`) – The experiment at which to compute expected information gain.

**Return float** The Bayes risk for the current posterior distribution of the hypothetical experiment `expparams`.

**est\_entropy** ()

Estimates the entropy of the current posterior as  $-\sum_i w_i \log w_i$  where  $\{w_i\}$  is the set of particles with nonzero weight.

**est\_kl\_divergence** (`other`, `kernel=None`, `delta=0.01`)

Finds the KL divergence between this and another SMC-approximated distribution by using a kernel density estimator to smooth over the other distribution's particles.

**Parameters** `other` (`SMCUpdater`) –

**est\_cluster\_moments** (`cluster_opts=None`)

**est\_cluster\_covs** (`cluster_opts=None`)

**est\_cluster\_metric** (`cluster_opts=None`)

Returns an estimate of how much of the variance in the current posterior can be explained by a separation between *clusters*.

**est\_credible\_region** (`level=0.95`, `return_outside=False`, `modelparam_slice=None`)

Returns an array containing particles inside a credible region of a given level, such that the described region has probability mass no less than the desired level.

Particles in the returned region are selected by including the highest- weight particles first until the desired credibility level is reached.

#### Parameters

- **level** (*float*) – Credibility level to report.
- **return\_outside** (*bool*) – If `True`, the return value is a tuple of the those particles within the credible region, and the rest of the posterior particle cloud.
- **modelparam\_slice** (*slice*) – Slice over which model parameters to consider.

#### Return type

`numpy.ndarray`, shape `(n_credible, n_mps)`, where `n_credible` is the number of particles in the credible region and `n_mps` corresponds to the size of `modelparam_slice`.

If `return_outside` is `True`, this method instead returns tuple `(inside, outside)` where `inside` is as described above, and `outside` has shape `(n_particles-n_credible, n_mps)`.

**Returns** An array of particles inside the estimated credible region. Or, if `return_outside` is `True`, both the particles inside and the particles outside, as a tuple.

**region\_est\_hull** (*level=0.95, modelparam\_slice=None*)

Estimates a credible region over models by taking the convex hull of a credible subset of particles.

#### Parameters

- **level** (*float*) – The desired credibility level (see `SMCUpdater.est_credible_region()`).
- **modelparam\_slice** (*slice*) – Slice over which model parameters to consider.

**Returns** The tuple `(faces, vertices)` where `faces` describes all the vertices of all of the faces on the exterior of the convex hull, and `vertices` is a list of all vertices on the exterior of the convex hull.

**Return type** `faces` is a `numpy.ndarray` with shape `(n_face, n_mps, n_mps)` and indices `(idx_face, idx_vertex, idx_mps)` where `n_mps` corresponds to the size of `modelparam_slice`. `vertices` is a `numpy.ndarray` of shape `(n_vertices, n_mps)`.

**region\_est\_ellipsoid** (*level=0.95, tol=0.0001, modelparam\_slice=None*)

Estimates a credible region over models by finding the minimum volume enclosing ellipse (MVEE) of a credible subset of particles.

#### Parameters

- **level** (*float*) – The desired credibility level (see `SMCUpdater.est_credible_region()`).
- **tol** (*float*) – The allowed error tolerance in the MVEE optimization (see `mvee()`).
- **modelparam\_slice** (*slice*) – Slice over which model parameters to consider.

**Returns** A tuple `(A, c)` where `A` is the covariance matrix of the ellipsoid and `c` is the center. A point  $x$  is in the ellipsoid whenever  $(x - c)^T A^{-1} (x - c) \leq 1$ .

**Return type** `A` is `np.ndarray` of shape `(n_mps, n_mps)` and `centroid` is `np.ndarray` of shape `(n_mps)`. `n_mps` corresponds to the size of `param_slice`.

**in\_credible\_region** (*points*, *level*=0.95, *modelparam\_slice*=None, *method*='hpd-hull', *tol*=0.0001)

Decides whether each of the points lie within a credible region of the current distribution.

If *tol* is None, the particles are tested directly against the convex hull object. If *tol* is a positive float, particles are tested to be in the interior of the smallest enclosing ellipsoid of this convex hull, see [`SMCUpdater.region\_est\_ellipsoid\(\)`](#).

#### Parameters

- **points** (*np.ndarray*) – An *np.ndarray* of shape (*n\_mps*) for a single point, or of shape (*n\_points*, *n\_mps*) for multiple points, where *n\_mps* corresponds to the same dimensionality as *param\_slice*.
- **level** (*float*) – The desired credibility level (see [`SMCUpdater.est\_credible\_region\(\)`](#)).
- **method** (*str*) – A string specifying which credible region estimator to use. One of 'pce', 'hpd-hull' or 'hpd-mvee' (see below).
- **tol** (*float*) – The allowed error tolerance for those methods which require a tolerance (see [`mvee\(\)`](#)).
- **modelparam\_slice** (*slice*) – A slice describing which model parameters to consider in the credible region, effectively marginizing out the remaining parameters. By default, all model parameters are included.

**Returns** A boolean array of shape (*n\_points*, ) specifying whether each of the points lies inside the confidence region.

The following values are valid for the *method* argument.

- **'pce': Posterior Covariance Ellipsoid.** Computes the covariance matrix of the particle distribution marginalized over the excluded slices and uses the  $\chi^2$  distribution to determine how to rescale it such the the corresponding ellipsoid has the correct size. The ellipsoid is translated by the mean of the particle distribution. It is determined which of the *points* are on the interior.
- **'hpd-hull': High Posterior Density Convex Hull.** See [`SMCUpdater.region\_est\_hull\(\)`](#). Computes the HPD region resulting from the particle approximation, computes the convex hull of this, and it is determined which of the *points* are on the interior.
- **'hpd-mvee': High Posterior Density Minimum Volume Enclosing Ellipsoid.** See [`SMCUpdater.region\_est\_ellipsoid\(\)`](#) and [`mvee\(\)`](#). Computes the HPD region resulting from the particle approximation, computes the convex hull of this, and determines the minimum enclosing ellipsoid. Determines which of the *points* are on the interior.

**risk** (*x0*)

**posterior\_marginal** (*idx\_param*=0, *res*=100, *smoothing*=0, *range\_min*=None, *range\_max*=None)

Returns an estimate of the marginal distribution of a given model parameter, based on taking the derivative of the interpolated cdf.

#### Parameters

- **idx\_param** (*int*) – Index of parameter to be marginalized.
- **res1** (*int*) – Resolution of of the axis.
- **smoothing** (*float*) – Standard deviation of the Gaussian kernel used to smooth; same units as parameter.
- **range\_min** (*float*) – Minimum range of the output axis.



- **range\_max** (*float*) – Maximum range of the output axis.

See also:

`SMCUpdater.plot_posterior_marginal()`

**plot\_posterior\_marginal** (*idx\_param*=0, *res*=100, *smoothing*=0, *range\_min*=None, *range\_max*=None, *label\_xaxis*=True, *other\_plot\_args*={}, *true\_model*=None)

Plots a marginal of the requested parameter.

#### Parameters

- **idx\_param** (*int*) – Index of parameter to be marginalized.
- **res1** (*int*) – Resolution of of the axis.
- **smoothing** (*float*) – Standard deviation of the Gaussian kernel used to smooth; same units as parameter.
- **range\_min** (*float*) – Minimum range of the output axis.
- **range\_max** (*float*) – Maximum range of the output axis.
- **label\_xaxis** (*bool*) – Labels the *x*-axis with the model parameter name given by this updater’s model.
- **other\_plot\_args** (*dict*) – Keyword arguments to be passed to matplotlib’s `plot` function.
- **true\_model** (*np.ndarray*) – Plots a given model parameter vector as the “true” model for comparison.

See also:

`SMCUpdater.posterior_marginal()`

**plot\_covariance** (*corr*=False, *param\_slice*=None, *tick\_labels*=None, *tick\_params*=None)

Plots the covariance matrix of the posterior as a Hinton diagram.

---

**Note:** This function requires that `mpltools` is installed.

---

#### Parameters

- **corr** (*bool*) – If `True`, the covariance matrix is first normalized by the outer product of the square root diagonal of the covariance matrix such that the correlation matrix is plotted instead.
- **param\_slice** (*slice*) – Slice of the model parameters to be plotted.
- **tick\_labels** (*list*) – List of tick labels for each component; by default, these are drawn from the model itself.

**posterior\_mesh** (*idx\_param1*=0, *idx\_param2*=1, *res1*=100, *res2*=100, *smoothing*=0.01)

Returns a mesh, useful for plotting, of kernel density estimation of a 2D projection of the current posterior distribution.

#### Parameters

- **idx\_param1** (*int*) – Parameter to be treated as *x* when plotting.
- **idx\_param2** (*int*) – Parameter to be treated as *y* when plotting.
- **res1** (*int*) – Resolution along the *x* direction.

- **res2** (*int*) – Resolution along the  $y$  direction.
- **smoothing** (*float*) – Standard deviation of the Gaussian kernel used to smooth the particle approximation to the current posterior.

See also:

`SMCUpdater.plot_posterior_contour()`

**plot\_posterior\_contour** (*idx\_param1=0, idx\_param2=1, res1=100, res2=100, smoothing=0.01*)

Plots a contour of the kernel density estimation of a 2D projection of the current posterior distribution.

#### Parameters

- **idx\_param1** (*int*) – Parameter to be treated as  $x$  when plotting.
- **idx\_param2** (*int*) – Parameter to be treated as  $y$  when plotting.
- **res1** (*int*) – Resolution along the  $x$  direction.
- **res2** (*int*) – Resolution along the  $y$  direction.
- **smoothing** (*float*) – Standard deviation of the Gaussian kernel used to smooth the particle approximation to the current posterior.

See also:

`SMCUpdater.posterior_mesh()`

## 3.15 Testing Models

### 3.15.1 Introduction

QInfer provides several premade models for quickly learning how to use the library, for making demonstrations, or to test new algorithms and approaches built on top of QInfer.

### 3.15.2 SimplePrecessionModel - Model of a single qubit undergoing Larmor precession

**class** `qinfer.SimplePrecessionModel` (*min\_freq=0*)

Bases: `qinfer.test_models.SimpleInversionModel`

Describes the free evolution of a single qubit prepared in the  $|+\rangle$  state under a Hamiltonian  $H = \omega\sigma_z/2$ , as explored in [GFWC12].

**Parameters** **min\_freq** (*float*) – Minimum value for  $\omega$  to accept as valid. This is used for testing techniques that mitigate the effects of degenerate models; there is no “good” reason to ever set this to be less than zero, other than to test with an explicitly broken model.

**Model Parameters** **omega** – The precession frequency  $\omega$ .

**Experiment Parameter** **float** *t* – The evolution time  $t$ .

**expparams\_dtype**

**likelihood** (*outcomes, modelparams, expparams*)

**score** (*outcomes, modelparams, expparams, return\_L=False*)

### 3.15.3 NoisyCoinModel - Classical coin flip model corrupted by a noisy process

**class** qinfer.NoisyCoinModel

Bases: qinfer.abstract\_model.FiniteOutcomeModel

Implements the “noisy coin” model of [FB12], where the model parameter  $p$  is the probability of the noisy coin. This model has two experiment parameters,  $\alpha$  and  $\beta$ , which are the probabilities of observing a “0” outcome conditioned on the “true” outcome being 0 and 1, respectively. That is, for an ideal coin,  $\alpha = 1$  and  $\beta = 0$ .

Note that  $\alpha$  and  $\beta$  are implemented as experiment parameters not because we expect to design over those values, but because a specification of each is necessary to honestly describe an experiment that was performed.

**Model Parameters** **p** – “Heads” probability  $p$ .

**Experiment Parameters**

- **alpha** (*float*) – Visibility parameter  $\alpha$ .
- **beta** (*float*) – Visibility parameter  $\beta$ .

**n\_modelparams**

**expparams\_dtype**

**is\_n\_outcomes\_constant**

**static are\_models\_valid** (*modelparams*)

**n\_outcomes** (*expparams*)

**likelihood** (*outcomes, modelparams, expparams*)

### 3.15.4 NDieModel

**class** qinfer.NDieModel (*n=6, threshold=1e-07*)

Bases: qinfer.abstract\_model.FiniteOutcomeModel

Implements a model of rolling a die with  $n$  sides, whose unknown model parameters are the weights of each side; a generalization of CoinModel. An experiment consists of rolling the die once. The faces of the die are zero indexed, labeled 0,1,2,...,n-1.

**Parameters**

- **n** (*int*) – Number of sides on the die.
- **threshold** (*float*) – How close to 1 the probabilities of the sides of the die must be.

**n\_modelparams**

**expparams\_dtype**

**is\_n\_outcomes\_constant**

Returns `True` if and only if the number of outcomes for each experiment is independent of the experiment being performed.

This property is assumed by inference engines to be constant for the lifetime of a Model instance.

**are\_models\_valid** (*modelparams*)

**n\_outcomes** (*expparams*)

Returns an array of dtype `uint` describing the number of outcomes for each experiment specified by *expparams*.

Parameters **expparams** (*numpy.ndarray*) – Array of experimental parameters. This array must be of dtype agreeing with the `expparams_dtype` property.

**likelihood** (*outcomes, modelparams, expparams*)

## 3.16 Quantum Tomography

### 3.16.1 TomographyBasis

**class** `qinfer.tomography.TomographyBasis` (*data, dims, labels=None, superrep=None, name=None*)

Bases: `object`

A basis of Hermitian operators used for representing tomographic objects (states and channels) as vectors of real elements. By assumption, a tomographic basis is taken to have an initial (0th) element proportional to the identity, and all other elements are taken to be traceless. For example, the Pauli matrices form a tomographic basis for qubits.

Instances of `TomographyBasis` convert between representations of tomographic objects as real vectors of model parameters and QuTiP `Qobj` instances. The latter is convenient for working with other libraries, and for reasoning about fidelities and other metrics, while model parameter representations are useful for defining prior distributions and tomographic models.

#### Parameters

- **data** (*np.ndarray*) – Dense array of shape  $(\text{dim} \times 2, \text{dim}, \text{dim})$  containing all elements of the new tomographic basis. `data[alpha, i, j]` is the  $(i, j)$ -th element of the  $\alpha$ -th matrix of the new basis.
- **dims** (*list*) – Dimensions specification used in converting to QuTiP representations. The product of all elements of `dims` must equal the dimension of axes 1 and 2 of `data`. For instance, `[2, 3]` specifies that the basis is over the tensor product of a qubit and a qutrit space.
- **labels** (*str* or *list* of *str*) – LaTeX-formatted labels for each basis element. If a single *str*, a subscript is added to each basis element's label.
- **superrep** (*str*) – Superoperator representation to pass to QuTiP when reconstructing states.

**data = None**

Dense matrix... TODO: document indices!

**dims = None**

Dimensions of each index, used when converting to QuTiP `Qobj` instances.

**labels = None**

Labels for each basis element.

**dim**

Dimension of the Hilbert space on which elements of this basis act.

Type `int`

**name**

Name to use when converting this basis to a string.

Type `str`

**flat()**

Returns a NumPy array that represents this operator basis in a flattened manner, such that `basis.flat()[i, j]` is the  $j$ th element of the flattened  $i$ th basis operator.

**state\_to\_modelparams** (*state*)

Converts a QuTiP-represented state into a model parameter vector.

**Parameters** *state* (*qutip.Qobj*) – State to be converted.

**Return type** `np.ndarray`

**Returns** The representation of the given state in this basis, as a vector of real parameters.

**modelparams\_to\_state** (*modelparams*)

Converts one or more vectors of model parameters into QuTiP-represented states.

**Parameters** *modelparams* (*np.ndarray*) – Array of shape `(basis.dim ** 2, )` or `(n_states, basis.dim ** 2)` containing states represented as model parameter vectors in this basis.

**Return type** *Qobj* or list of *Qobj* instances.

**Returns** The given states represented as *Qobj* instances.

**covariance\_mtx\_to\_superop** (*mtx*)

Converts a covariance matrix to the corresponding superoperator, represented as a QuTiP *Qobj* with `type="super"`.

## Built-in bases

`qinfer.tomography.gell_mann_basis` (*dim*)

Returns a *TomographyBasis* on *dim* dimensions using the generalized Gell-Mann matrices.

This implementation is based on a MATLAB-language implementation provided by Carlos Riofrío, Seth Merkel and Andrew Silberfarb. Used with permission.

**Parameters** *dim* (*int*) – Dimension of the individual matrices making up the returned basis.

**Return type** *TomographyBasis*

**Returns** A basis of `dim * dim` Gell-Mann matrices.

`qinfer.tomography.pauli_basis` (*nq=1*)

Returns a *TomographyBasis* for the Pauli basis on *nq* qubits.

**Parameters** *nq* (*int*) – Number of qubits on which the returned basis is defined.

`qinfer.tomography.tensor_product_basis` (*\*bases*)

Returns a *TomographyBasis* formed by the tensor product of two or more factor bases. Each basis element is the tensor product of basis elements from the underlying factors.

## 3.16.2 DensityOperatorDistribution

**class** `qinfer.tomography.DensityOperatorDistribution` (*basis*)

Bases: `qinfer.distributions.SingleSampleMixin`, `qinfer.distributions.Distribution`

Distribution over density operators parameterized in a given basis.

**Parameters** *basis* (*int* or *TomographyBasis*) – Basis to use in representing sampled density operators. If an *int*, assumes a default (Gell-Mann) basis of that dimension.

**n\_rvs**

Number of random variables represented by this distribution.

Type `int`**dim**

Dimension of the Hilbert space on which sampled density operators act.

Type `int`**basis**

Basis used to represent sampled density operators as model parameter vectors.

### 3.16.3 Specific Distributions

**class** `qinfer.tomography.TensorProductDistribution` (*factors*)Bases: `qinfer.tomography.distributions.DensityOperatorDistribution`

This class is implemented using QuTiP (v3.1.0 or later), and thus will not work unless QuTiP is installed.

**Parameters** **factors** (list of `DensityOperatorDistribution` instances) – Distributions representing each factor of the tensor product used to generate samples.**class** `qinfer.tomography.GinibreDistribution` (*basis*, *rank=None*)Bases: `qinfer.tomography.distributions.DensityOperatorDistribution`

Distribution over all trace-1 positive semidefinite operators of a given rank. Generalizes the Hilbert-Schmidt (full-rank) and Haar (rank-1) distributions.

**Parameters**

- **basis** (`TomographyBasis`) – Basis to use in generating samples.
- **rank** (`int`) – Rank of each sampled state. If `None`, defaults to full-rank.

**class** `qinfer.tomography.GinibreReditDistribution` (*basis*, *rank=None*)Bases: `qinfer.tomography.distributions.DensityOperatorDistribution`

Distribution over all real-valued trace-1 positive semidefinite operators of a given rank. Generalizes the Hilbert-Schmidt (full-rank) and Haar (rank-1) distributions. Useful for plotting.

**Parameters**

- **basis** (`TomographyBasis`) – Basis to use in generating samples.
- **rank** (`int`) – Rank of each sampled state. If `None`, defaults to full-rank.

**class** `qinfer.tomography.BCSZChoiDistribution` (*basis*, *rank=None*, *enforce\_tp=True*)Bases: `qinfer.tomography.distributions.DensityOperatorDistribution`

Samples Choi states for completely-positive (CP) or CP and trace-preserving (CPTP) maps, as generated by the BCSZ prior [BCSZ09]. The sampled states are normalized as states (trace 1).

**class** `qinfer.tomography.GADFLIDistribution` (*fiducial\_distribution*, *mean*)Bases: `qinfer.tomography.distributions.DensityOperatorDistribution`

Samples operators from the generalized amplitude damping prior for likelihood-based inference [GCC16], given a fiducial distribution and the desired mean for the prior.

**Parameters**

- **fiducial\_distribution** (`DensityOperatorDistribution`) – Distribution from which samples are initially drawn before transformation under generalized amplitude damping.

- **mean** (*qutip.Qobj*) – State which will be the mean of the GAD-transformed samples.

### 3.16.4 Models

**class** `qinfer.tomography.TomographyModel` (*basis*, *allow\_subnormalized=False*)

Bases: `qinfer.abstract_model.FiniteOutcomeModel`

Model for tomographically learning a quantum state using two-outcome positive-operator valued measures (POVMs).

#### Parameters

- **basis** (*TomographyBasis*) – Basis used in representing states as model parameter vectors.
- **allow\_subnormalized** (*bool*) – If `False`, states  $\rho$  are constrained during resampling such that  $\text{Tr}(\rho) = 1$ .

**dim**

Dimension of the Hilbert space on which density operators learned by this model act.

Type `int`

**basis**

Basis used in converting between *Qobj* and model parameter vector representations of states.

Type *TomographyBasis*

**n\_modelparams**

**modelparam\_names**

**is\_n\_outcomes\_constant**

**expparams\_dtype**

**n\_outcomes** (*expparams*)

**are\_models\_valid** (*modelparams*)

**canonicalize** (*modelparams*)

Truncates negative eigenvalues and from each state represented by a tensor of model parameter vectors, and renormalizes as appropriate.

**Parameters** **modelparams** (*np.ndarray*) – Array of shape  $(n\_states, \text{dim} \times 2)$  containing model parameter representations of each of *n\_states* different states.

**Returns** The same model parameter tensor with all states truncated to be positive operators. If *allow\_subnormalized* is `False`, all states are also renormalized to trace one.

**trunc\_neg\_eigs** (*particle*)

Given a state represented as a model parameter vector, returns a model parameter vector representing the same state with any negative eigenvalues set to zero.

**Parameters** **particle** (*np.ndarray*) – Vector of length  $(\text{dim} \times 2, )$  representing a state.

**Returns** The same state with any negative eigenvalues set to zero.

**renormalize** (*modelparams*)

Renormalizes one or more states represented as model parameter vectors, such that each state has trace 1.

**Parameters** **modelparams** (*np.ndarray*) – Array of shape  $(n\_states, \text{dim} \times 2)$  representing one or more states as model parameter vectors.

**Returns** The same state, normalized to trace one.

**likelihood** (*outcomes, modelparams, expparams*)

**class** `qinfer.tomography.DiffusiveTomographyModel` (*basis, allow\_subnormalized=False*)

Bases: `qinfer.tomography.models.TomographyModel`

**n\_modelparams**

**expparams\_dtype**

**modelparam\_names**

**are\_models\_valid** (*modelparams*)

**canonicalize** (*modelparams*)

**likelihood** (*outcomes, modelparams, expparams*)

**update\_timestep** (*modelparams, expparams*)

### 3.16.5 Heuristics

#### Abstract Heuristics

**class** `qinfer.tomography.StateTomographyHeuristic` (*updater, basis=None, other\_fields=None*)

Bases: `qinfer.expdesign.Heuristic`

**class** `qinfer.tomography.ProcessTomographyHeuristic` (*updater, basis, other\_fields=None*)

Bases: `qinfer.expdesign.Heuristic`

**class** `qinfer.tomography.BestOfKMetaheuristic` (*updater, base\_heuristic, k=3, other\_fields=None*)

Bases: `qinfer.expdesign.Heuristic`

Draws  $k$  different state or tomography measurements, then selects the one that has the largest expected value under the action of the covariance superoperator for the current posterior.

#### Specific Heuristics

**class** `qinfer.tomography.RandomStabilizerStateHeuristic` (*updater, basis=None, other\_fields=None*)

Bases: `qinfer.tomography.expdesign.StateTomographyHeuristic`

Randomly chooses rank-1 projectors onto a stabilizer state.

**class** `qinfer.tomography.RandomPauliHeuristic` (*updater, basis=None, other\_fields=None*)

Bases: `qinfer.tomography.expdesign.StateTomographyHeuristic`

Randomly chooses a Pauli measurement. Defined for qubits only.

**class** `qinfer.tomography.ProductHeuristic` (*updater, basis, prep\_heuristic\_class, meas\_heuristic\_class, other\_fields=None*)

Bases: `qinfer.tomography.expdesign.ProcessTomographyHeuristic`

Takes two heuristic classes, one for preparations and one for measurements, then returns a sample from each. The preparation heuristic is assumed to return only trace-1 Hermitian operators.



### 3.16.6 Plotting Functions

`qinfer.tomography.plot_cov_ellipse` (*cov*, *pos*, *nstd*=2, *ax*=None, *\*\*kwargs*)

Plots an *nstd* sigma error ellipse based on the specified covariance matrix (*cov*). Additional keyword arguments are passed on to the ellipse patch artist.

#### Parameters

- **cov** – The 2x2 covariance matrix to base the ellipse on.
- **pos** – The location of the center of the ellipse. Expects a 2-element sequence of [*x*0, *y*0].
- **nstd** – The radius of the ellipse in numbers of standard deviations. Defaults to 2 standard deviations.
- **ax** – The axis that the ellipse will be plotted on. Defaults to the current axis.

**Returns** A matplotlib ellipse artist.

`qinfer.tomography.plot_rebit_prior` (*prior*, *rebit\_axes*=[1, 2], *n\_samples*=2000, *true\_state*=None, *true\_size*=250, *force\_mean*=None, *legend*=True, *mean\_color\_index*=2)

Plots rebit states drawn from a given prior.

#### Parameters

- **prior** (`qinfer.tomography.DensityOperatorDistribution`) – Distribution over rebit states to plot.
- **rebit\_axes** (*list*) – List containing indices for the *x* and *z* axes.
- **n\_samples** (*int*) – Number of samples to draw from the prior.
- **true\_state** (*np.ndarray*) – State to be plotted as a “true” state for comparison.

`qinfer.tomography.plot_rebit_posterior` (*updater*, *prior*=None, *true\_state*=None, *n\_std*=3, *rebit\_axes*=[1, 2], *true\_size*=250, *legend*=True, *level*=0.95, *region\_est\_method*='cov')

Plots posterior distributions over rebits, including covariance ellipsoids

#### Parameters

- **updater** (`qinfer.smc.SMCUpdater`) – Posterior distribution over rebits.
- **qinfer.tomography.DensityOperatorDistribution** – Prior distribution over rebit states.
- **true\_state** (*np.ndarray*) – Model parameters for “true” state to plot as comparison.
- **n\_std** (*float*) – Number of standard deviations out from the mean at which to draw the covariance ellipse. Only used if *region\_est\_method* is ‘cov’.
- **level** (*float*) – Credibility level to use for computing region estimators from convex hulls.
- **rebit\_axes** (*list*) – List containing indices for the *x* and *z* axes.
- **region\_est\_method** (*str*) – Method to use to draw region estimation. Must be one of None, ‘cov’ or ‘hull’.

## 3.17 Utility Functions

### 3.17.1 Function Reference

`qinfer.utils.binomial_pdf(N, n, p)`

Returns the PDF of the binomial distribution  $\text{Bin}(N, p)$  evaluated at  $n$ .

`qinfer.utils.outer_product(vec)`

Returns the outer product of a vector  $v$  with itself,  $vv^T$ .

`qinfer.utils.particle_meanfn(weights, locations, fn=None)`

Returns the mean of a function  $f$  over model parameters.

#### Parameters

- **weights** (*numpy.ndarray*) – Weights of each particle.
- **locations** (*numpy.ndarray*) – Locations of each particle.
- **fn** (*callable*) – Function of model parameters to take the mean of. If `None`, the identity function is assumed.

`qinfer.utils.particle_covariance_mtx(weights, locations)`

Returns an estimate of the covariance of a distribution represented by a given set of SMC particle.

#### Parameters

- **weights** – An array containing the weights of each particle.
- **location** – An array containing the locations of each particle.

**Return type** *numpy.ndarray*, shape (n\_modelparams, n\_modelparams).

**Returns** An array containing the estimated covariance matrix.

`qinfer.utils.in_ellipsoid(x, A, c)`

Determines which of the points  $x$  are in the closed ellipsoid with shape matrix  $A$  centered at  $c$ . For a single point  $x$ , this is computed as

$$(c - x)^T \cdot A^{-1} \cdot (c - x) \leq 1$$

#### Parameters

- **x** (*np.ndarray*) – Shape (n\_points, dim) or n\_points.
- **A** (*np.ndarray*) – Shape (dim, dim), positive definite
- **c** (*np.ndarray*) – Shape (dim)

**Returns** *bool* or array of bools of length n\_points

`qinfer.utils.ellipsoid_volume(A=None, invA=None)`

Returns the volume of an ellipsoid given either its matrix or the inverse of its matrix.

`qinfer.utils.mvee(points, tol=0.001)`

Returns the minimum-volume enclosing ellipse (MVEE) of a set of points, using the Khachiyan algorithm.

`qinfer.utils.uniquify(seq)`

Returns the unique elements of a sequence *seq*.

`qinfer.utils.format_uncertainty(value, uncertainty, scinotn_break=4)`

Given a value and its uncertainty, format as a LaTeX string for pretty-printing.

**Parameters** `scinotn_break` (*int*) – How many decimal points to print before breaking into scientific notation.

## DEVELOPMENT GUIDE

### 4.1 Writing Documentation

The documentation for **QInfer** is written using the [Sphinx documentation engine](#), and is hosted by ReadTheDocs. This allows us to produce high-quality HTML- and LaTeX-formatted reference and tutorial material for **QInfer**. In particular, the documentation [hosted by ReadTheDocs](#) is integrated with the [GitHub project](#) for **QInfer**, simplifying the process of building and deploying documentation.

In this section, we will discuss how to use Sphinx and ReadTheDocs together to contribute to and improve **QInfer** documentation.

#### 4.1.1 Building Documentation With Sphinx

In developing and writing documentation, it is helpful to be able to compile the current version of the documentation offline. To do so, first install Sphinx itself. If you are using Anaconda:

```
$ conda install sphinx
```

Otherwise, we suggest installing Sphinx using [pip](#):

```
$ pip install sphinx
```

In either case, after installing Sphinx, you may need to install additional libraries that used by particular examples in the **QInfer** documentation. On Anaconda:

```
$ conda install scikit-learn ipython future matplotlib  
$ conda install -c conda-forge qutip  
$ pip install mpltools
```

Otherwise:

```
$ pip install -r doc/rtd-requirements.txt
```

With the dependencies installed, you can now build the documentation using the `Makefile` provided by Sphinx, or using the `make.bat` script for Windows. Note that because the documentation includes several computationally-intensive examples, the build process may take a significant amount of time (a few minutes). On Linux and OS X:

```
$ cd doc/  
$ make clean # Deletes all previously compiled outputs.  
$ make html # Builds HTML-formatted docs.  
$ make latexpdf # Builds PDF-formatted docs using LaTeX.
```

All of the compiled outputs will be saved to the `doc/_build` folder. In particular, the HTML version can be found at `doc/_build/html/index.html`.

On Windows, we recommend using PowerShell to run `make.bat`:

```
PS > cd doc/  
PS > .\make.bat clean  
PS > .\make.bat html
```

Note that on Windows, building PDF-formatted docs requires an additional step. First, make the LaTeX-formatted source:

```
PS > .\make latex
```

This will produce a folder called `doc/_build/latex` containing `QInfer.tex`. Build this with your favorite LaTeX front-end to produce the final PDF.

## 4.1.2 Formatting Documentation With reStructuredText

The documentation itself is written in the reStructuredText language, an extensible and (largely) human-readable text format. We recommend reading the [primer](#) provided with Sphinx to get a start. Largely, however, documentation can be written as plain text, with emphasis indicated by `*asterisks*`, strong text indicated by `**double asterisks**`, and verbatim snippets indicated by ``double backticks``. Sections are denoted by different kinds of underlining, using `=`, `-`, `~` and `^` to indicate sections, subsections, paragraphs and subparagraphs, respectively.

Links are a bit more complicated, and take on a couple several different forms:

- Inline links consist of backticks, with addresses denoted in angle-brackets, ``link text <link target>`_`. Note the final `_`, which denotes that the backticks describe a link.
- Alternatively, the link target may be placed later on the page, as in the following snippet:

```
Lorem `ipsum`_ dolor sit amet...  
  
.. _ipsum: http://www.lipsum.com/
```

- Links within the documentation are made using `:ref:`. For example, `:ref:`apiref`` formats as [API Reference](#). The target of such a reference must be declared before a section header, as in the following example, which declares the target `foobar`:

```
.. _foobar:  
  
A Foo About Bar  
-----
```

- Links to Python classes, modules and functions are formatted using `:class:`, `:mod:` and `:func:`, respectively. For example, `:class:`qinfer.SMCUpdater`` formats as [qinfer.SMCUpdater](#). To suppress the path to a Python name, preface the name with a tilde (`~`), as in `:class:`~qinfer.SMCUpdater``. For a Python name to be a valid link target, it must be listed in the [API Reference](#) (see below), or must be documented in one of the external projects listed in `doc/conf.py`. For instance, to link to NumPy documentation, use a link of the form `:class:`~numpy.ndarray``.
- Finally, **QInfer** provides special notation for linking to DOIs, Handles and arXiv postings:

```
:doi:`10.1088/1367-2630/18/3/033024`, :hdl:`10012/9217`,  
:arxiv:`1304.5828`
```

## Typesetting Math

Math is formatted using the Sphinx markup `:math: `...`` in place of `$`, and using the `.. math::` directive in place of `$$`. When building HTML- or PDF-formatted documentation, this is automatically converted to [MathJax](#)-

or LaTeX-formatted math. The **QInfer** documentation is configured with several macros available to each of Math-Jax and LaTeX, specified in `doc/_templates/page.html` and `doc/conf.py`, respectively. For example, `:math: '\expect'` is configured to produce the blackboard-bold expectation operator  $\mathbb{E}$ .

### 4.1.3 Docstrings and API References

One of the most useful features of Sphinx is that it can import documentation from Python code itself. In particular, the `.. autofunction::` and `.. autoclass::` directives import documentation from functions and classes, respectively. These directives typeset the docstrings for their targets as reStructuredText, with the following notation used to indicate arguments, return types, etc.:

- `:param name:` is used to declare that a class' initializer or a function takes an argument named `name`, and is followed by a description of that parameter.
- `:param type name:` can be used to indicate that `name` has the type `type`. If `type` is a recognized Python type, then Sphinx will automatically convert it into a link.
- `:type name:` can be used to provide more detailed information about the type of the parameter `name`, and is followed by a longer description of that parameter's type. `:type:` on its own can be used to denote the type of a property accessor.
- `:return:` is used to describe what a function returns.
- `:rtype:` is used to describe the type of a return value.
- `:raises exc_type:` denotes that the described function raises an exception of type `exc_type`, and describes the conditions under which that exception is raised.

In addition to the standard Sphinx fields described above, **QInfer** adds the following fields:

- `:modelparam name:` describes a model parameter named `name`, where the name is formatted as math (or should be, pending bugs in the documentation configuration).
- `:expparam field_type field_name:` describes an experiment parameter field named `field_name` with `dtype` `field_type`.
- `:scalar-expparam scalar_type` describes that a class has exactly one experiment parameter of type `scalar_type`.
- `:column dtype name:` describes a column for data taken by *Simple Estimation Functions* functions.

Importantly, if math is included in a docstring, it is highly recommended to format the docstring as a *raw string*; that is, as a string starting with `r'` or `r"` for inline strings or `r'''` or `r"""` for multi-line strings. This avoids having to escape TeX markup that appears within a docstring. For instance, consider the following hypothetical function:

```
def state(theta, phi):
    r"""
    Returns an array representing :math:\cos(\theta) \ket{0} +
    \sin(\theta) e^{i \phi} \ket{1}.
    """
    ...
```

If the docstring were instead declared using `"""`, then `\t` everywhere inside the docstring would be interpreted by Python as a tab character, and not as the start of a LaTeX command.

### 4.1.4 Showing Code Snippets

The documentation would be useless without code snippets, so Sphinx provides several ways to show snippets. Perhaps the most common is *doctest-style*:

```
Lorem ipsum dolor sit amet...
```

```
>>> print("Hello, world!")
Hello, world!
```

As described in `_doctest_devguide`, these snippets are run automatically as *tests* to ensure that the documentation and code are both correct. To mark a particular line in a snippet as not testable, add `# doctest: +SKIP` as a comment after.

For longer snippets, or for snippets that should not be run as tests, use the `.. code:: python` directive:

```
.. code:: python

    print("Hello, world!")
```

This formats as:

```
print("Hello, world!")
```

Finally, a block can be formatted as code without any syntax highlighting by using the `::` notation on the previous line, and then indenting the block itself:

```
This is in fact how this section denotes reStructuredText code samples::

    :foobar: is not a valid reStructuredText role.
```

## 4.1.5 Plotting Support

Sphinx can also run Python code and plot the resulting figures. To do so, use the `.. plot::` directive. Note that any such plots should be relatively quick to generate, especially so as to not overburden the build servers provided by ReadTheDocs. The `.. plot::` directive has been configured to automatically import **QInfer** itself and to import `matplotlib` as `plt`. Thus, for example, the following demonstrates plotting functionality provided by the `qinfer.tomography` module:

```
.. plot::

    basis = tomography.bases.pauli_basis(1)
    prior = tomography.distributions.GinibreDistribution(basis)
    tomography.plot_rebit_prior(prior, rebit_axes=[1, 3])
    plt.show()
```

Note the `plt.show()` call at the end; this is *required* to produce the final figure!

## 4.2 Unit and Documentation Testing

### 4.2.1 Unit Tests

### 4.2.2 Documentation Tests

As described in *Showing Code Snippets*, Sphinx integrates with Python's `doctest` module to help ensure that both the documentation and underlying library are correct. Doctests consist of short snippets of code along with their expected output. A doctest *passes* if the actual output of the snippet matches its expected output. For instance, a doctest that `1 + 1` correctly produces `2` could be written as:

Below, we show an example of addition `in` practice:

```
>>> 1 + 1
2
```

Later, we will consider more advanced operators.

The blank lines above and below the doctest separate it from the surrounding text, while the expected output appears immediately below the relevant code.

To run the doctests in the **QInfer** documentation using Linux or OS X:

```
$ cd doc/
$ make doctest
```

To run the doctests on Windows using PowerShell, use `.\make` instead:

```
PS > cd doc/
PS > .\make doctest
```

As with the unit tests, doctests are automatically run on pull requests, to help ensure the correctness of contributed documentation.

## Test Annotations

A doctest snippet may be annotated with one or more comments that change the behavior of that test. The `doctest` documentation goes into far more detail, but the two we will commonly need are `# doctest: +SKIP` and `# doctest: +ELLIPSIS`. The former causes a test to be skipped entirely. Skipping tests can be useful if the output of a doctest is random, for instance.

The second, `+ELLIPSIS`, causes any ellipsis (`...`) in the expected output to act as a wild card. For instance, both of the following doctests would pass:

```
>>> print([1, 2, 3])
[1, ..., 3]
>>> print([1, 2, 3, 4, 'foo', 3])
[1, ..., 3]
```

## Doctest Annoyances

There are a few annoyances that come along with writing tests based on string-equivalence of outputs, in particular for a cross-platform and 2/3 compatible library. In particular:

- NumPy, 2to3 and `type/class`: Python 2 and 3 differ on whether the type of NumPy `ndarray` prints as `type` (Python 2) `class` (Python 3):

```
>>> print(type(np.array([1])))
<type 'numpy.ndarray'> # Python 2
<class 'numpy.ndarray'> # Python 3
```

Thus, to write a doctest that checks if something is a NumPy array or not, it is preferred to use an `isinstance` check instead:

```
>>> isinstance(np.array([1]), np.ndarray)
True
```

Though this sacrifices some on readability, it gains on portability and correctness.



- `int` versus `long` in array shapes: The Windows and Linux versions of NumPy behave differently with respect to when a NumPy shape is represented as a `tuple` of `int` versus a `tuple` of `long` values. This can cause doctests to choke on spurious `L` suffixes:

```
>>> print(np.zeros((1, 10)).shape)
(1, 10) # tuple of int
(1L, 10L) # tuple of long
```

Since `int` and `long` respect `==`, however, the same trick as above can help:

```
>>> np.zeros((1, 10)).shape == (1, 10)
True
```

## ACKNOWLEDGEMENTS

We gratefully acknowledge contributions and testing to the **QInfer** project by the following individuals:

- Thomas Alexander
- Steven Casagrande
- Jonathan Gross
- Ian Hincks
- Michal Kononenko
- Yuval Sanders

Additionally, we thank those that have helped us to test **QInfer**, and that have made useful suggestions, pushing us forward.

- Joshua Combes
- Rahul Deshpande
- Nathan Wiebe



- [BCSZ09] Bruzda, W., Cappellini, V., Sommers, H-J. & Życzkowski, K. Random quantum operations. *Physics Letters A*. **373** 3 320–324 (2009). doi:10.1016/j.physleta.2008.11.043.
- [FB12] Ferrie C., Blume-Kohout R. Estimating the bias of a noisy coin. *AIP Conf. Proc.* 1443, 14-21 (2012). doi:10.1063/1.3703615. arXiv:1201.1493.
- [FGC12] Ferrie C., Granade C. E. & Cory D. G. How to best sample a periodic probability distribution, or on the accuracy of Hamiltonian finding strategies. *Quantum Information Processing* (2012). doi:10.1007/s11128-012-0407-6. arXiv:1110.3067.
- [FG13] Ferrie C., Granade C. E. Likelihood-free parameter estimation. arXiv:1304.5828
- [Fer14] Ferrie C. High posterior density ellipsoids of quantum states. *New Journal of Physics*. **16** 023006 (2014). doi:10.1088/1367-2630/16/2/023006. arXiv:1310.1903.
- [GFWC12] Granade C. E., Ferrie C., Wiebe N. & Cory D. G. Robust online Hamiltonian learning. *New Journal of Physics* **14** 103013 (2012). doi:10.1088/1367-2630/14/10/103013. arXiv:1207.1655.
- [GFC14] Granade C. E., Ferrie C. & Cory D. G. Accelerated randomized benchmarking. arXiv:1404.5275.
- [Gra15] Granade C. E. Characterization, verification and control for large quantum systems. PhD thesis. hdl:10012/9217.
- [JDD08] Johansen A. M., Doucet A. & Davy M. Particle methods for maximum likelihood estimation in latent variable models. doi:10.1007/s11222-007-9037-8.
- [KL+08] Knill E., Leibfried D., Reichle R., Britton J., Blakestad R. B., Jost J. D., Langer C., Ozeri R., Seidelin S., and Wineland D. J. Randomized benchmarking of quantum gates. *Physical Review A*. **77** 1, 012307 (2008). doi:10.1103/PhysRevA.77.012307.
- [LW01] Liu J. and West M. Combined parameter and state estimation in simulation-based filtering. *Sequential Monte Carlo Methods in Practice* (2001).
- [Mez06] Mezzadri F. How to generate random matrices from the classical compact groups. (2006). arXiv:math-ph/0609050v2.
- [MGE12] Magesan E., Gambetta J. M., & Emerson J. Characterizing quantum gates via randomized benchmarking. *Physical Review A*. **85** 042311 (2012). doi:10.1103/PhysRevA.85.042311. arXiv:1109.6887.
- [Mis12] Miszczak J. Generating and using truly random quantum states in Mathematica. *Computer Physics Communications* **183** 118-124 (2012). doi:10.1016/j.cpc.2011.08.002.
- [SSK14] Stenberg M., Sanders Y. R., Wilhelm F. Efficient estimation of resonant coupling between quantum systems. arXiv:1407.5631
- [WGFC13a] Wiebe N., Granade C. E., Ferrie C. & Cory D. G. Hamiltonian Learning and Certification Using Quantum Resources. arXiv:1309.0876

- [WGFC13b] Wiebe N., Granade C. E., Ferrie C. & Cory D. G. Quantum Hamiltonian Learning Using Imperfect Quantum Resources. [arXiv:1311.5269](#)
- [GCC16] Granade C. E., Combes J. & Cory D. G. Practical Bayesian Tomography. [doi:10.1088/1367-2630/18/3/033024](#)
- [OSZ10] Osipov V. A., Sommers H.-J., Zyczkowski K., Random Bures mixed states and the distribution of their purity, [doi:10.1088/1751-8113/43/5/055302](#)

## A

AcceleratedPrecessionModel (class in qinfer), 55  
 allow\_identical\_outcomes (qinfer.Model attribute), 39  
 are\_expparam\_dtypes\_consistent() (qinfer.BinomialModel method), 42  
 are\_expparam\_dtypes\_consistent() (qinfer.MultinomialModel method), 43  
 are\_expparam\_dtypes\_consistent() (qinfer.Simulatable method), 36  
 are\_models\_valid() (qinfer.AcceleratedPrecessionModel static method), 55  
 are\_models\_valid() (qinfer.NDieModel method), 72  
 are\_models\_valid() (qinfer.NoisyCoinModel static method), 72  
 are\_models\_valid() (qinfer.RandomizedBenchmarkingModel method), 61  
 are\_models\_valid() (qinfer.Simulatable method), 36  
 are\_models\_valid() (qinfer.tomography.DiffusiveTomographyModel method), 77  
 are\_models\_valid() (qinfer.tomography.TomographyModel method), 76

## B

base\_model (qinfer.Simulatable attribute), 36  
 basis (qinfer.tomography.DensityOperatorDistribution attribute), 75  
 basis (qinfer.tomography.TomographyModel attribute), 76  
 batch\_update() (qinfer.SMCUpdater method), 66  
 bayes\_risk() (qinfer.SMCUpdater method), 67  
 BCSZChoiDistribution (class in qinfer.tomography), 75  
 BestOfKMetaheuristic (class in qinfer.tomography), 77  
 BetaBinomialDistribution (class in qinfer), 46  
 BetaDistribution (class in qinfer), 45  
 binomial\_pdf() (in module qinfer.utils), 79  
 BinomialModel (class in qinfer), 41

## C

call\_count (qinfer.Model attribute), 38  
 canonicalize() (qinfer.Simulatable method), 38  
 canonicalize() (qinfer.tomography.DiffusiveTomographyModel method), 77  
 canonicalize() (qinfer.tomography.TomographyModel method), 76  
 clear\_cache() (qinfer.DirectViewParallelizedModel method), 57  
 clear\_cache() (qinfer.Simulatable method), 37  
 ConstantDistribution (class in qinfer), 45  
 covariance\_mtx\_to\_superop() (qinfer.tomography.TomographyBasis method), 74

## D

data (qinfer.tomography.TomographyBasis attribute), 73  
 data\_record (qinfer.SMCUpdater attribute), 65  
 decorated\_model (qinfer.BinomialModel attribute), 42  
 decorated\_model (qinfer.MultinomialModel attribute), 43  
 DensityOperatorDistribution (class in qinfer.tomography), 74  
 description (qinfer.IPythonProgressBar attribute), 56  
 design\_expparams\_field() (qinfer.ExperimentDesigner method), 53  
 DifferentiableModel (class in qinfer), 40  
 DiffusiveTomographyModel (class in qinfer.tomography), 77  
 dim (qinfer.tomography.DensityOperatorDistribution attribute), 75  
 dim (qinfer.tomography.TomographyBasis attribute), 73  
 dim (qinfer.tomography.TomographyModel attribute), 76  
 dims (qinfer.tomography.TomographyBasis attribute), 73  
 DirectViewParallelizedModel (class in qinfer), 57  
 distance() (qinfer.Simulatable method), 37  
 Distribution (class in qinfer), 44  
 Domain (class in qinfer), 48  
 domain() (qinfer.BinomialModel method), 42  
 domain() (qinfer.FiniteOutcomeModel method), 40  
 domain() (qinfer.MultinomialModel method), 43  
 domain() (qinfer.Simulatable method), 36  
 dtype (qinfer.Domain attribute), 49

dtype (qinfer.IntegerDomain attribute), 51  
 dtype (qinfer.MultinomialDomain attribute), 52  
 dtype (qinfer.RealDomain attribute), 50

## E

ellipsoid\_volume() (in module qinfer.utils), 79  
 est\_cluster\_covs() (qinfer.SMCUpdater method), 67  
 est\_cluster\_metric() (qinfer.SMCUpdater method), 67  
 est\_cluster\_moments() (qinfer.SMCUpdater method), 67  
 est\_covariance\_mtx() (qinfer.SMCUpdater method), 67  
 est\_credible\_region() (qinfer.SMCUpdater method), 67  
 est\_entropy() (qinfer.SMCUpdater method), 67  
 est\_kl\_divergence() (qinfer.SMCUpdater method), 67  
 est\_mean() (qinfer.SMCUpdater method), 66  
 est\_meanfn() (qinfer.SMCUpdater method), 66  
 example\_point (qinfer.Domain attribute), 49  
 example\_point (qinfer.IntegerDomain attribute), 51  
 example\_point (qinfer.MultinomialDomain attribute), 52  
 example\_point (qinfer.RealDomain attribute), 50  
 expected\_information\_gain() (qinfer.SMCUpdater method), 67  
 experiment\_cost() (qinfer.Simulatable method), 37  
 ExperimentDesigner (class in qinfer), 53  
 expparams\_dtype (qinfer.AcceleratedPrecessionModel attribute), 55  
 expparams\_dtype (qinfer.BinomialModel attribute), 42  
 expparams\_dtype (qinfer.MultinomialModel attribute), 43  
 expparams\_dtype (qinfer.NDieModel attribute), 72  
 expparams\_dtype (qinfer.NoisyCoinModel attribute), 72  
 expparams\_dtype (qinfer.RandomizedBenchmarkingModel attribute), 61  
 expparams\_dtype (qinfer.SimplePrecessionModel attribute), 71  
 expparams\_dtype (qinfer.Simulatable attribute), 35  
 expparams\_dtype (qinfer.tomography.DiffusiveTomographyModel attribute), 77  
 expparams\_dtype (qinfer.tomography.TomographyModel attribute), 76  
 ExpSparseHeuristic (class in qinfer), 54

## F

F() (in module qinfer.rb), 61  
 finished() (qinfer.IPythonProgressBar method), 56  
 FiniteOutcomeModel (class in qinfer), 39  
 fisher\_information() (qinfer.DifferentiableModel method), 40  
 flat() (qinfer.tomography.TomographyBasis method), 73  
 format\_uncertainty() (in module qinfer.utils), 79  
 from\_regular\_array() (qinfer.MultinomialDomain method), 52

## G

GADFLIDistribution (class in qinfer.tomography), 75

GammaDistribution (class in qinfer), 46  
 gell\_mann\_basis() (in module qinfer.tomography), 74  
 GinibreDistribution (class in qinfer.tomography), 75  
 GinibreReditDistribution (class in qinfer.tomography), 75  
 GinibreUniform (class in qinfer), 47  
 grad\_log\_pdf() (qinfer.MultivariateNormalDistribution method), 45  
 grad\_log\_pdf() (qinfer.NormalDistribution method), 44  
 grad\_log\_pdf() (qinfer.PostselectedDistribution method), 47  
 grad\_log\_pdf() (qinfer.UniformDistribution method), 44

## H

h (qinfer.ScoreMixin attribute), 56  
 HaarUniform (class in qinfer), 46  
 Heuristic (class in qinfer), 54  
 HilbertSchmidtUniform (class in qinfer), 46  
 hypothetical\_update() (qinfer.SMCUpdater method), 65

## I

in\_credible\_region() (qinfer.SMCUpdater method), 68  
 in\_domain() (qinfer.Domain method), 49  
 in\_domain() (qinfer.IntegerDomain method), 51  
 in\_domain() (qinfer.MultinomialDomain method), 52  
 in\_domain() (qinfer.RealDomain method), 50  
 in\_ellipsoid() (in module qinfer.utils), 79  
 IntegerDomain (class in qinfer), 50  
 IPythonProgressBar (class in qinfer), 56  
 is\_continuous (qinfer.Domain attribute), 48  
 is\_continuous (qinfer.IntegerDomain attribute), 51  
 is\_continuous (qinfer.MultinomialDomain attribute), 52  
 is\_continuous (qinfer.RealDomain attribute), 50  
 is\_discrete (qinfer.Domain attribute), 49  
 is\_finite (qinfer.Domain attribute), 49  
 is\_finite (qinfer.IntegerDomain attribute), 51  
 is\_finite (qinfer.MultinomialDomain attribute), 52  
 is\_finite (qinfer.RealDomain attribute), 50  
 is\_model\_valid() (qinfer.Model method), 39  
 is\_n\_outcomes\_constant (qinfer.AcceleratedPrecessionModel attribute), 55  
 is\_n\_outcomes\_constant (qinfer.BinomialModel attribute), 42  
 is\_n\_outcomes\_constant (qinfer.MultinomialModel attribute), 43  
 is\_n\_outcomes\_constant (qinfer.NDieModel attribute), 72  
 is\_n\_outcomes\_constant (qinfer.NoisyCoinModel attribute), 72  
 is\_n\_outcomes\_constant (qinfer.RandomizedBenchmarkingModel attribute), 61  
 is\_n\_outcomes\_constant (qinfer.Simulatable attribute), 35

- is\_n\_outcomes\_constant (qinfer.tomography.TomographyModel attribute), 76
- ## J
- just\_resampled (qinfer.SMCUpdater attribute), 64

## L

labels (qinfer.tomography.TomographyBasis attribute), 73

likelihood() (qinfer.AcceleratedPrecessionModel method), 55

likelihood() (qinfer.BinomialModel method), 42

likelihood() (qinfer.DirectViewParallelizedModel method), 57

likelihood() (qinfer.MLEModel method), 44

likelihood() (qinfer.Model method), 38

likelihood() (qinfer.MultinomialModel method), 43

likelihood() (qinfer.NDieModel method), 73

likelihood() (qinfer.NoisyCoinModel method), 72

likelihood() (qinfer.PoisonedModel method), 41

likelihood() (qinfer.RandomizedBenchmarkingModel method), 61

likelihood() (qinfer.SimplePrecessionModel method), 71

likelihood() (qinfer.tomography.DiffusiveTomographyModel method), 77

likelihood() (qinfer.tomography.TomographyModel method), 77

LiuWestResampler (class in qinfer), 61

log\_total\_likelihood (qinfer.SMCUpdater attribute), 65

LogNormalDistribution (class in qinfer), 45

## M

make\_Paulis() (qinfer.HilbertSchmidtUniform method), 46

max (qinfer.IntegerDomain attribute), 51

max (qinfer.RealDomain attribute), 49

min (qinfer.IntegerDomain attribute), 51

min (qinfer.RealDomain attribute), 49

min\_n\_ess (qinfer.SMCUpdater attribute), 65

MixtureDistribution (class in qinfer), 47

MLEModel (class in qinfer), 43

Model (class in qinfer), 38

model\_chain (qinfer.Simulatable attribute), 35

modelparam\_names (qinfer.RandomizedBenchmarkingModel attribute), 61

modelparam\_names (qinfer.Simulatable attribute), 36

modelparam\_names (qinfer.tomography.DiffusiveTomographyModel attribute), 77

modelparam\_names (qinfer.tomography.TomographyModel attribute), 76

modelparams\_to\_state() (qinfer.tomography.TomographyBasis method), 74

MultinomialDomain (class in qinfer), 51

MultinomialModel (class in qinfer), 42

MultivariateNormalDistribution (class in qinfer), 44

mvee() (in module qinfer.utils), 79

## N

n\_dist (qinfer.MixtureDistribution attribute), 48

n\_elements (qinfer.MultinomialDomain attribute), 52

n\_engines (qinfer.DirectViewParallelizedModel attribute), 57

n\_ess (qinfer.SMCUpdater attribute), 65

n\_meas (qinfer.MultinomialDomain attribute), 52

n\_members (qinfer.Domain attribute), 49

n\_members (qinfer.IntegerDomain attribute), 51

n\_members (qinfer.MultinomialDomain attribute), 52

n\_members (qinfer.RealDomain attribute), 50

n\_modelparams (qinfer.AcceleratedPrecessionModel attribute), 55

n\_modelparams (qinfer.NDieModel attribute), 72

n\_modelparams (qinfer.NoisyCoinModel attribute), 72

n\_modelparams (qinfer.RandomizedBenchmarkingModel attribute), 61

n\_modelparams (qinfer.Simulatable attribute), 35

n\_modelparams (qinfer.tomography.DiffusiveTomographyModel attribute), 77

n\_modelparams (qinfer.tomography.TomographyModel attribute), 76

n\_outcomes() (qinfer.AcceleratedPrecessionModel method), 55

n\_outcomes() (qinfer.BinomialModel method), 42

n\_outcomes() (qinfer.MultinomialModel method), 43

n\_outcomes() (qinfer.NDieModel method), 72

n\_outcomes() (qinfer.NoisyCoinModel method), 72

n\_outcomes() (qinfer.RandomizedBenchmarkingModel method), 61

n\_outcomes() (qinfer.Simulatable method), 36

n\_outcomes() (qinfer.tomography.TomographyModel method), 76

n\_outcomes\_cutoff (qinfer.FiniteOutcomeModel attribute), 40

n\_particles (qinfer.SMCUpdater attribute), 64

n\_rvs (qinfer.BetaBinomialDistribution attribute), 46

n\_rvs (qinfer.BetaDistribution attribute), 46

n\_rvs (qinfer.ConstantDistribution attribute), 45

n\_rvs (qinfer.Distribution attribute), 44

n\_rvs (qinfer.GammaDistribution attribute), 46

n\_rvs (qinfer.GinibreUniform attribute), 47

n\_rvs (qinfer.HaarUniform attribute), 47

n\_rvs (qinfer.HilbertSchmidtUniform attribute), 46

n\_rvs (qinfer.LogNormalDistribution attribute), 45

n\_rvs (qinfer.MixtureDistribution attribute), 48



n\_rvs (qinfer.MultivariateNormalDistribution attribute), 45  
n\_rvs (qinfer.NormalDistribution attribute), 44  
n\_rvs (qinfer.PostselectedDistribution attribute), 47  
n\_rvs (qinfer.ProductDistribution attribute), 47  
n\_rvs (qinfer.SlantedNormalDistribution attribute), 45  
n\_rvs (qinfer.SMCUpdater attribute), 66  
n\_rvs (qinfer.tomography.DensityOperatorDistribution attribute), 74  
n\_rvs (qinfer.UniformDistribution attribute), 44  
n\_sides (qinfer.MultinomialModel attribute), 43  
name (qinfer.tomography.TomographyBasis attribute), 73  
NDieModel (class in qinfer), 72  
new\_exp() (qinfer.ExperimentDesigner method), 53  
NoisyCoinModel (class in qinfer), 72  
NormalDistribution (class in qinfer), 44  
normalization\_record (qinfer.SMCUpdater attribute), 64

## O

outcome\_warning\_threshold (qinfer.Model attribute), 39  
outer\_product() (in module qinfer.utils), 79

## P

p() (in module qinfer.rb), 61  
particle\_covariance\_mtx() (in module qinfer.utils), 79  
particle\_meanfn() (in module qinfer.utils), 79  
pauli\_basis() (in module qinfer.tomography), 74  
perf\_test() (in module qinfer), 58  
perf\_test\_multiple() (in module qinfer), 58  
PGH (class in qinfer), 54  
plot\_cov\_ellipse() (in module qinfer.tomography), 78  
plot\_covariance() (qinfer.SMCUpdater method), 70  
plot\_posterior\_contour() (qinfer.SMCUpdater method), 71  
plot\_posterior\_marginal() (qinfer.SMCUpdater method), 70  
plot\_rebit\_posterior() (in module qinfer.tomography), 78  
plot\_rebit\_prior() (in module qinfer.tomography), 78  
PoisonedModel (class in qinfer), 41  
posterior\_marginal() (qinfer.SMCUpdater method), 69  
posterior\_mesh() (qinfer.SMCUpdater method), 70  
PostselectedDistribution (class in qinfer), 47  
pr0\_to\_likelihood\_array() (qinfer.FiniteOutcomeModel static method), 40  
ProcessTomographyHeuristic (class in qinfer.tomography), 77  
ProductDistribution (class in qinfer), 47  
ProductHeuristic (class in qinfer.tomography), 77

## Q

Q (qinfer.Simulatable attribute), 36  
qinfer (module), 1

## R

RandomizedBenchmarkingModel (class in qinfer), 60  
RandomPauliHeuristic (class in qinfer.tomography), 77  
RandomStabilizerStateHeuristic (class in qinfer.tomography), 77  
RealDomain (class in qinfer), 49  
region\_est\_ellipsoid() (qinfer.SMCUpdater method), 68  
region\_est\_hull() (qinfer.SMCUpdater method), 68  
renormalize() (qinfer.tomography.TomographyModel method), 76  
resample() (qinfer.SMCUpdater method), 66  
resample\_count (qinfer.SMCUpdater attribute), 64  
resampling\_divergences (qinfer.SMCUpdater attribute), 65  
reset() (qinfer.SMCUpdater method), 65  
risk() (qinfer.SMCUpdater method), 69

## S

sample() (qinfer.BetaBinomialDistribution method), 46  
sample() (qinfer.BetaDistribution method), 46  
sample() (qinfer.ConstantDistribution method), 45  
sample() (qinfer.Distribution method), 44  
sample() (qinfer.GammaDistribution method), 46  
sample() (qinfer.GinibreUniform method), 47  
sample() (qinfer.HaarUniform method), 47  
sample() (qinfer.HilbertSchmidtUniform method), 46  
sample() (qinfer.LogNormalDistribution method), 45  
sample() (qinfer.MixtureDistribution method), 48  
sample() (qinfer.MultivariateNormalDistribution method), 45  
sample() (qinfer.NormalDistribution method), 44  
sample() (qinfer.PostselectedDistribution method), 47  
sample() (qinfer.ProductDistribution method), 47  
sample() (qinfer.SingleSampleMixin method), 48  
sample() (qinfer.SlantedNormalDistribution method), 45  
sample() (qinfer.SMCUpdater method), 66  
sample() (qinfer.UniformDistribution method), 44  
score() (qinfer.DifferentiableModel method), 40  
score() (qinfer.RandomizedBenchmarkingModel method), 61  
score() (qinfer.ScoreMixin method), 56  
score() (qinfer.SimplePrecessionModel method), 71  
ScoreMixin (class in qinfer), 56  
sim\_count (qinfer.Simulatable attribute), 36  
simple\_est\_prec() (in module qinfer), 62  
simple\_est\_rb() (in module qinfer), 62  
SimplePrecessionModel (class in qinfer), 71  
Simulatable (class in qinfer), 35  
simulate\_experiment() (qinfer.BinomialModel method), 42  
simulate\_experiment() (qinfer.FiniteOutcomeModel method), 40  
simulate\_experiment() (qinfer.MLEModel method), 43

[simulate\\_experiment\(\)](#) ([qinfer.MultinomialModel](#) method), [43](#)  
[simulate\\_experiment\(\)](#) ([qinfer.PoisonedModel](#) method), [41](#)  
[simulate\\_experiment\(\)](#) ([qinfer.Simulatable](#) method), [37](#)  
[SingleSampleMixin](#) (class in [qinfer](#)), [48](#)  
[SlantedNormalDistribution](#) (class in [qinfer](#)), [45](#)  
[SMCUpdater](#) (class in [qinfer](#)), [64](#)  
[start\(\)](#) ([qinfer.IPythonProgressBar](#) method), [56](#)  
[state\\_to\\_modelparams\(\)](#) ([qinfer.tomography.TomographyBasis](#) method), [74](#)  
[StateTomographyHeuristic](#) (class in [qinfer.tomography](#)), [77](#)

## T

[tensor\\_product\\_basis\(\)](#) (in module [qinfer.tomography](#)), [74](#)  
[TensorProductDistribution](#) (class in [qinfer.tomography](#)), [75](#)  
[to\\_regular\\_array\(\)](#) ([qinfer.MultinomialDomain](#) method), [52](#)  
[TomographyBasis](#) (class in [qinfer.tomography](#)), [73](#)  
[TomographyModel](#) (class in [qinfer.tomography](#)), [76](#)  
[trunc\\_neg\\_eigs\(\)](#) ([qinfer.tomography.TomographyModel](#) method), [76](#)

## U

[underlying\\_domain](#) ([qinfer.MultinomialModel](#) attribute), [43](#)  
[underlying\\_model](#) ([qinfer.Simulatable](#) attribute), [36](#)  
[UniformDistribution](#) (class in [qinfer](#)), [44](#)  
[uniquify\(\)](#) (in module [qinfer.utils](#)), [79](#)  
[update\(\)](#) ([qinfer.IPythonProgressBar](#) method), [56](#)  
[update\(\)](#) ([qinfer.SMCUpdater](#) method), [66](#)  
[update\\_timestep\(\)](#) ([qinfer.BinomialModel](#) method), [42](#)  
[update\\_timestep\(\)](#) ([qinfer.Simulatable](#) method), [37](#)  
[update\\_timestep\(\)](#) ([qinfer.tomography.DiffusiveTomographyModel](#) method), [77](#)

## V

[values](#) ([qinfer.Domain](#) attribute), [49](#)  
[values](#) ([qinfer.IntegerDomain](#) attribute), [51](#)  
[values](#) ([qinfer.MultinomialDomain](#) attribute), [52](#)  
[values](#) ([qinfer.RealDomain](#) attribute), [50](#)
